# Supplementary material for: Online storage ring optimization using dimension-reduction and genetic algorithms
Source: arXiv:1807.10720 ancillary file (2019-04-04)

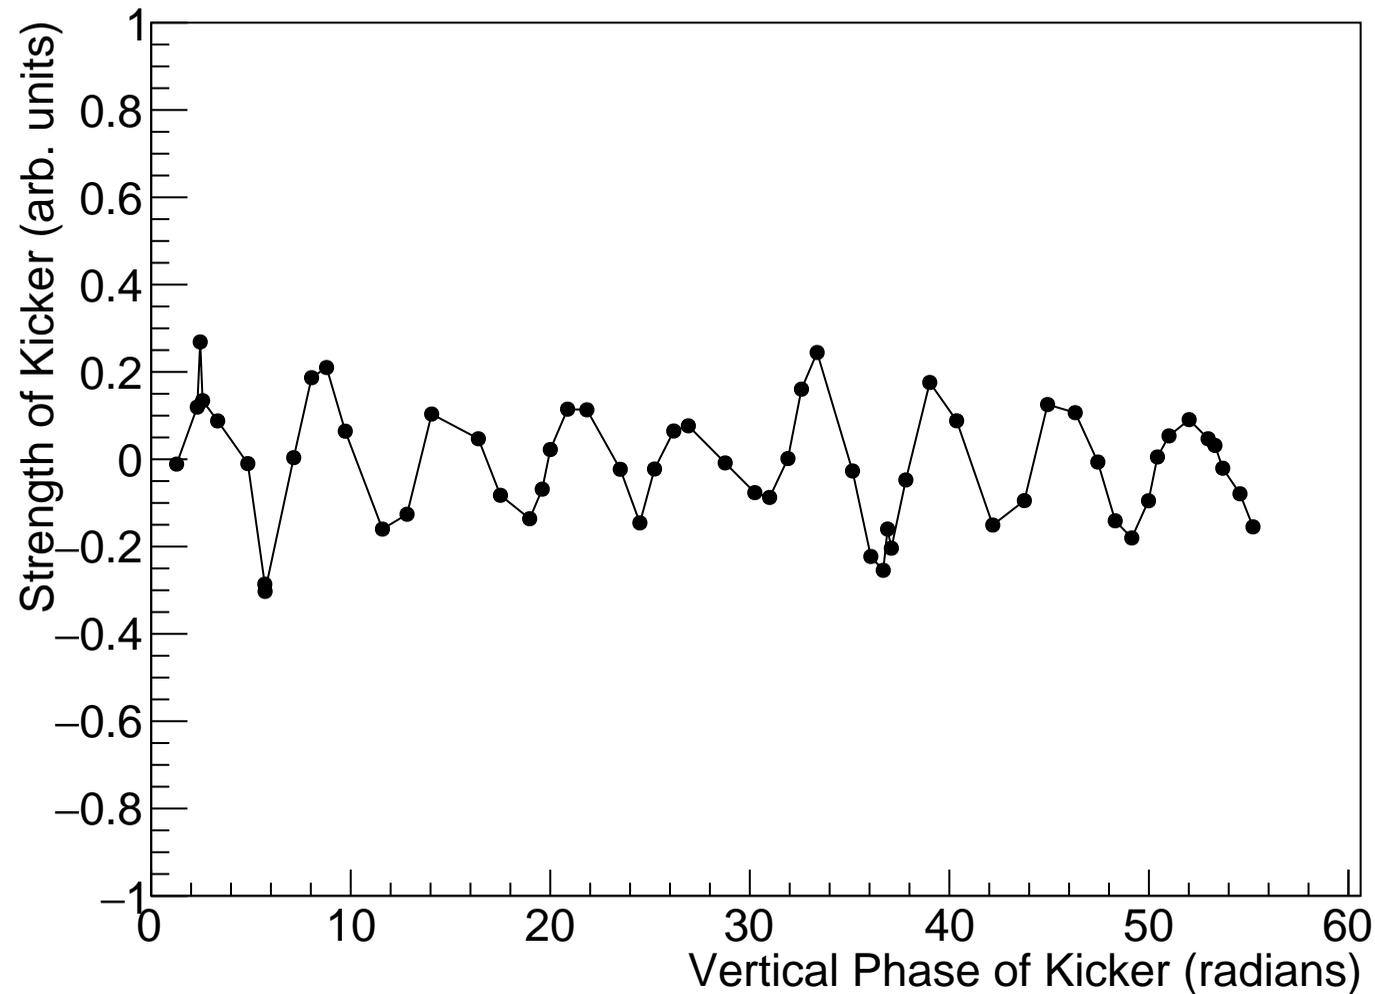

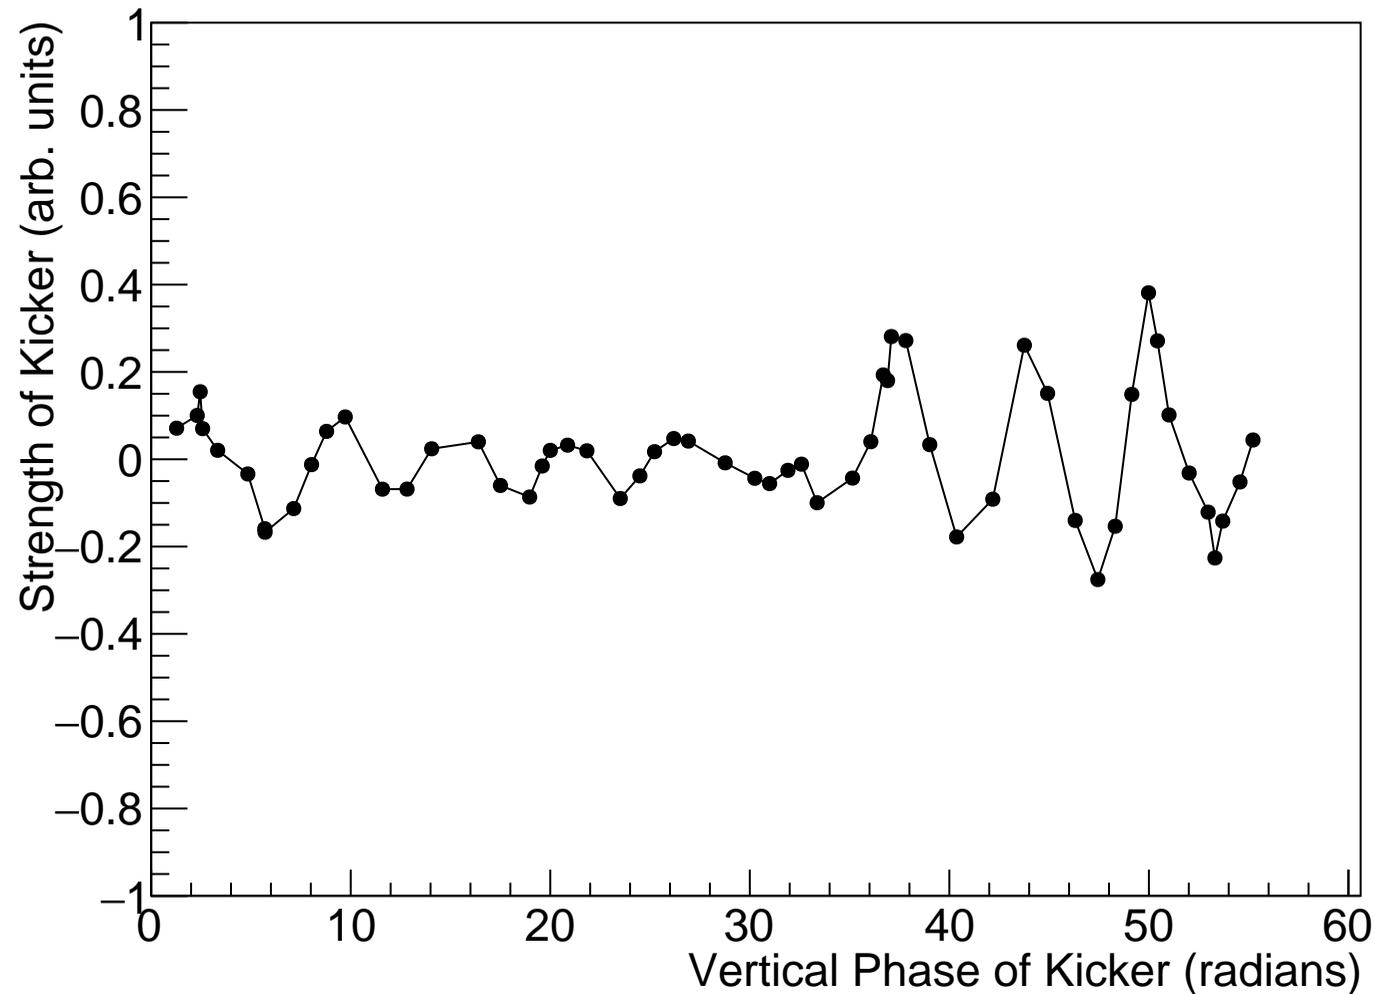

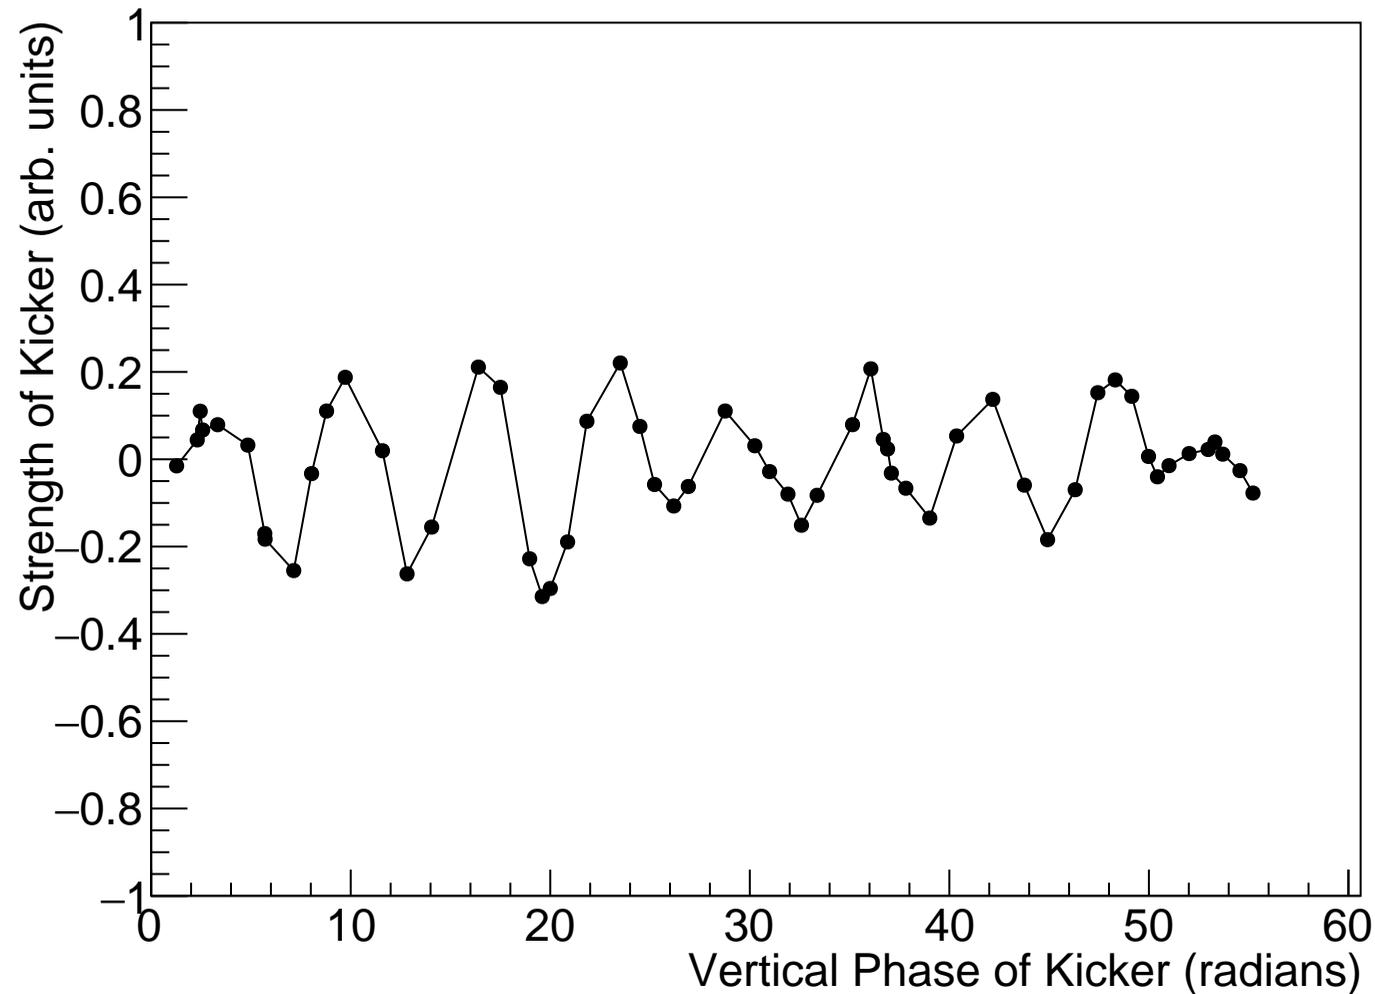

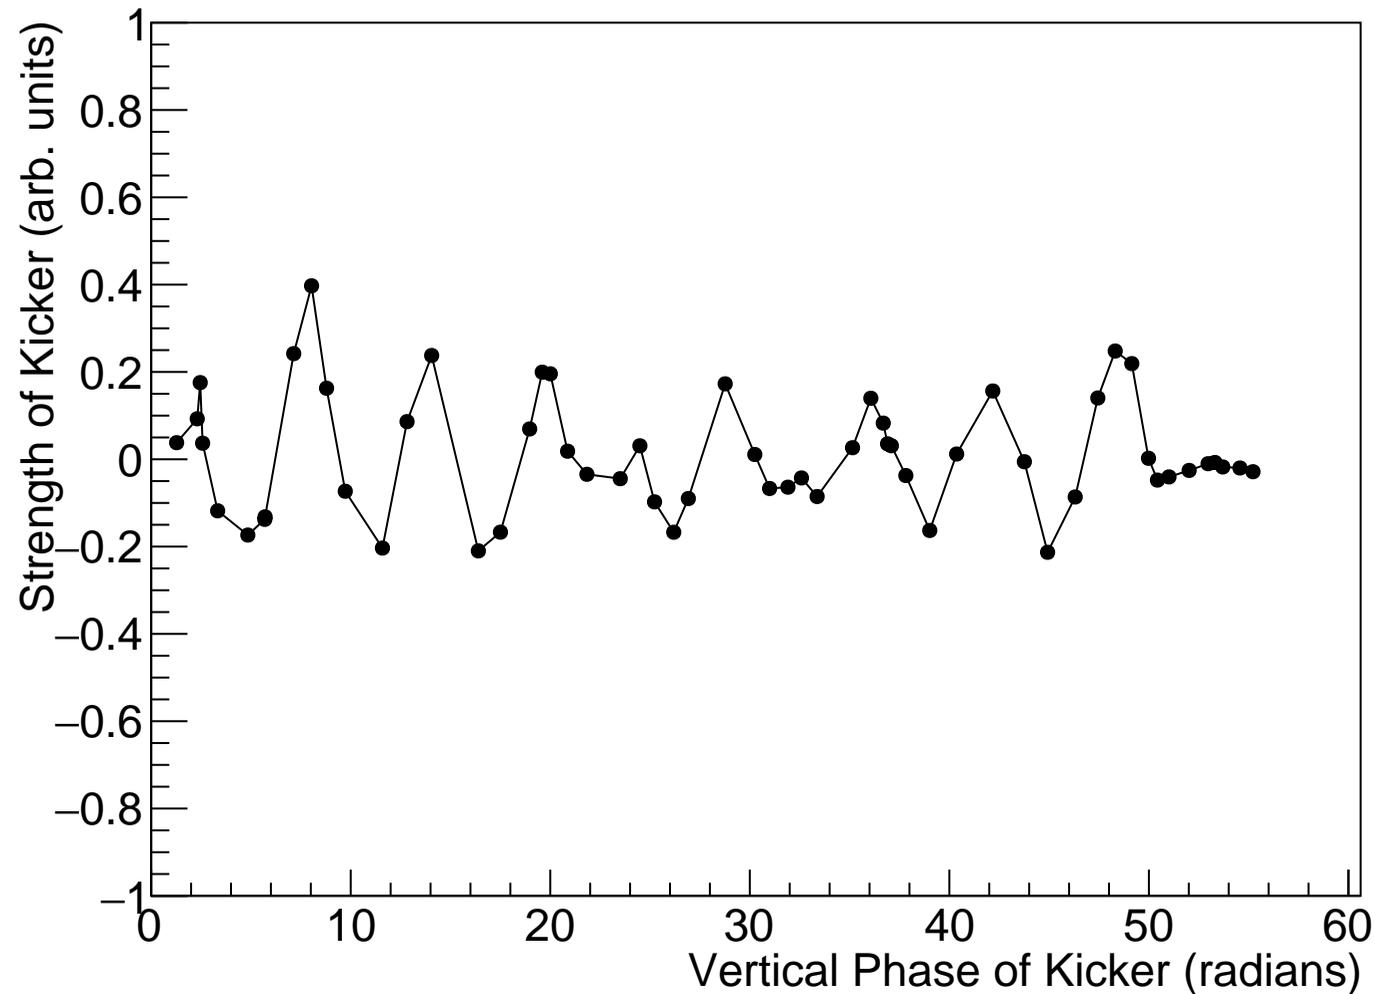

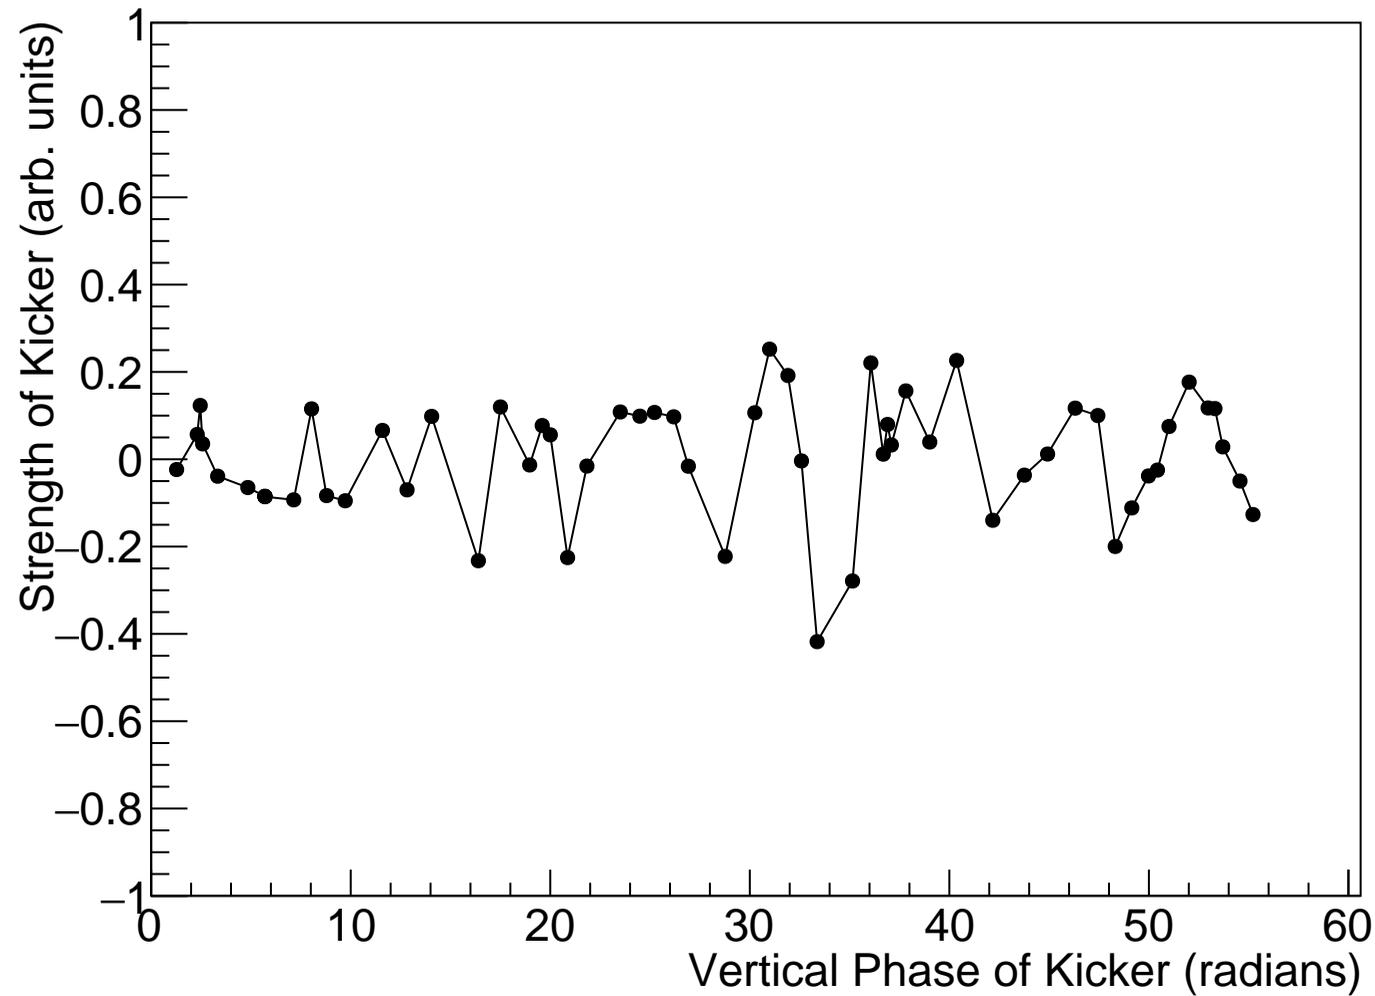

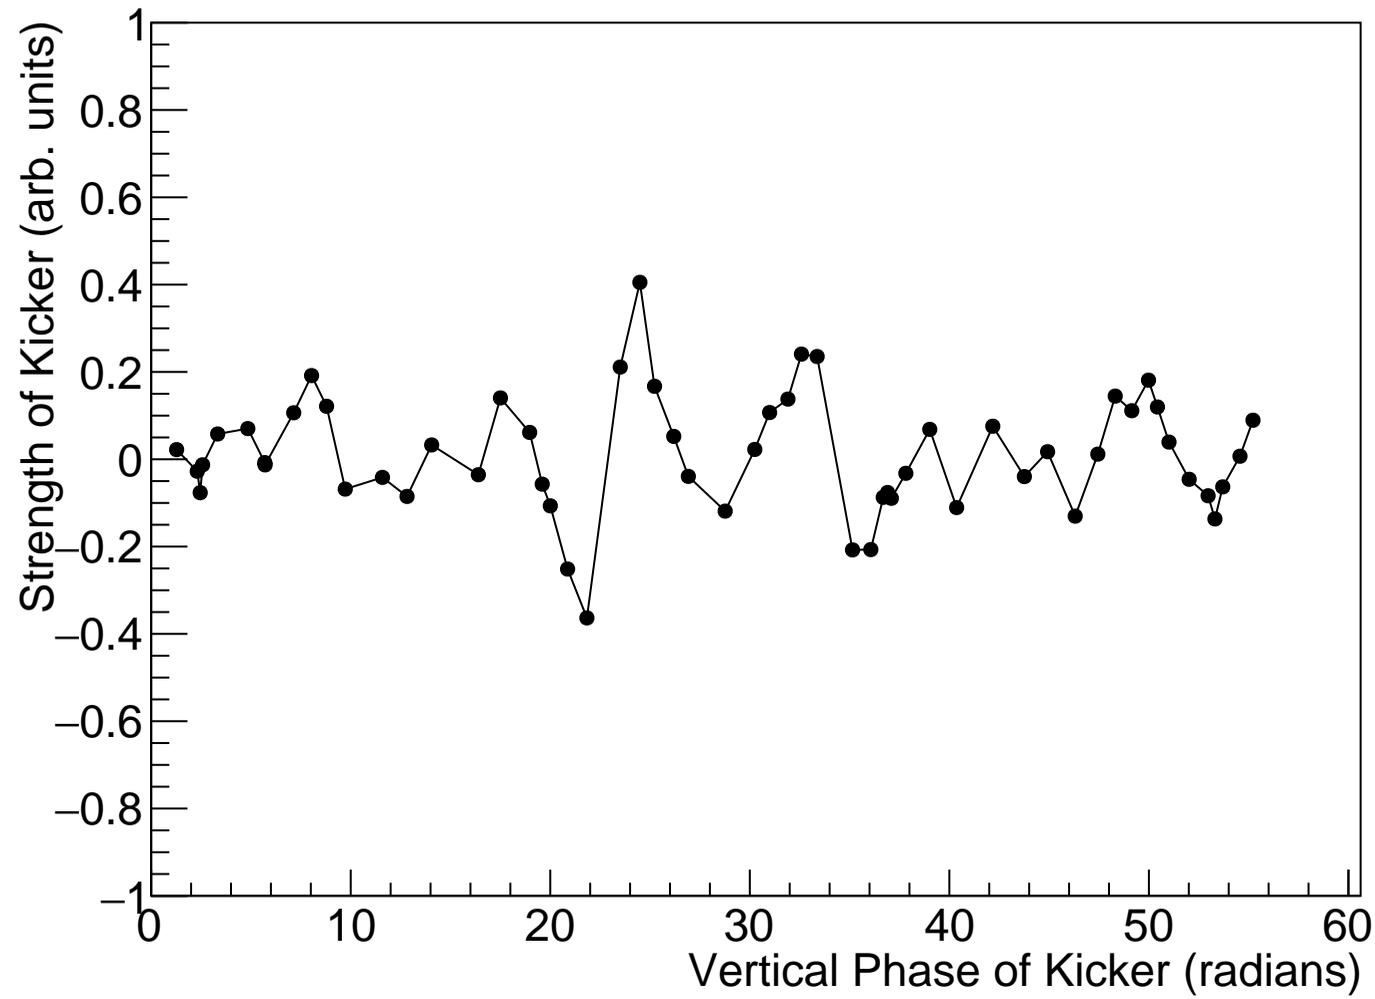

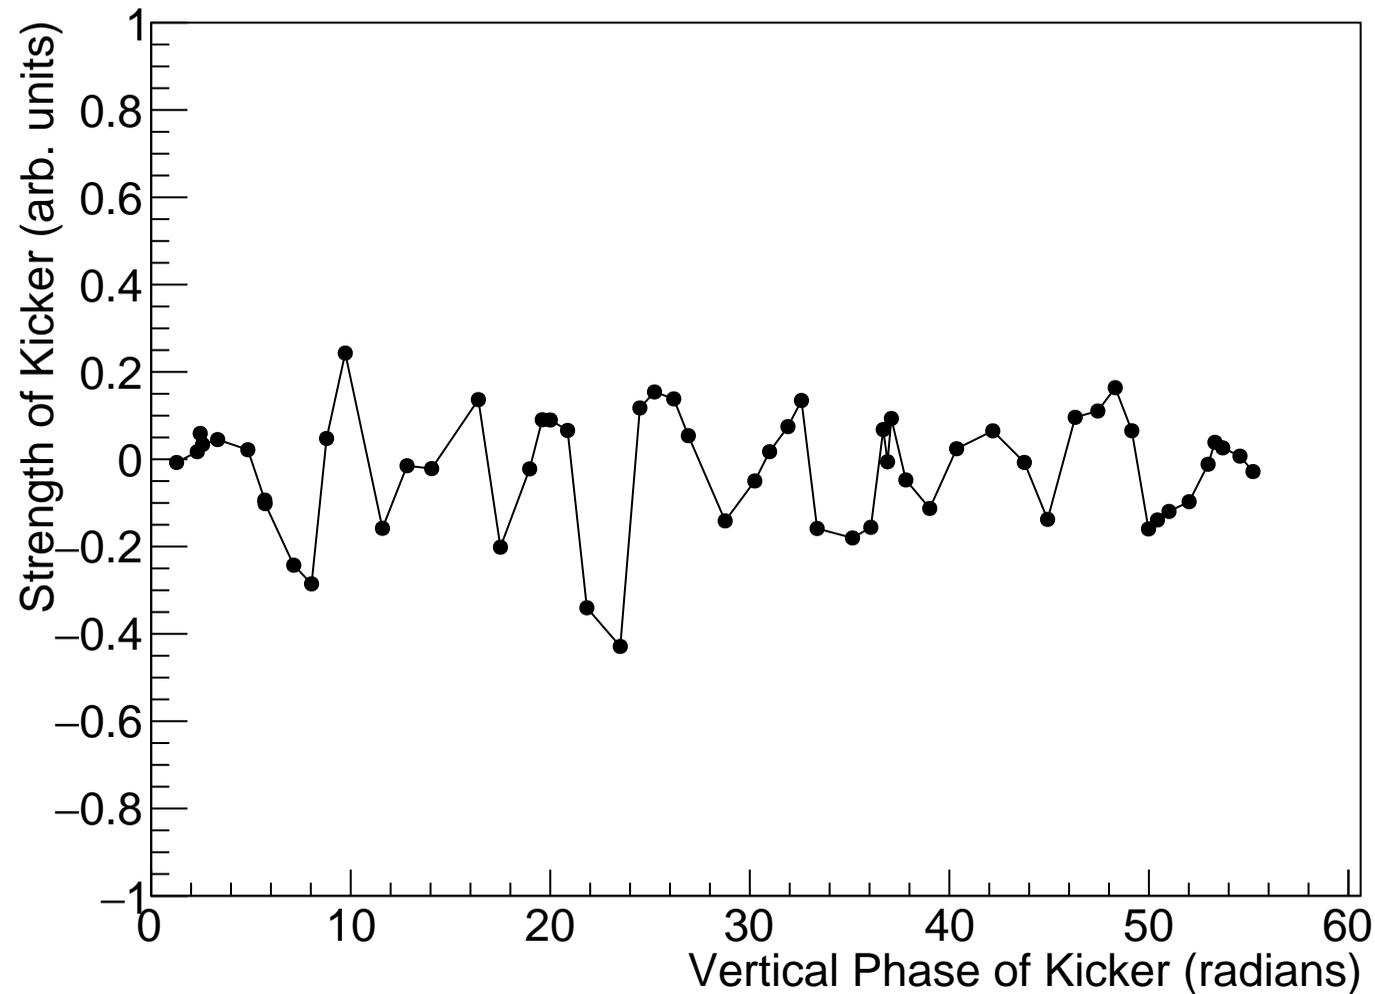

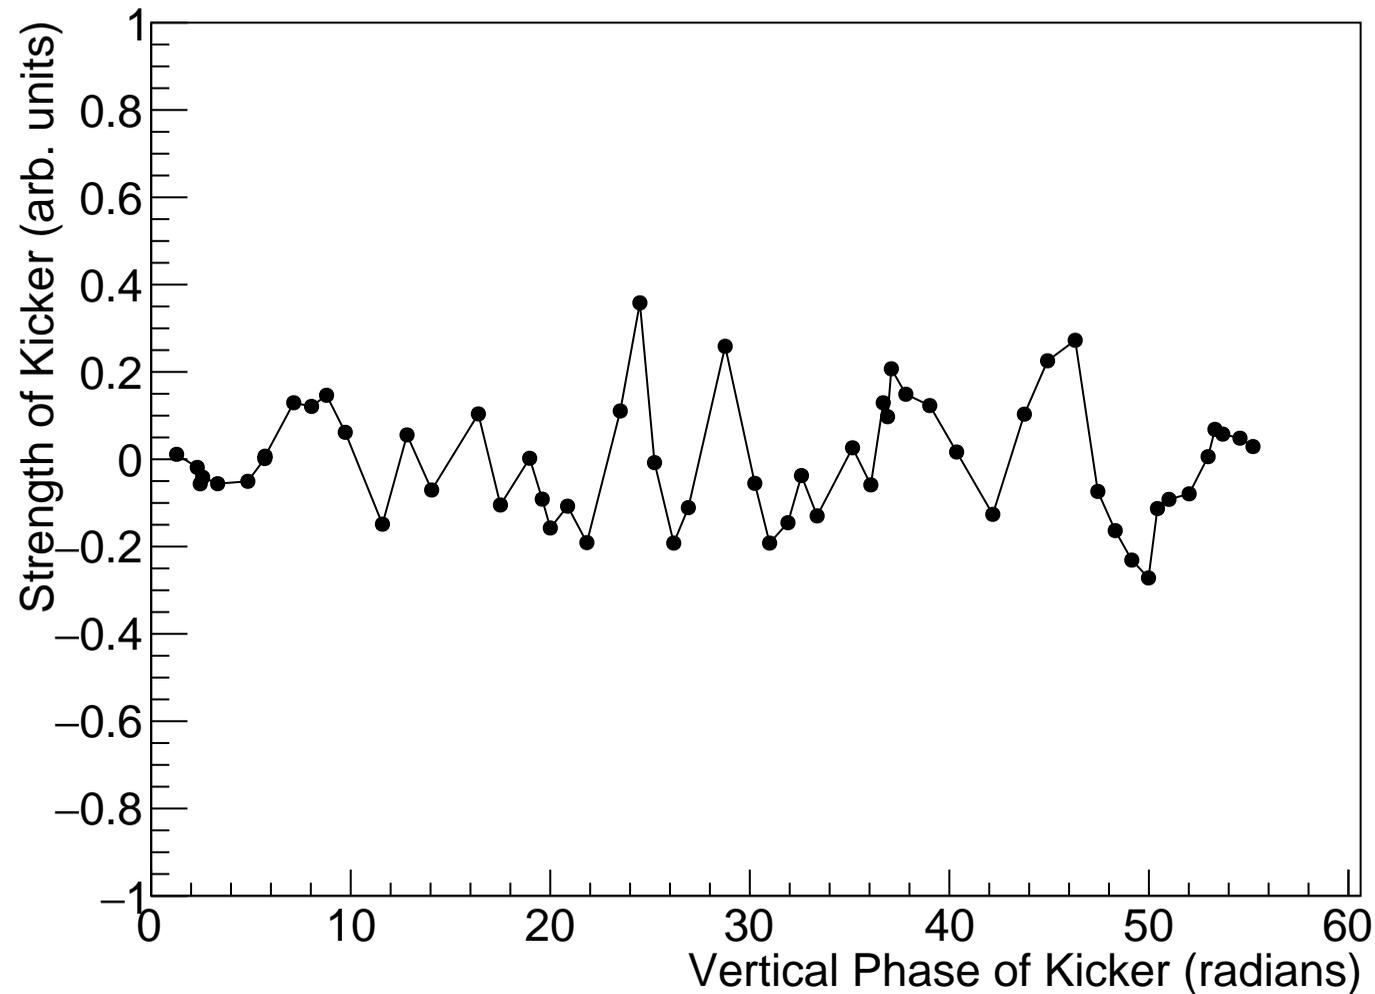

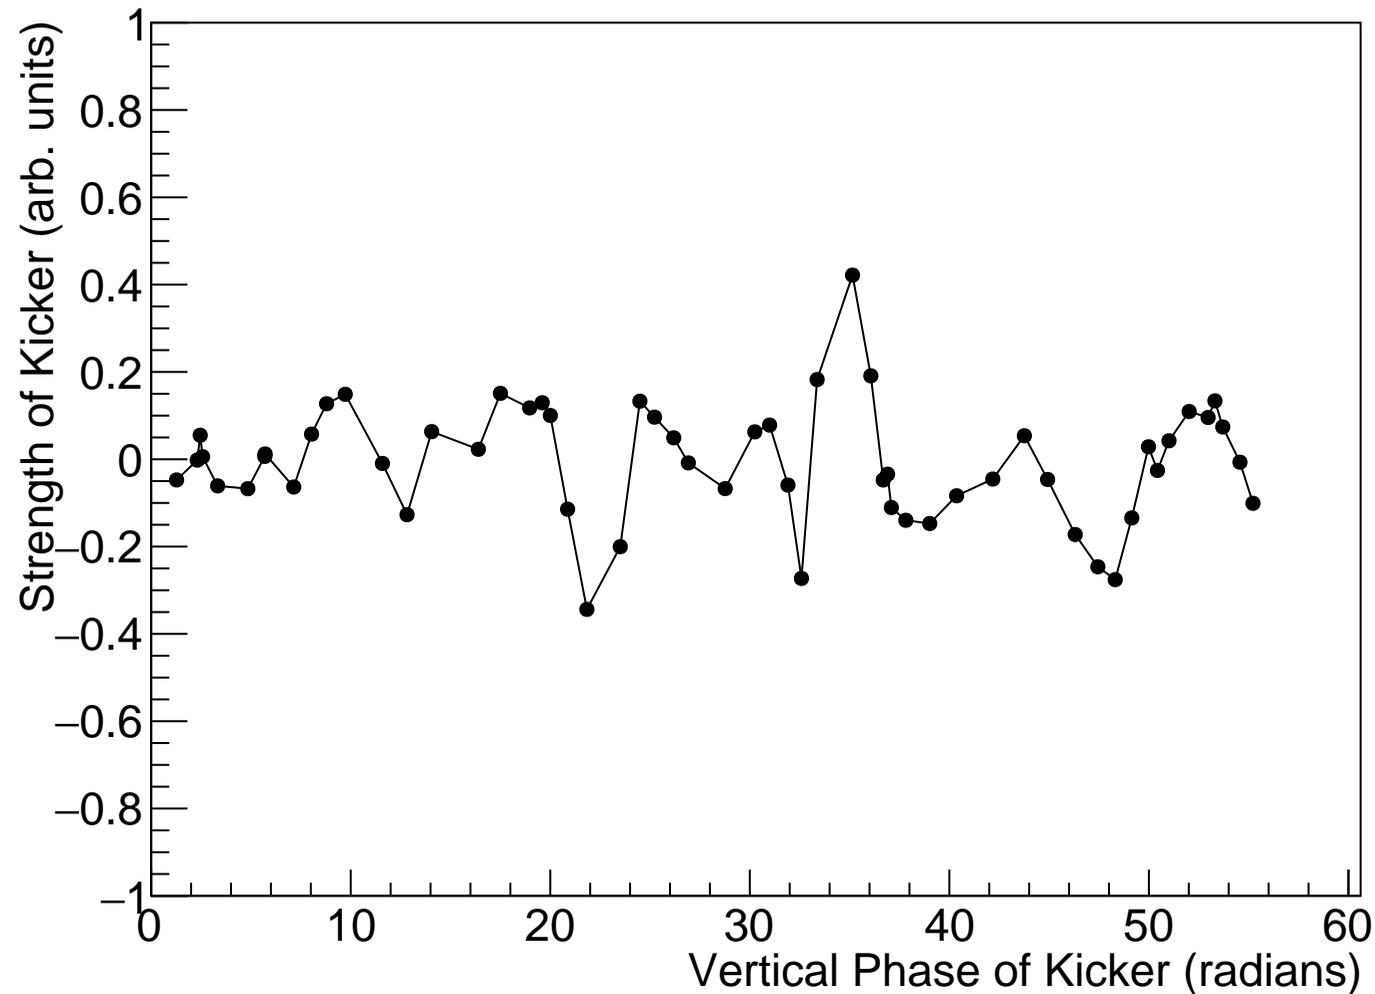

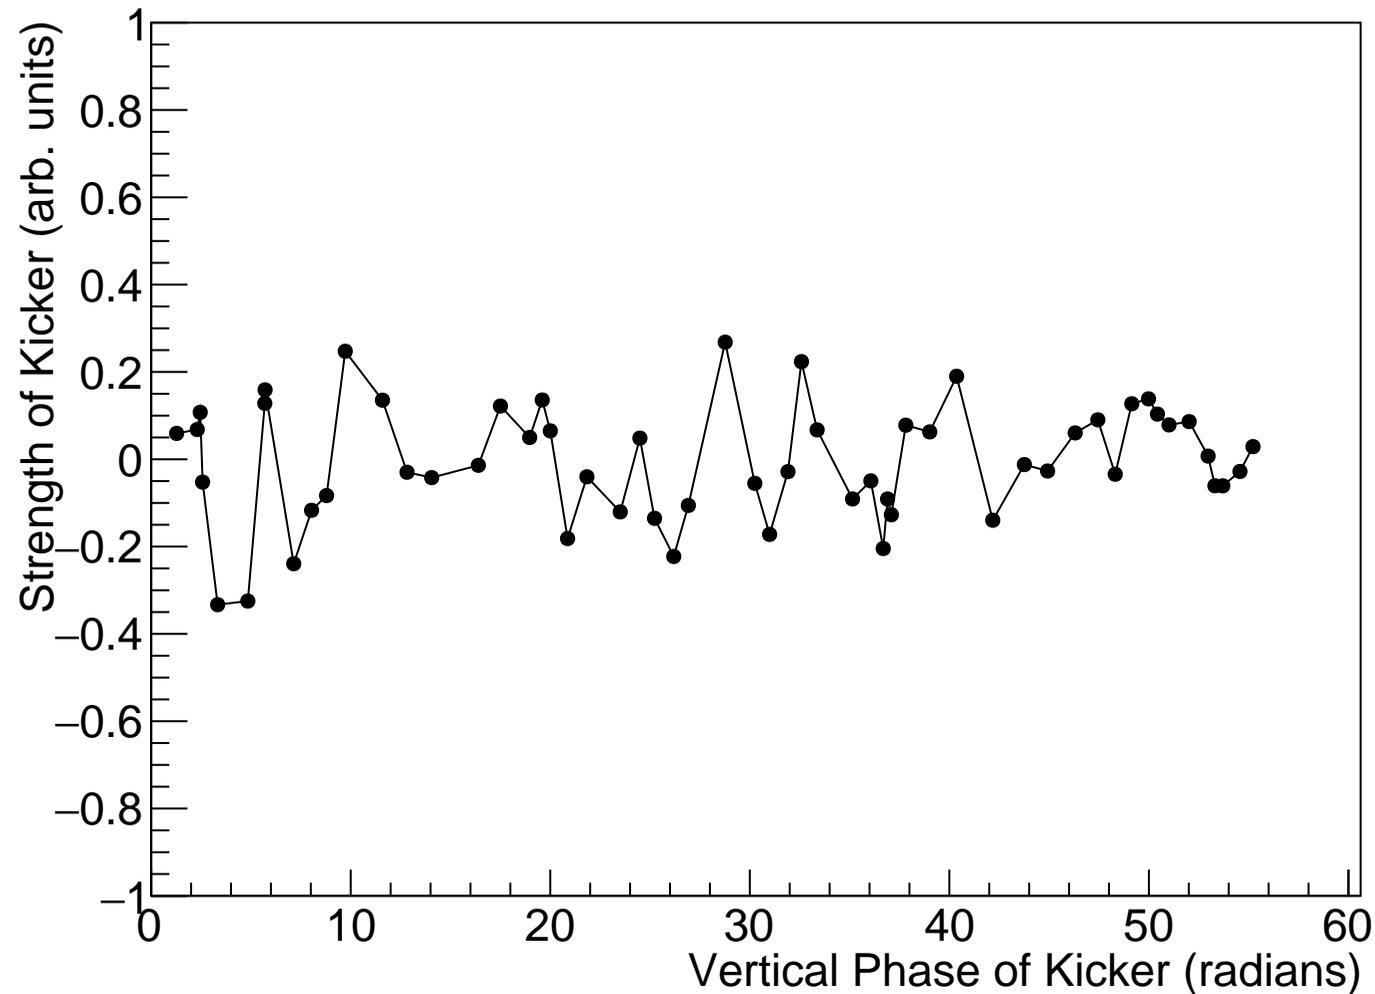

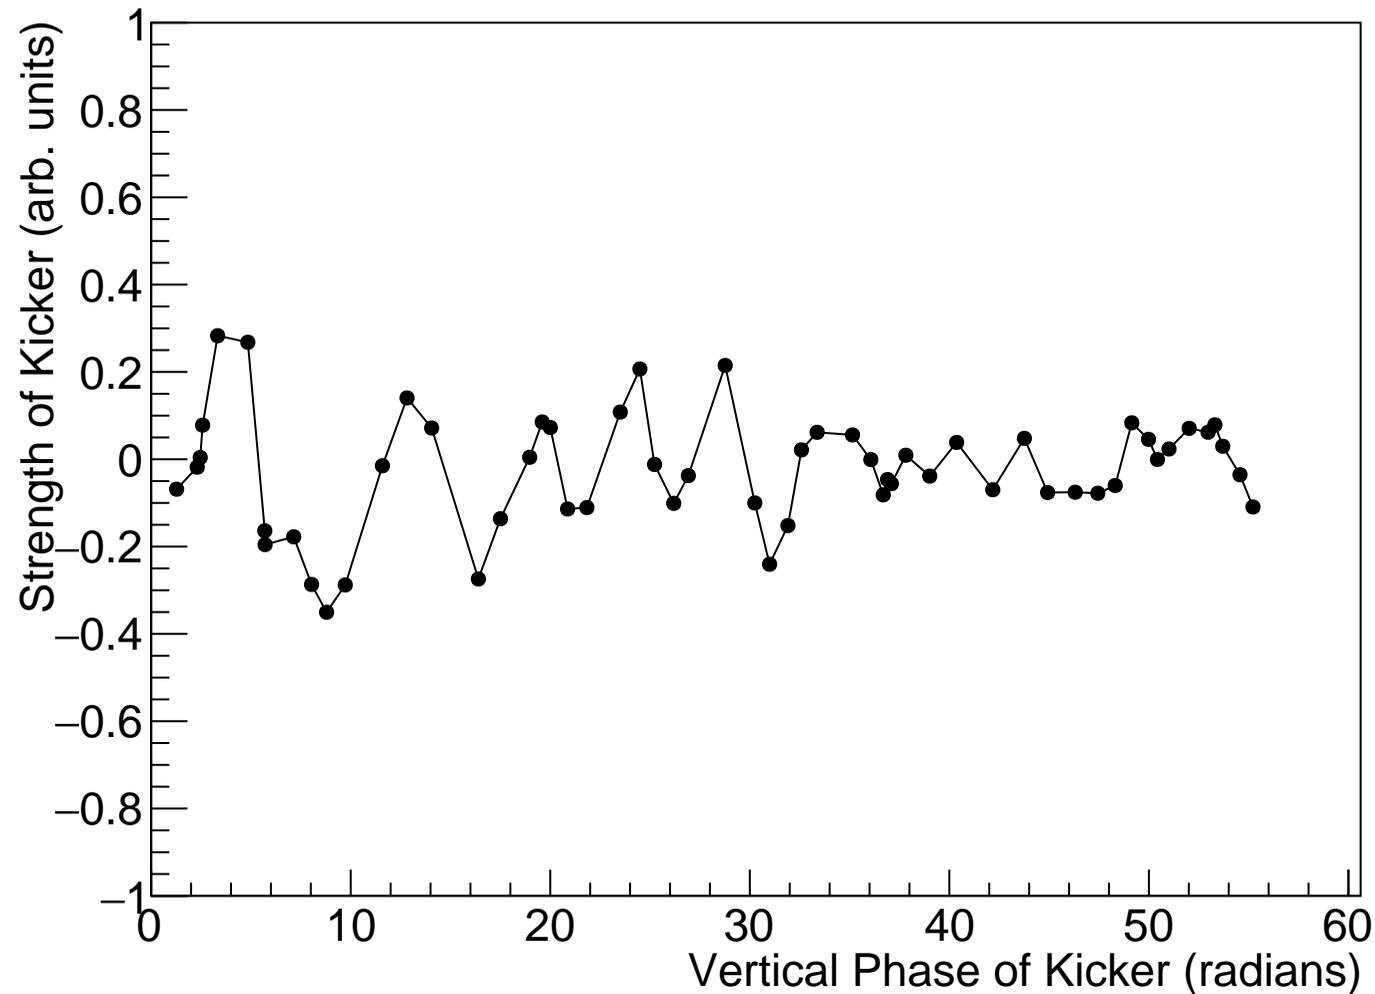

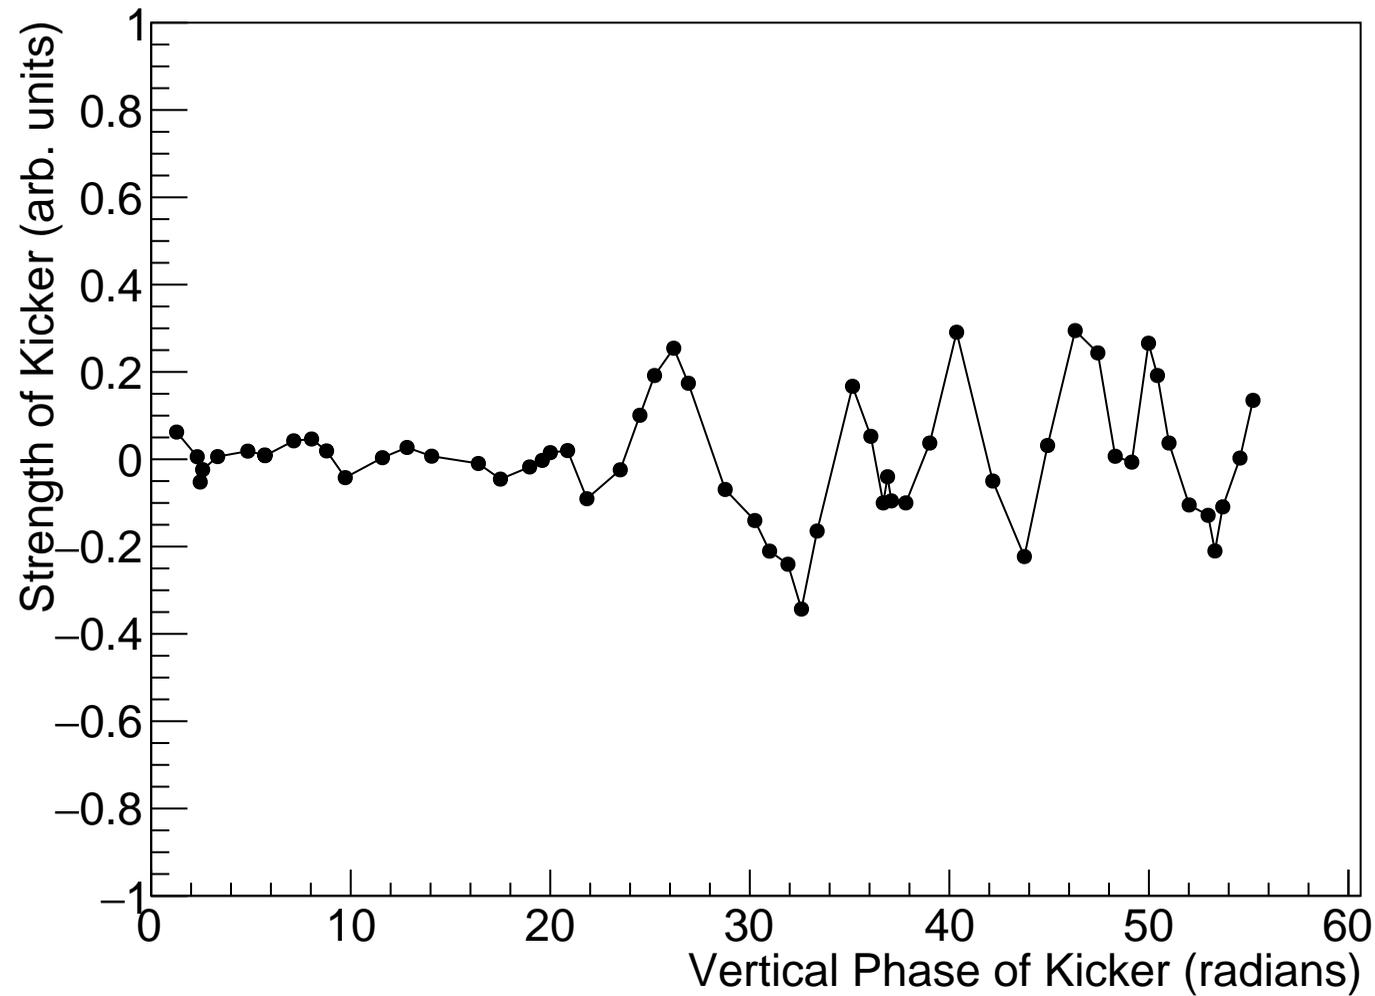

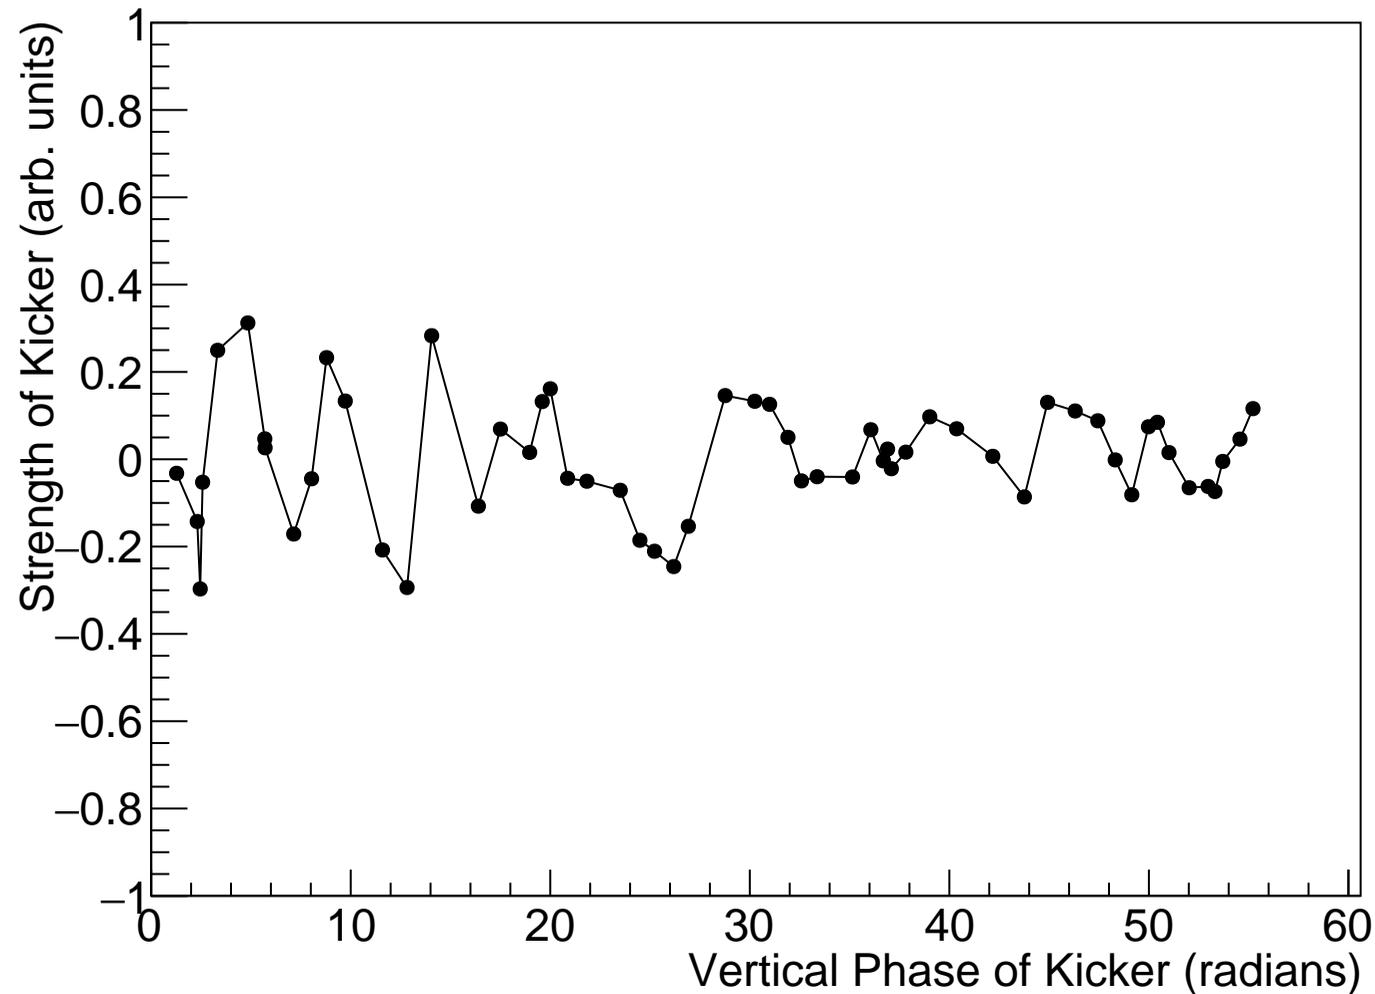

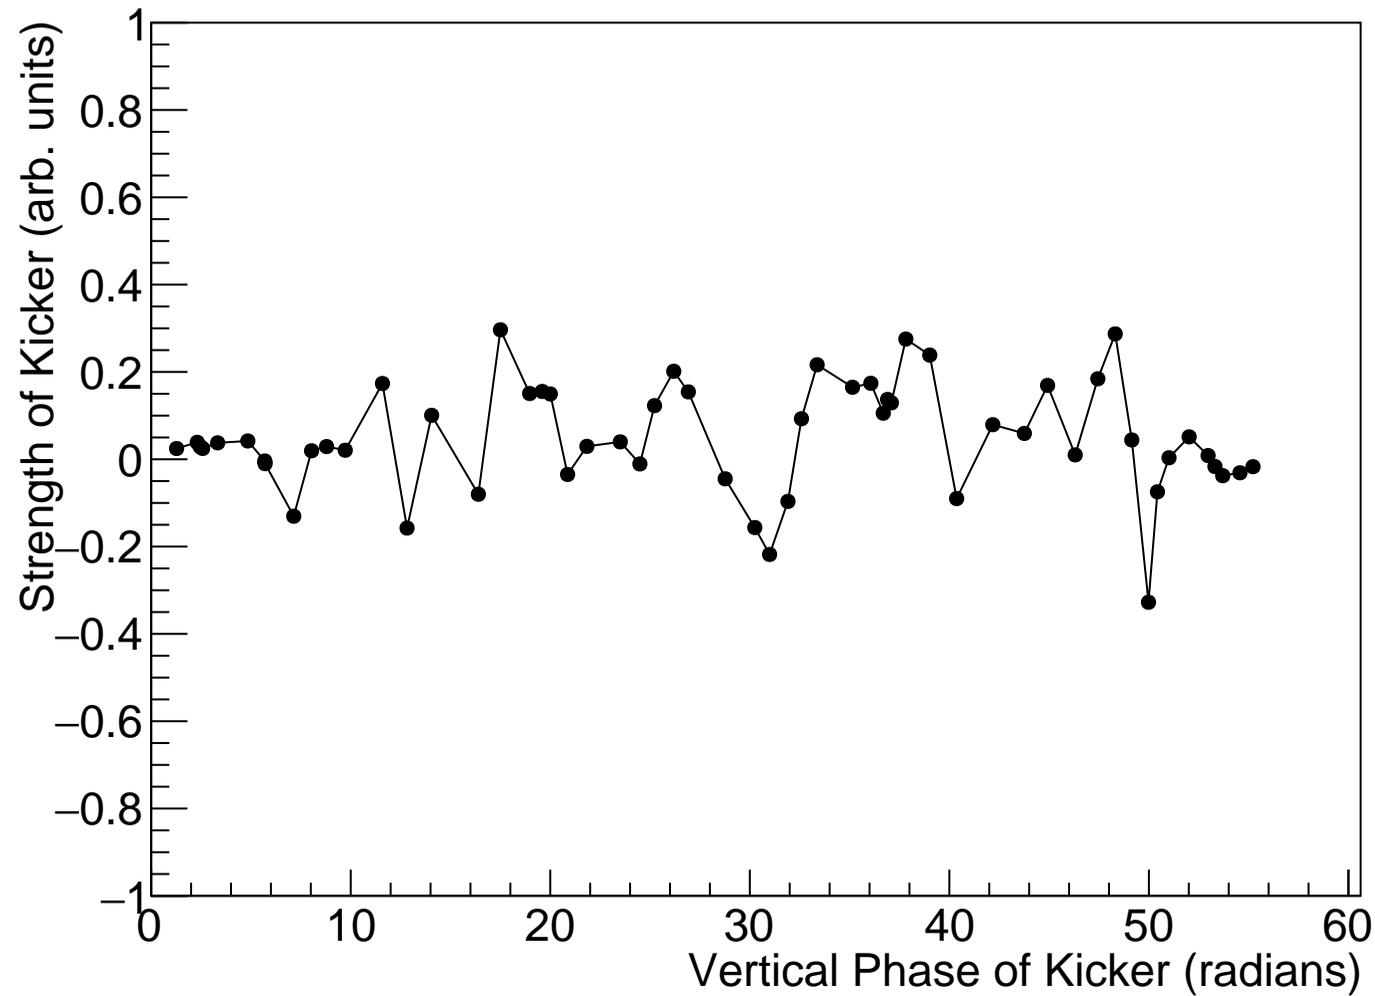

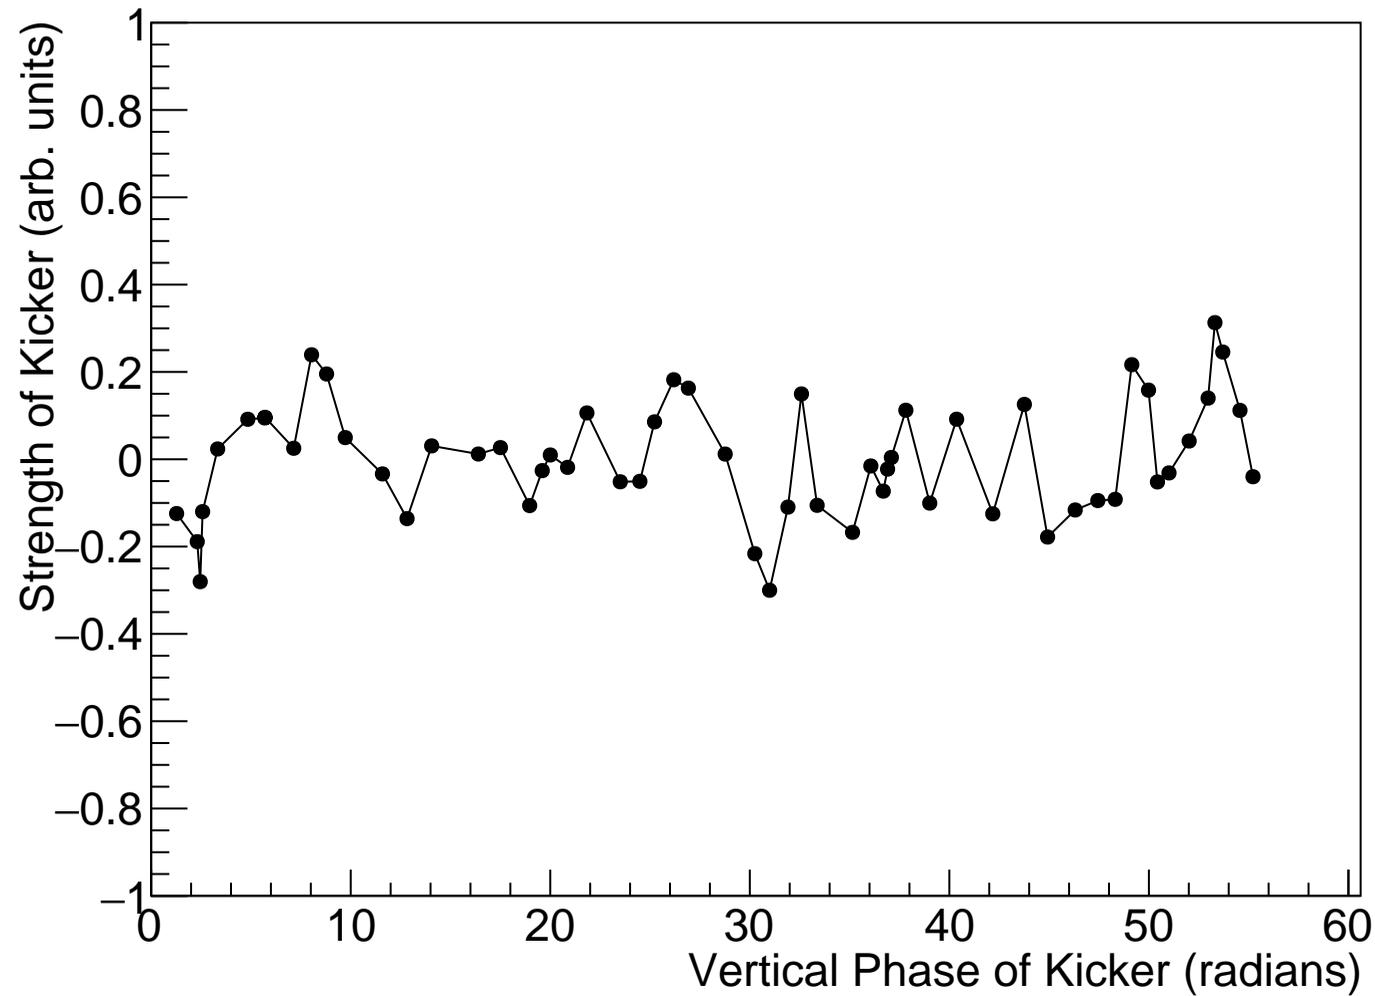

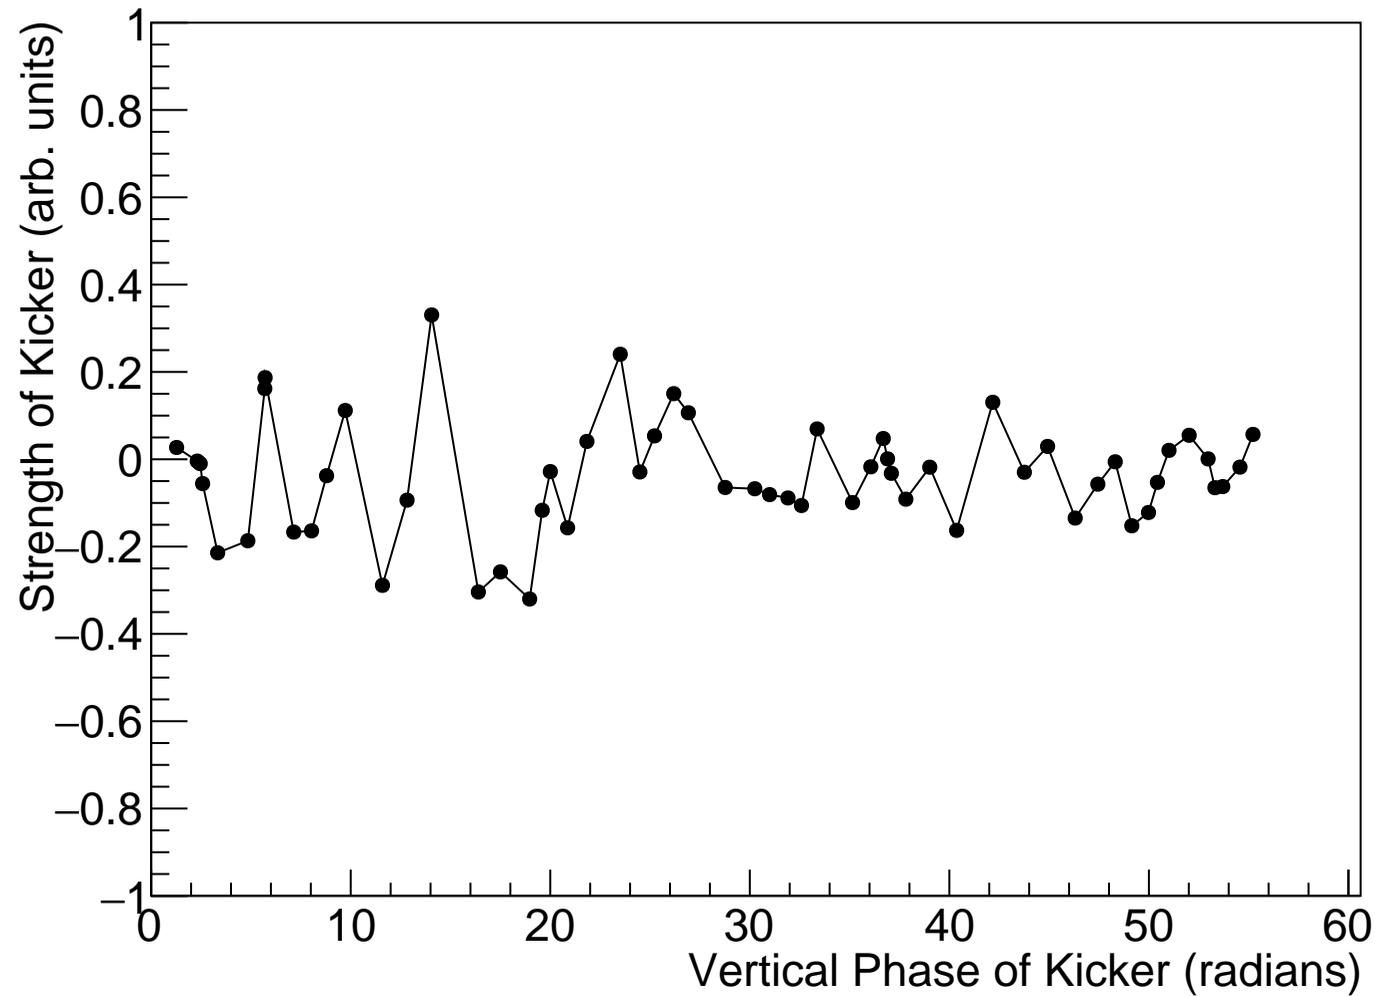

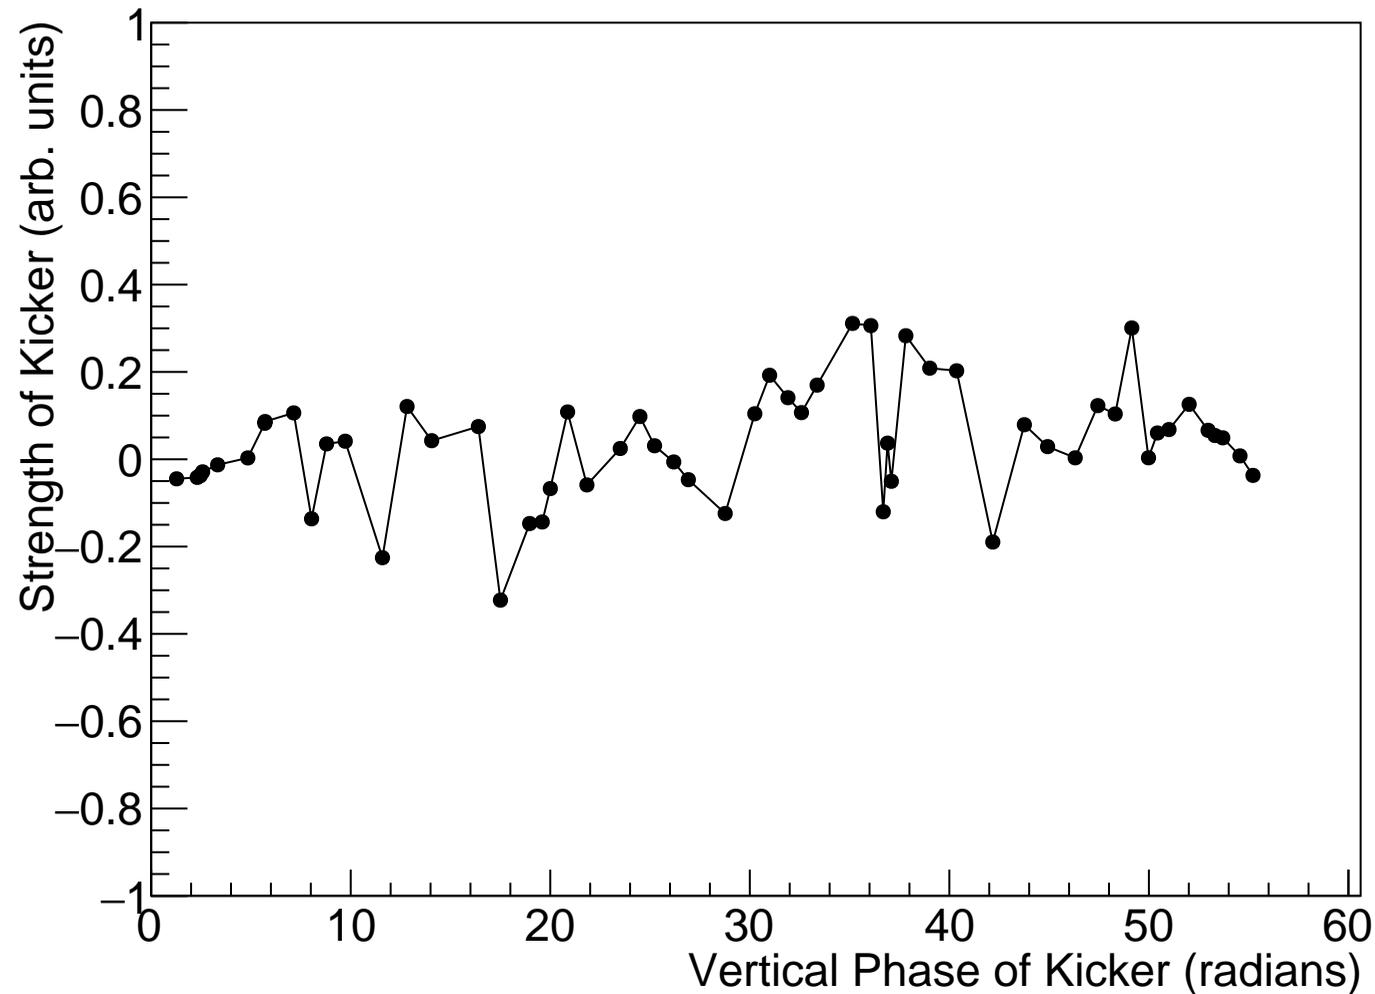

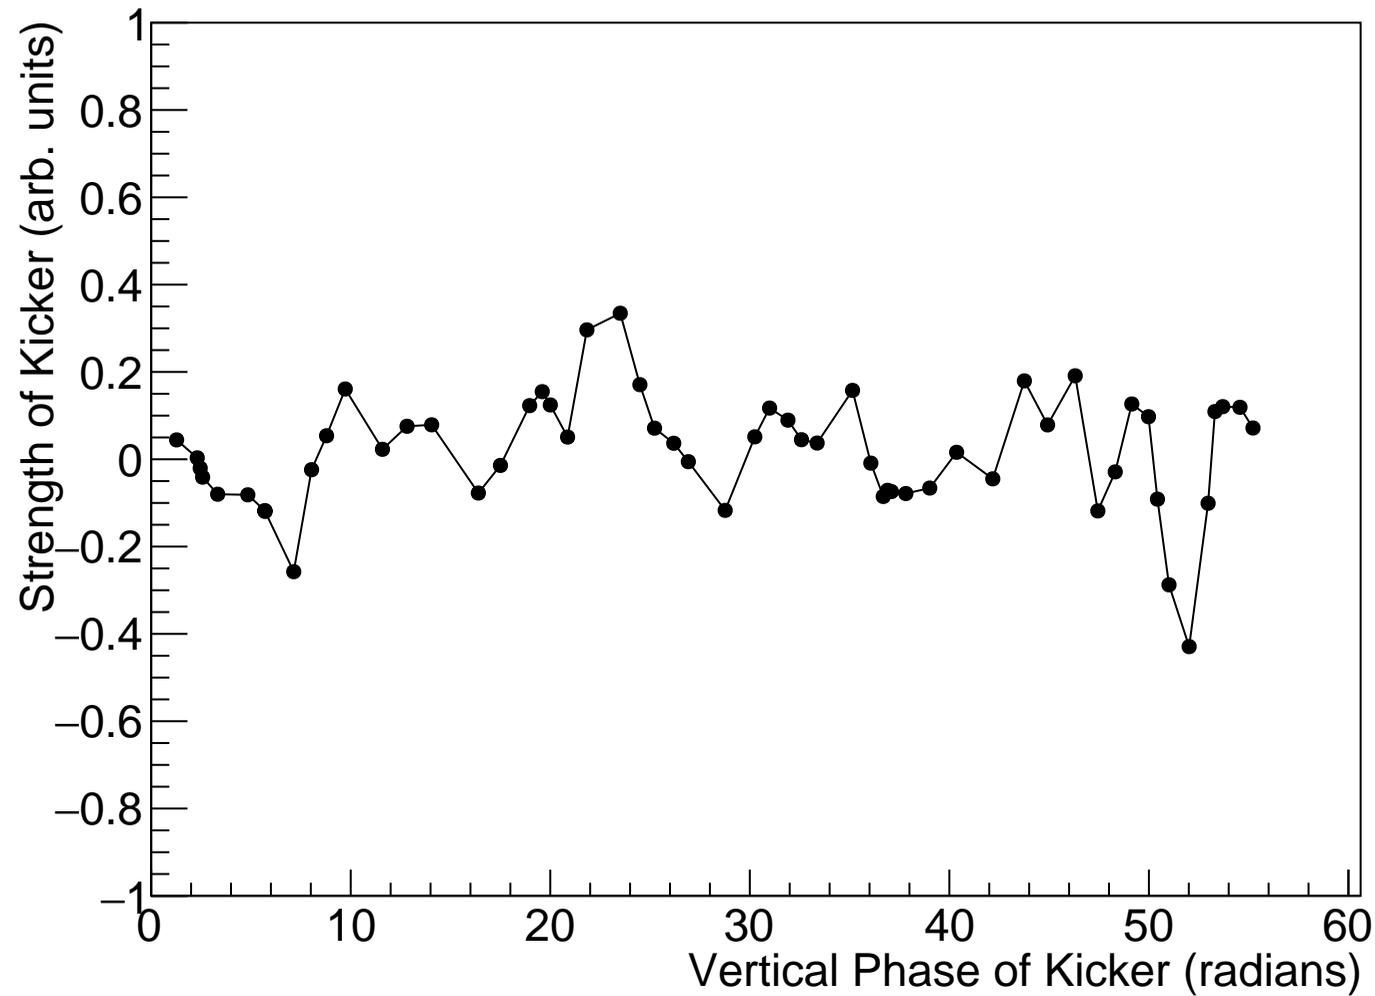

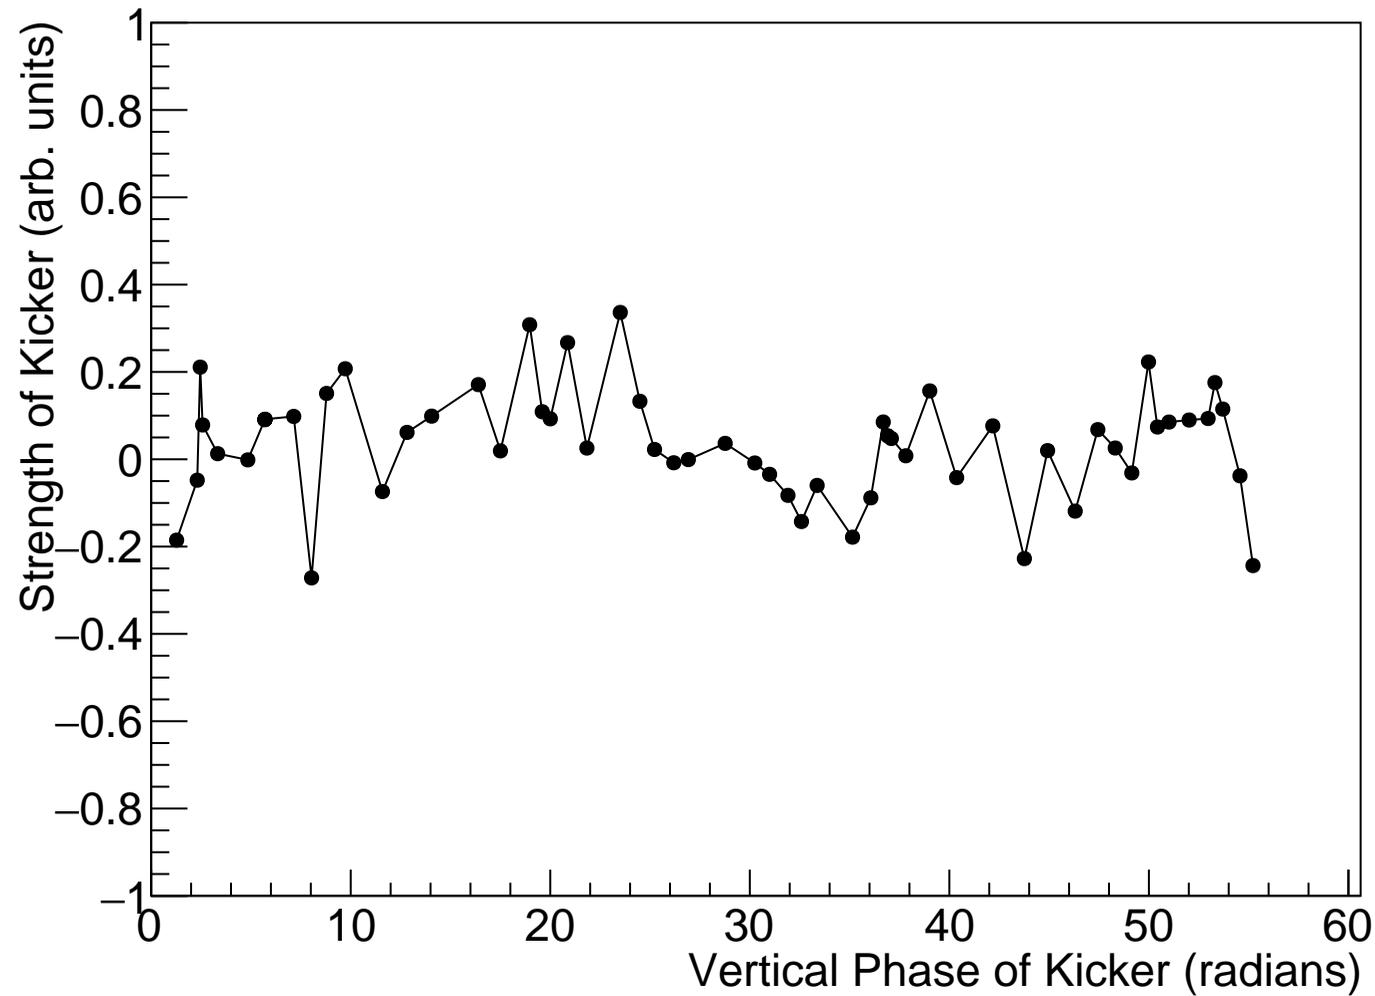

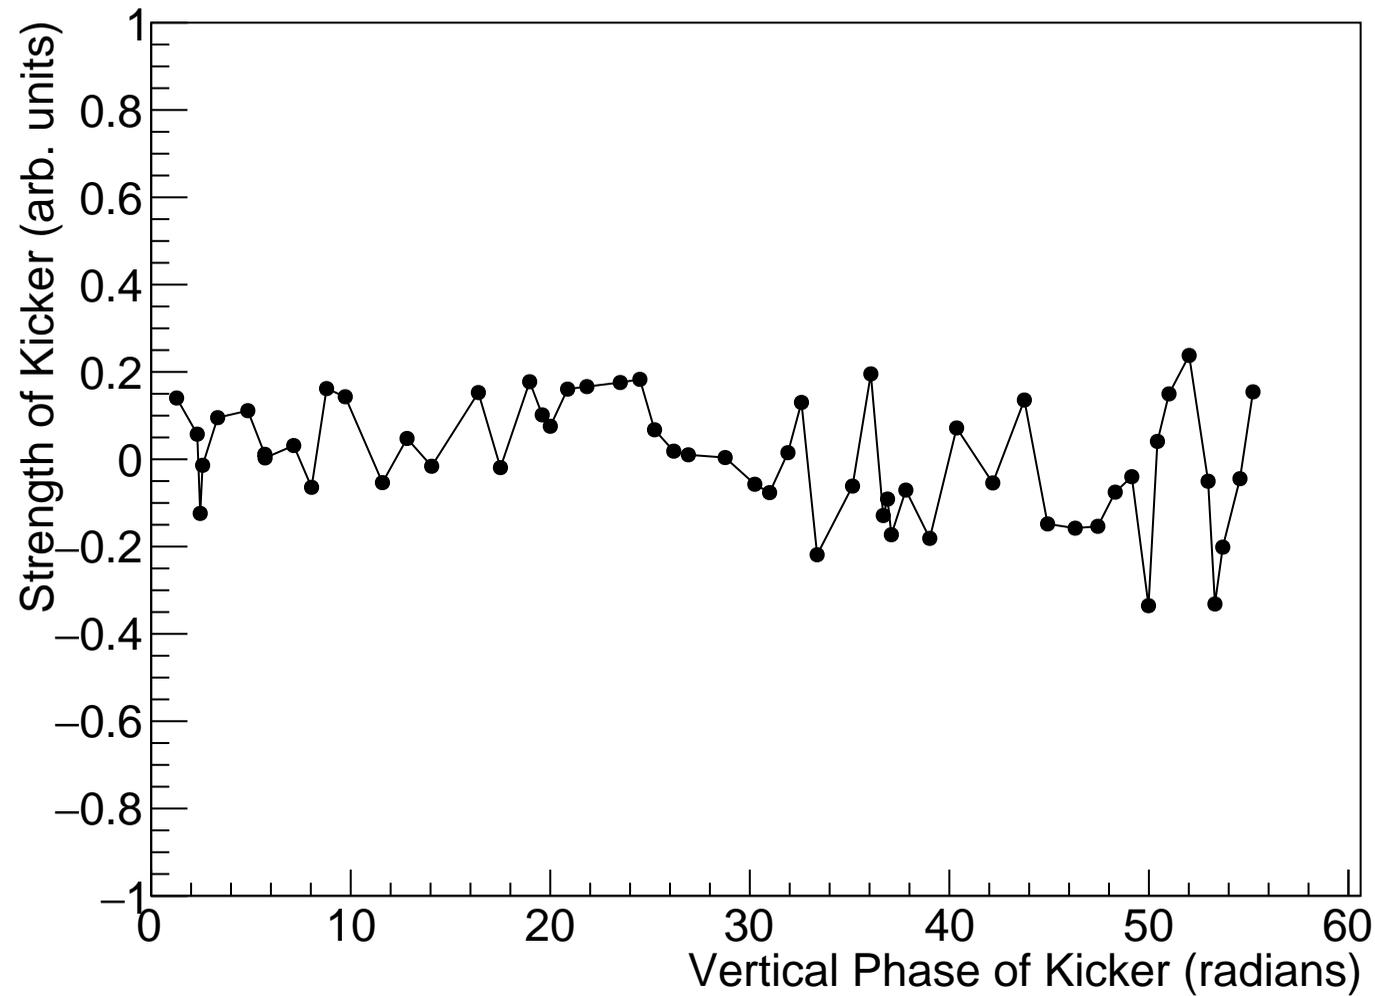

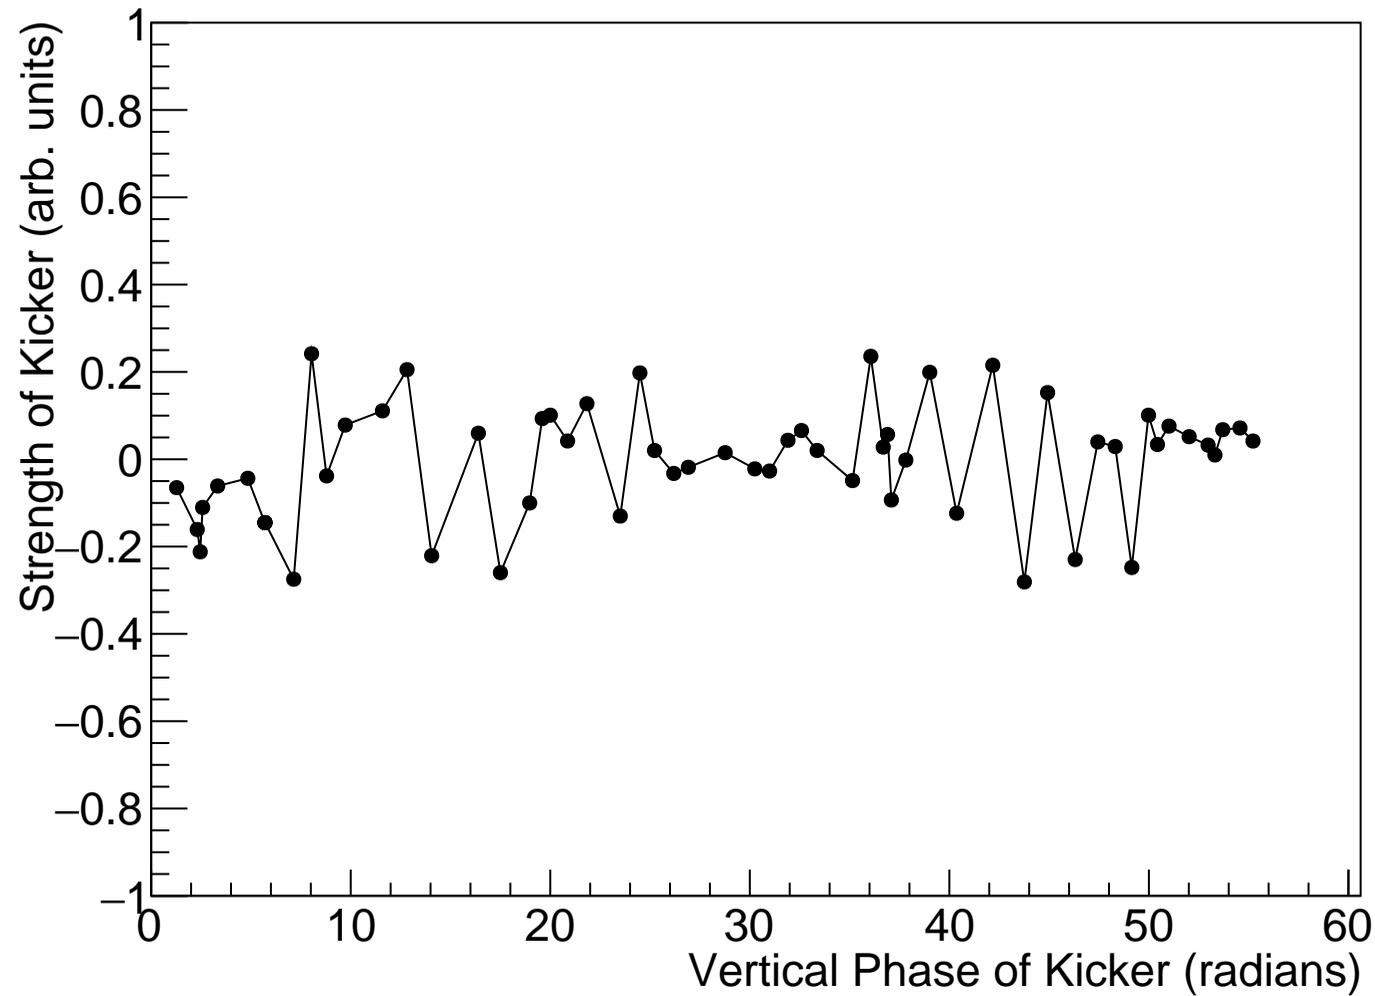

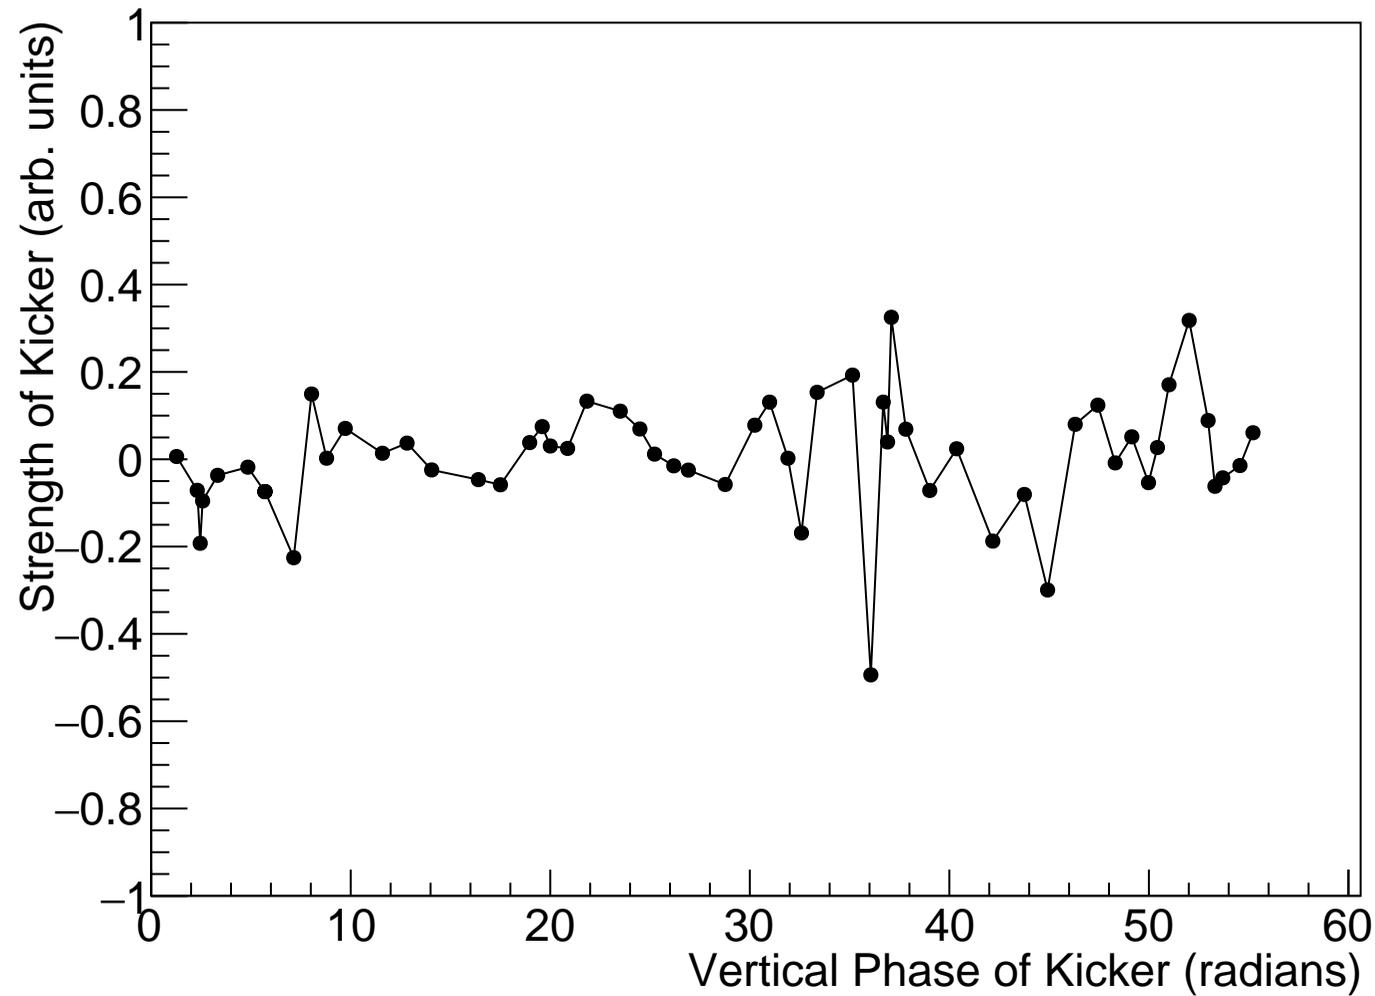

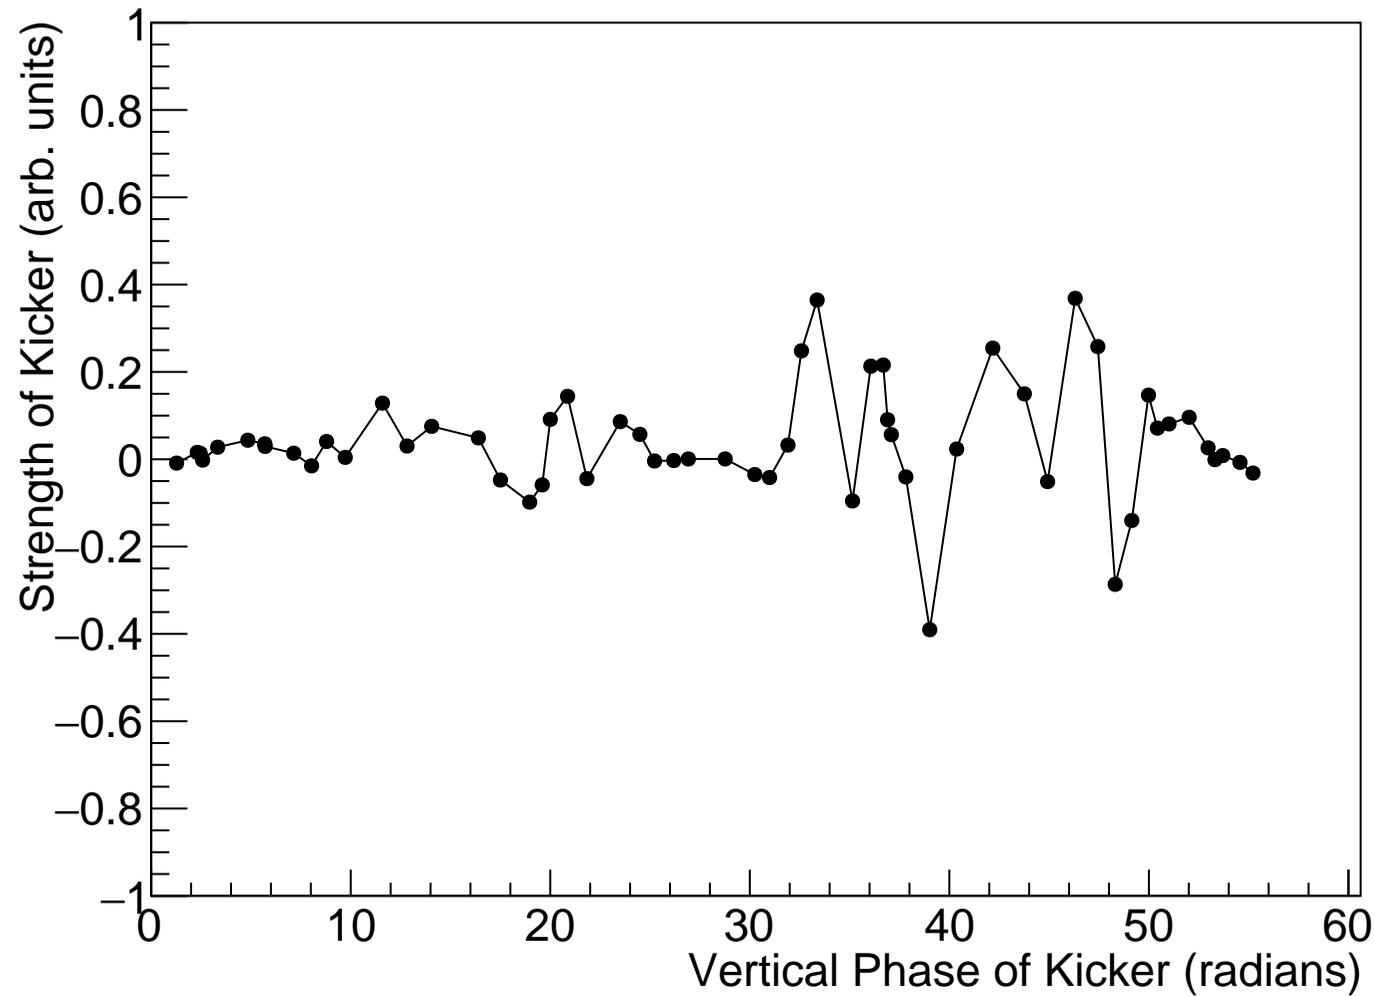

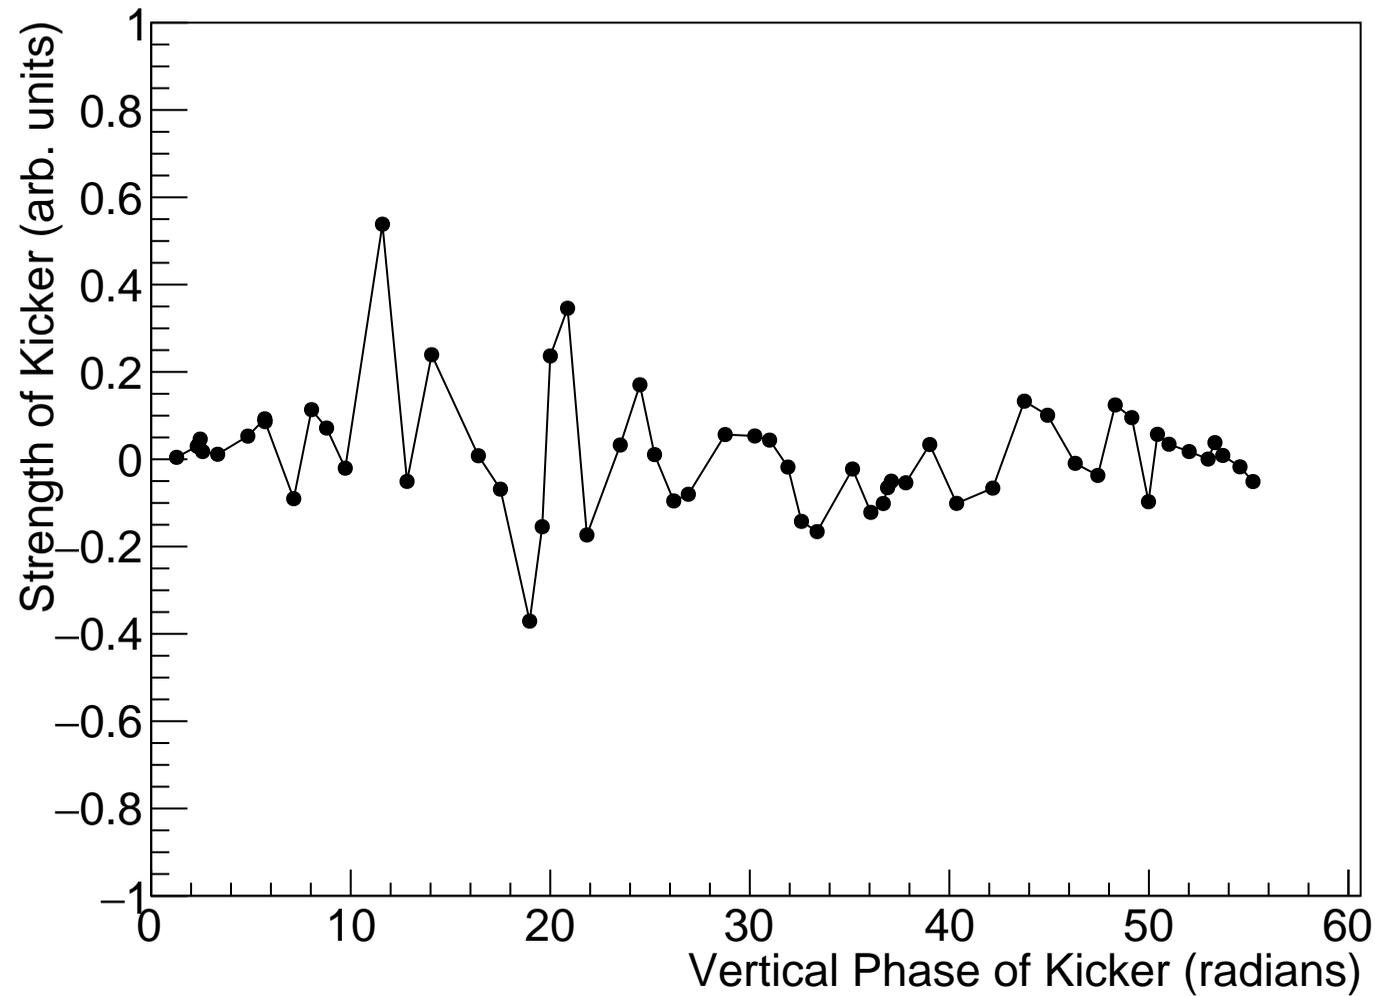

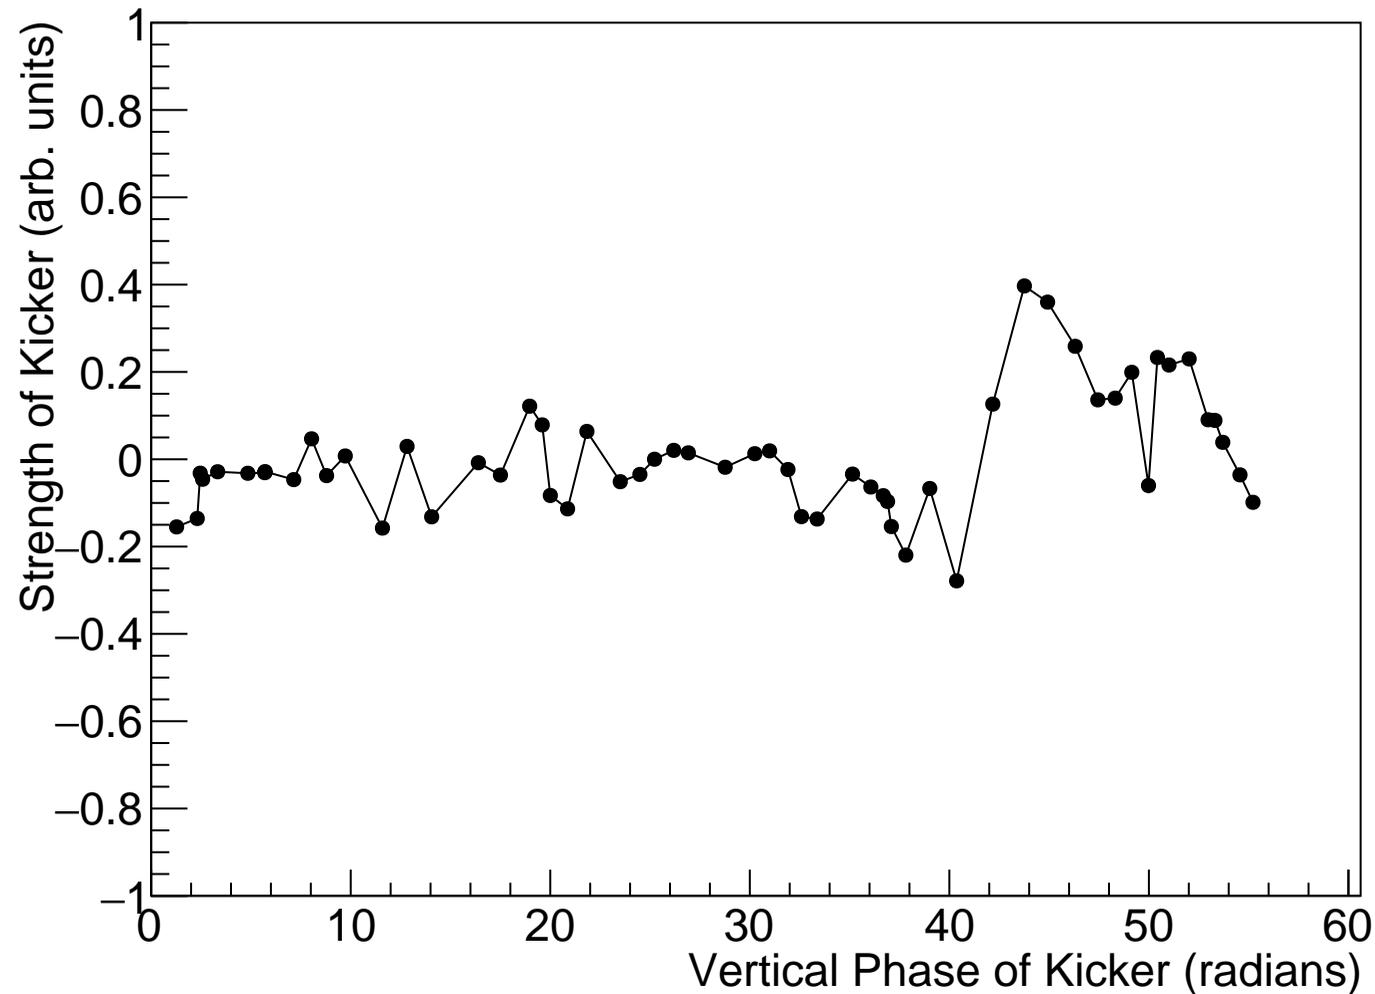

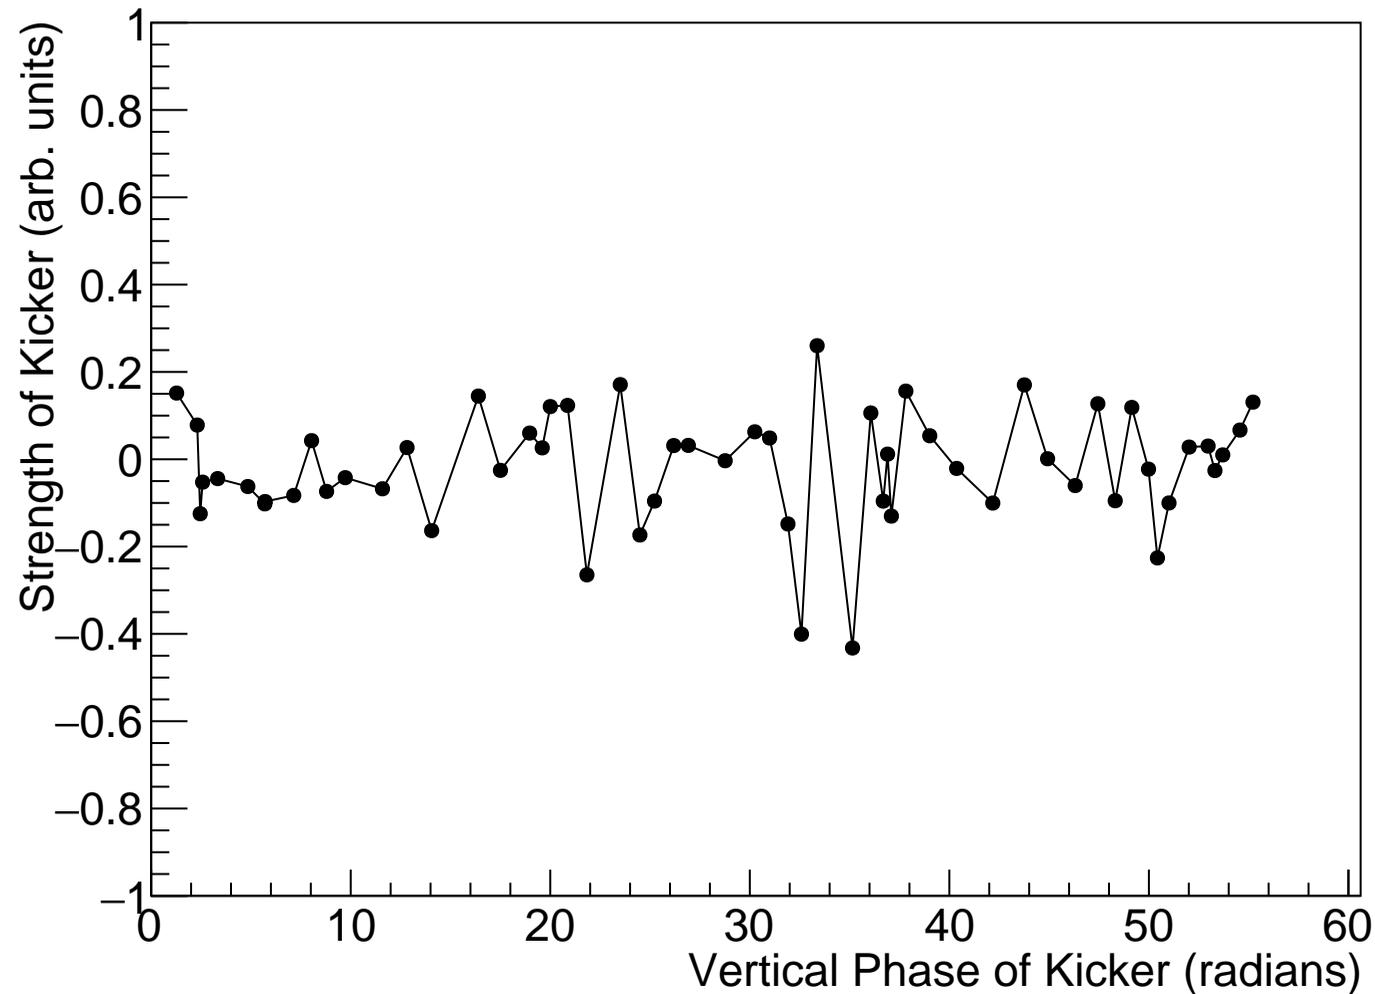

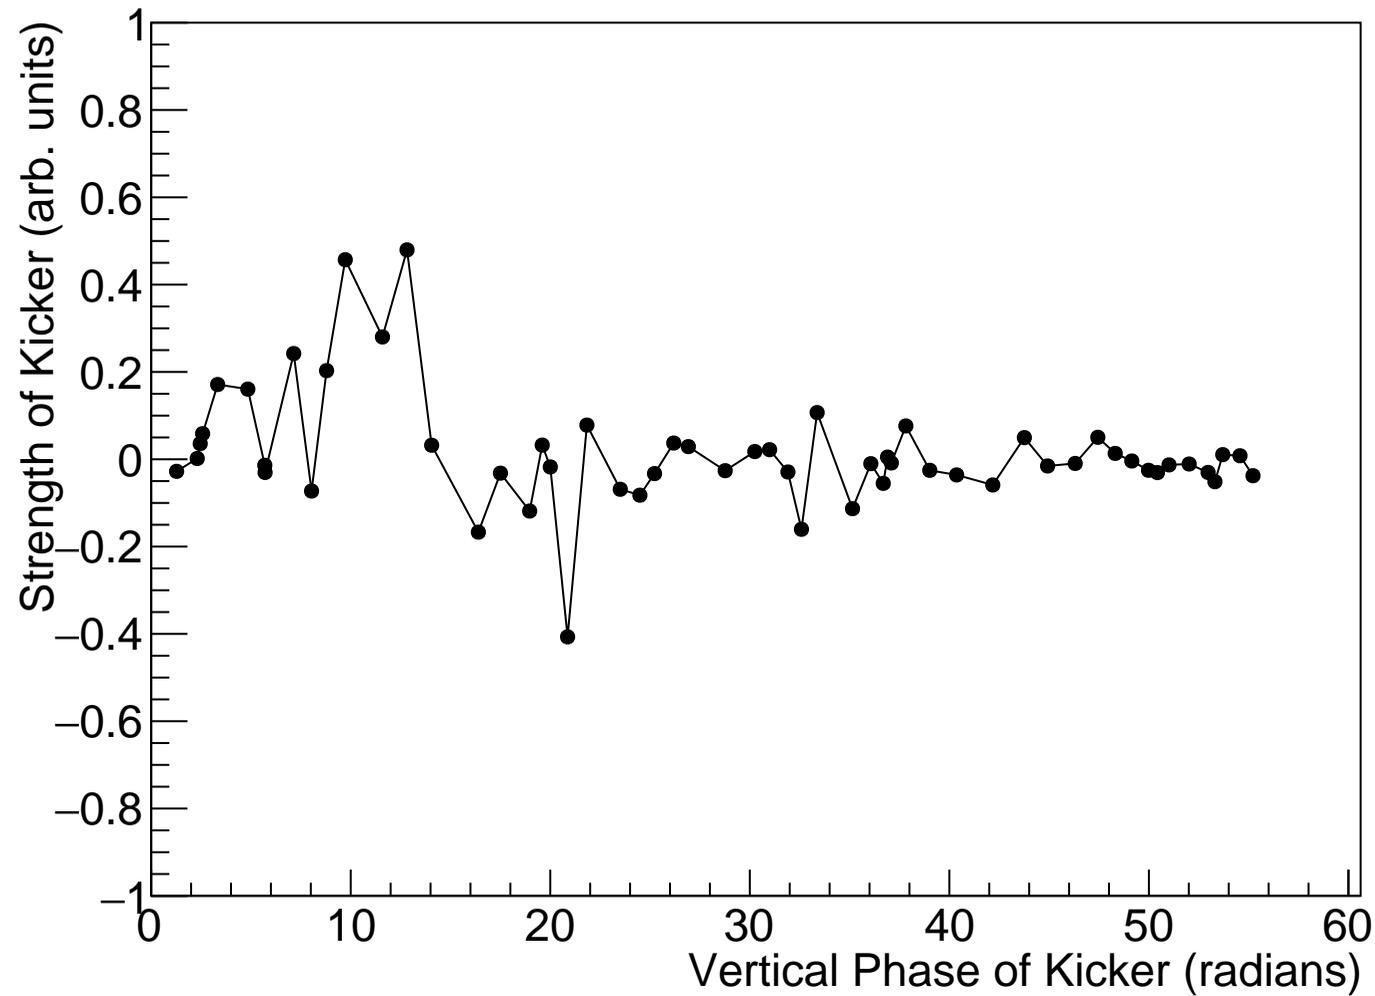

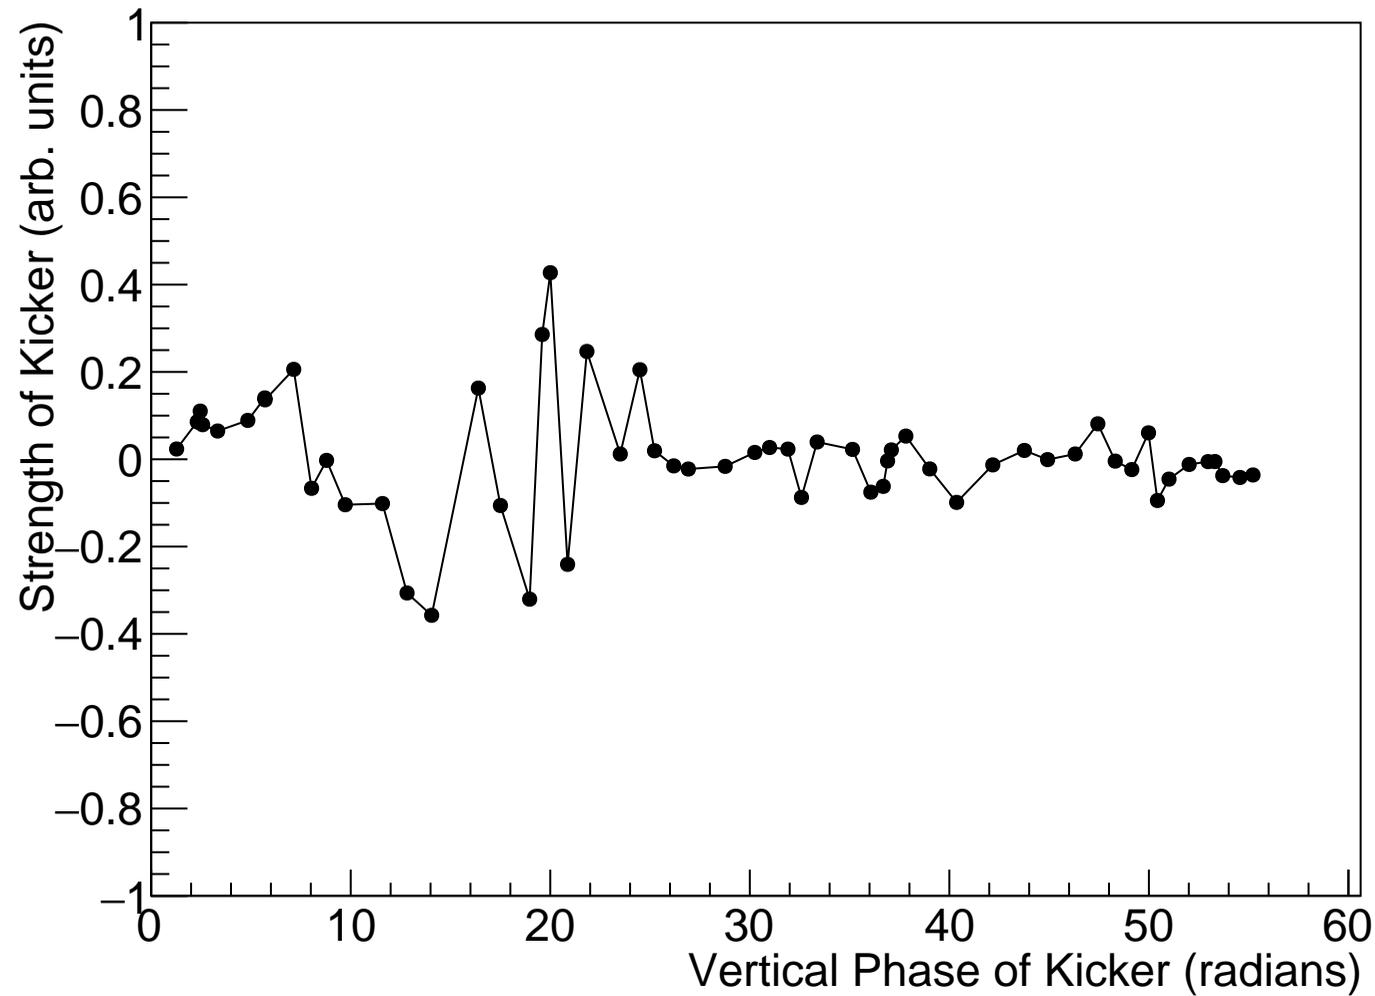

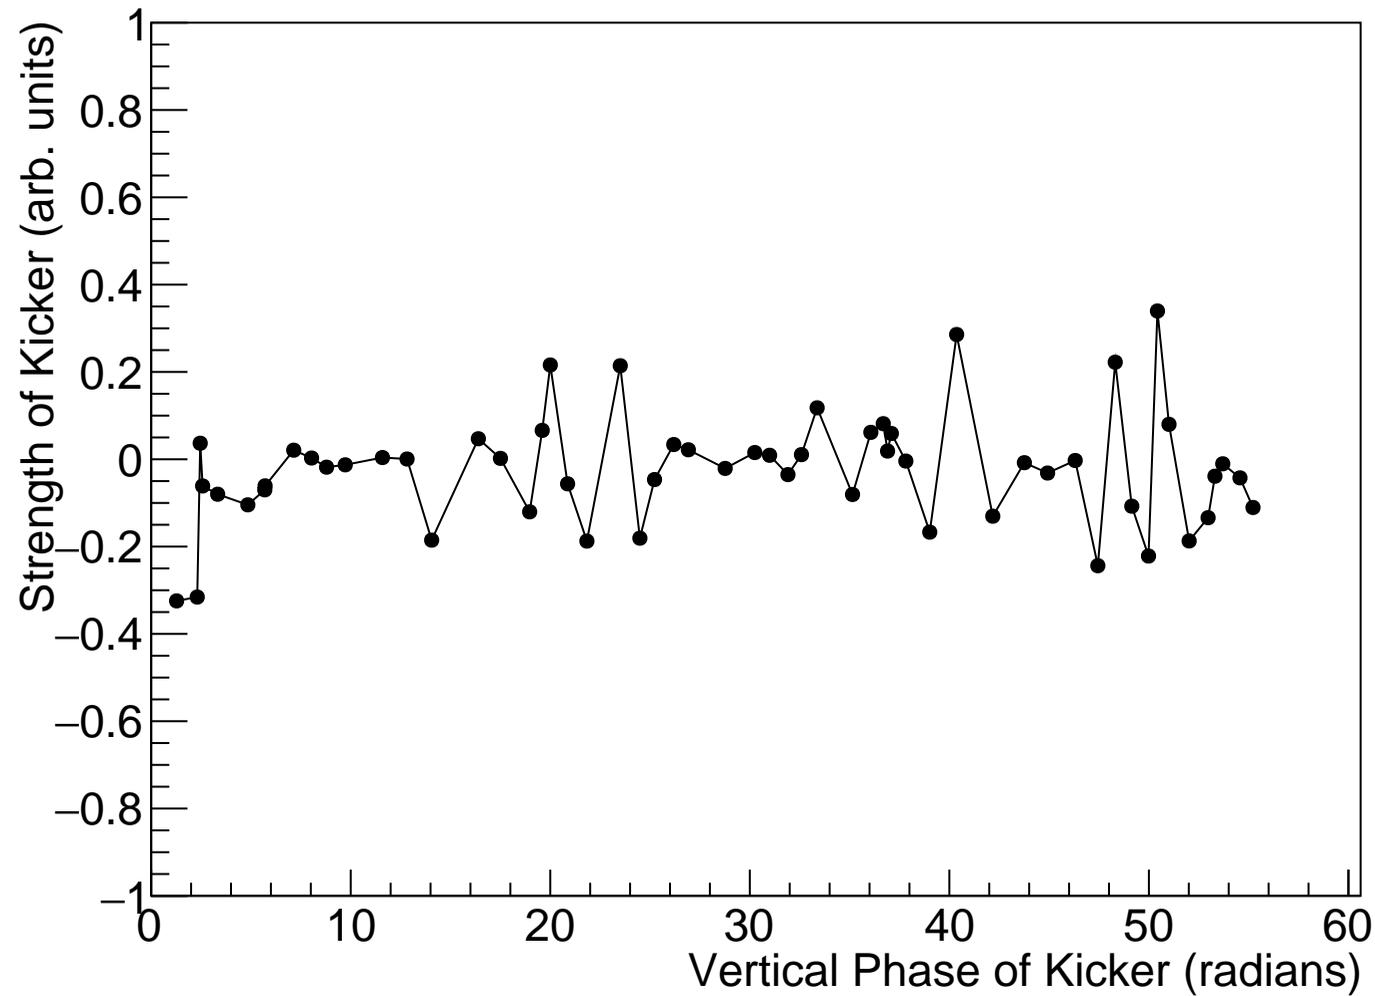

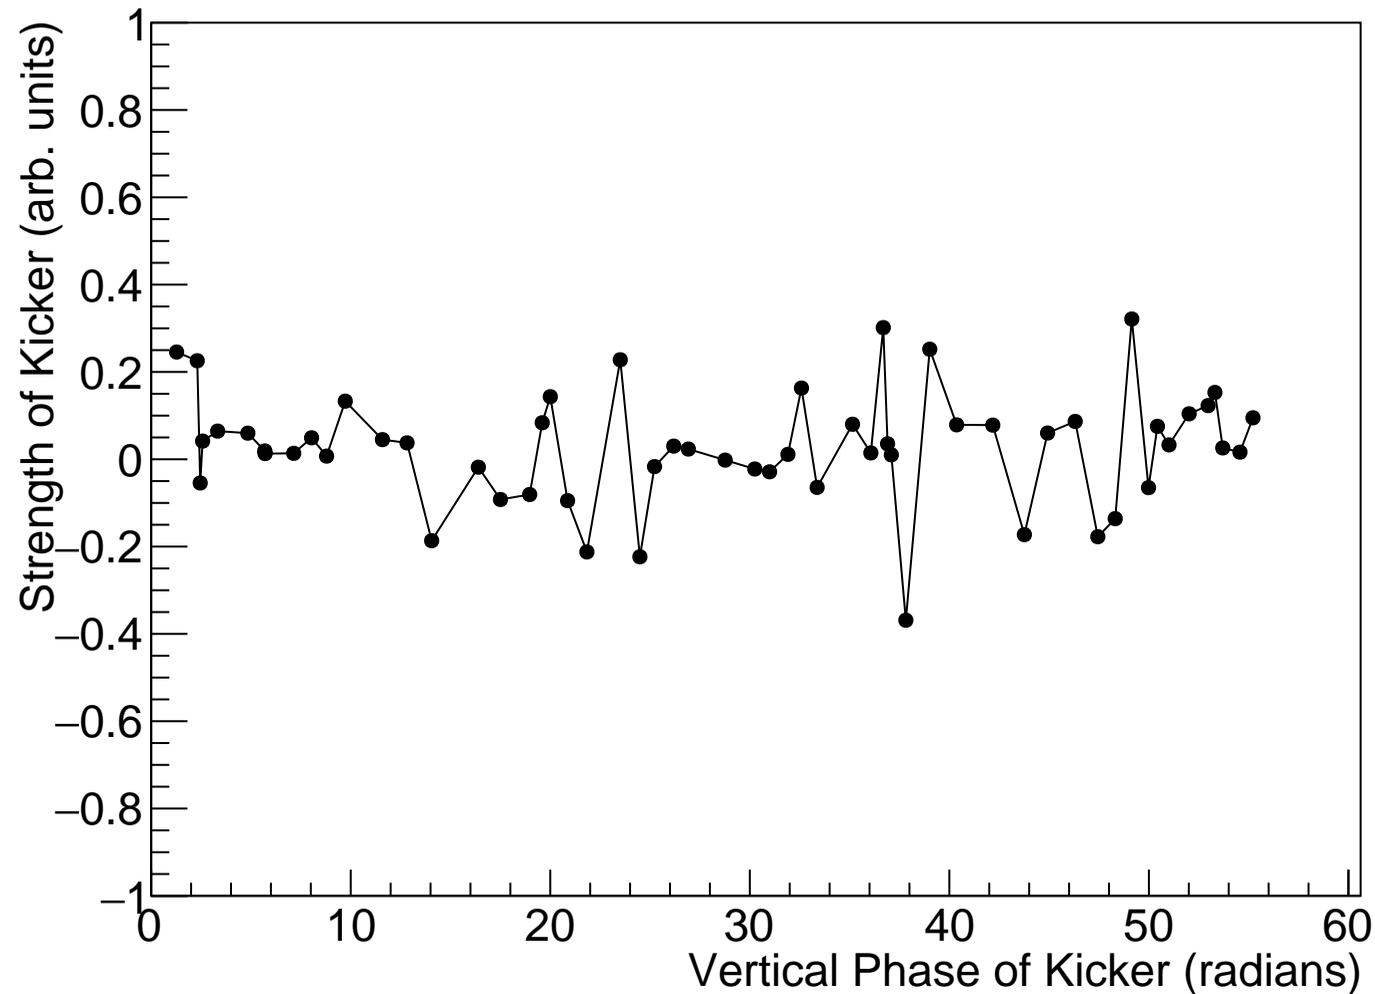

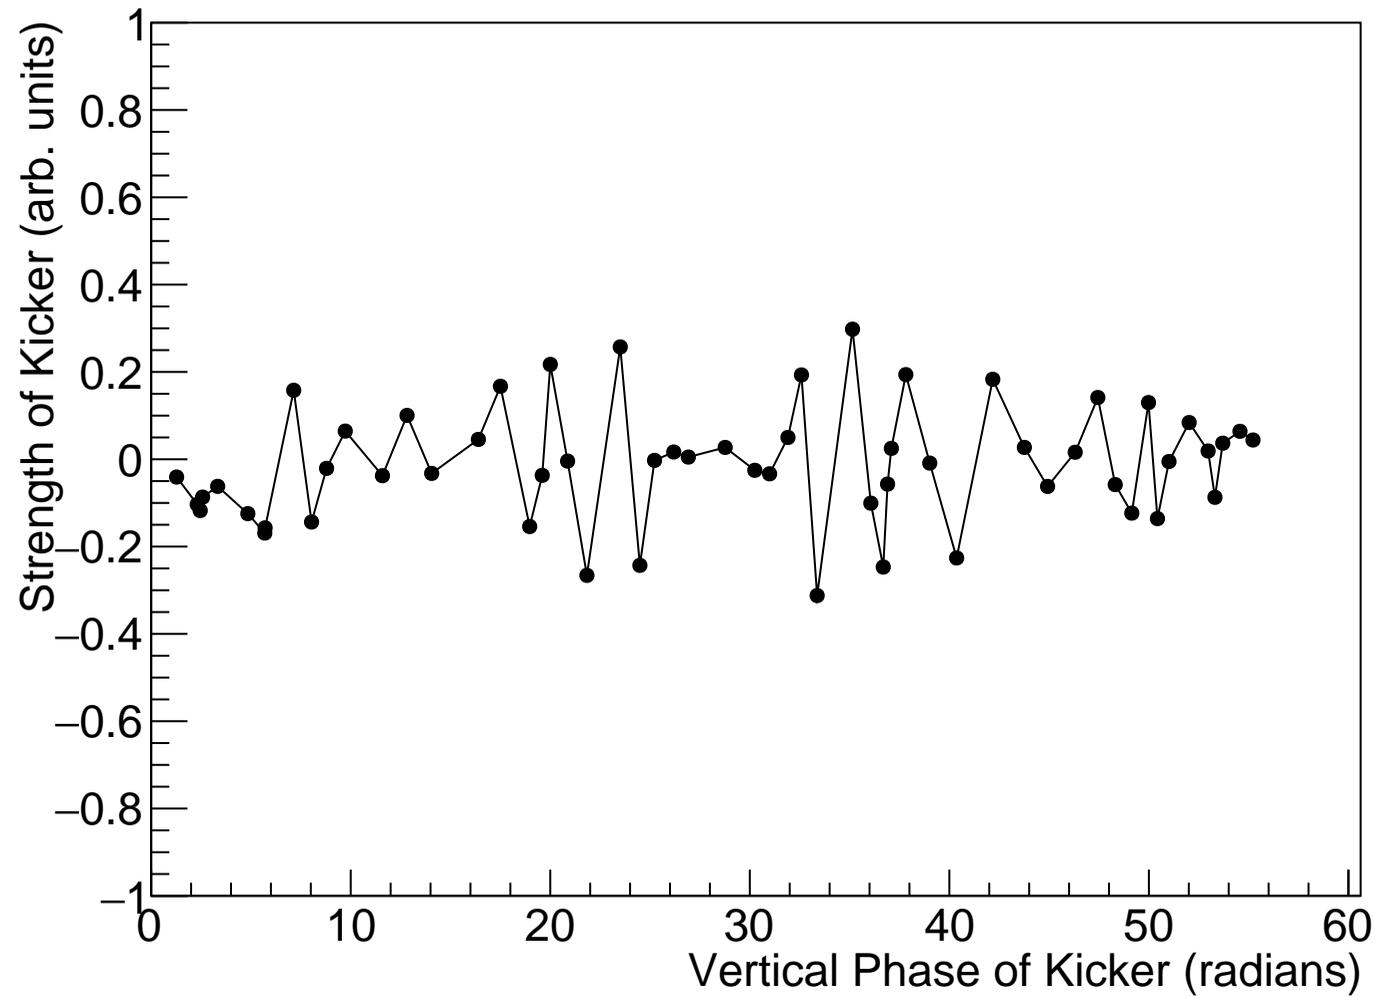

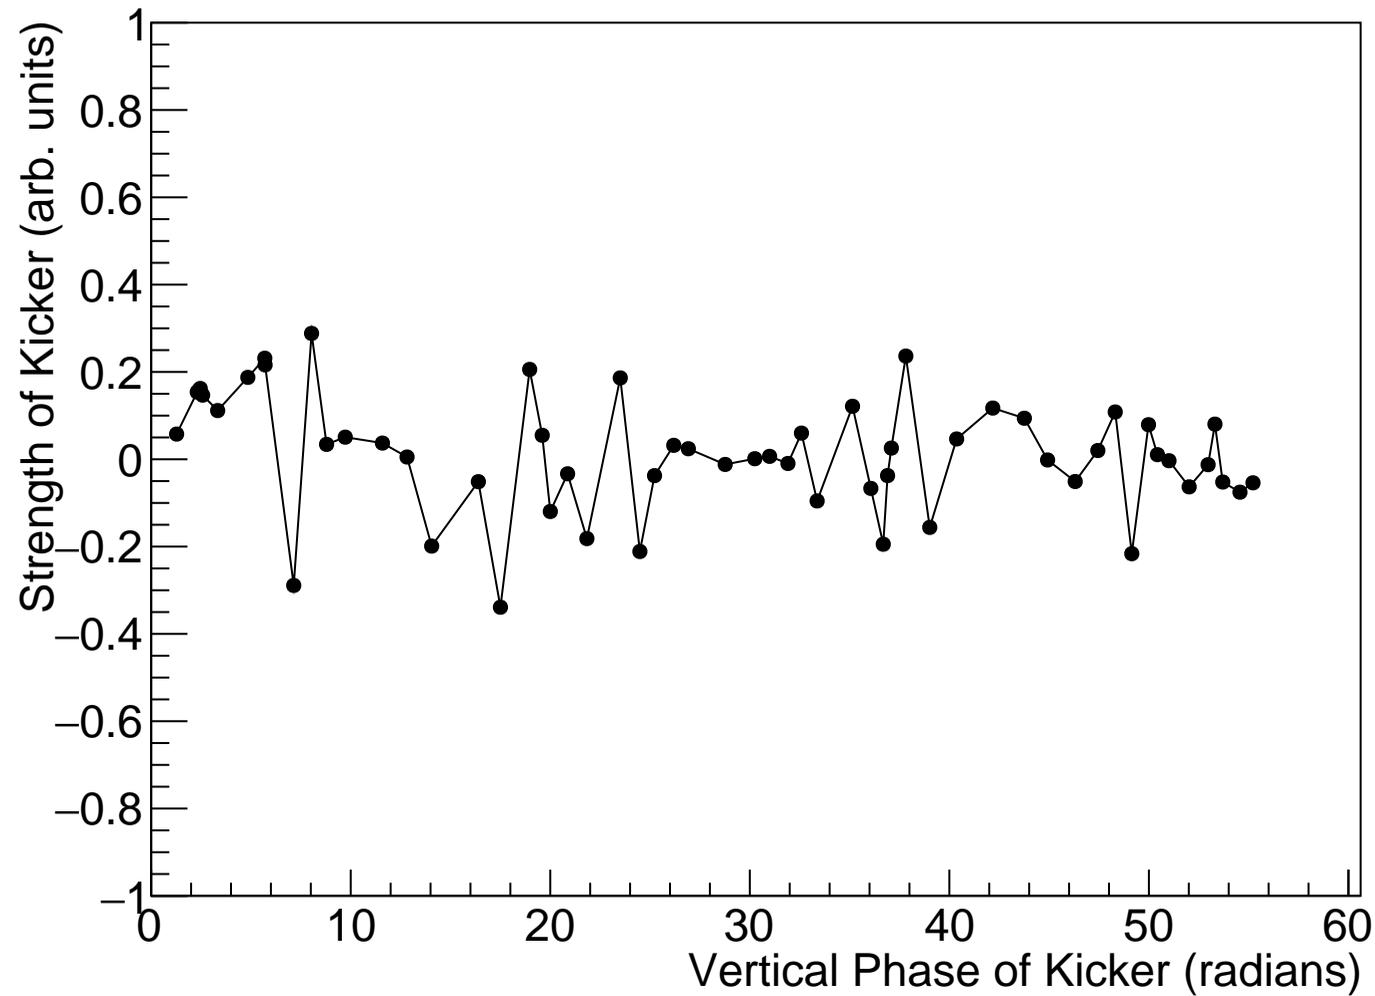

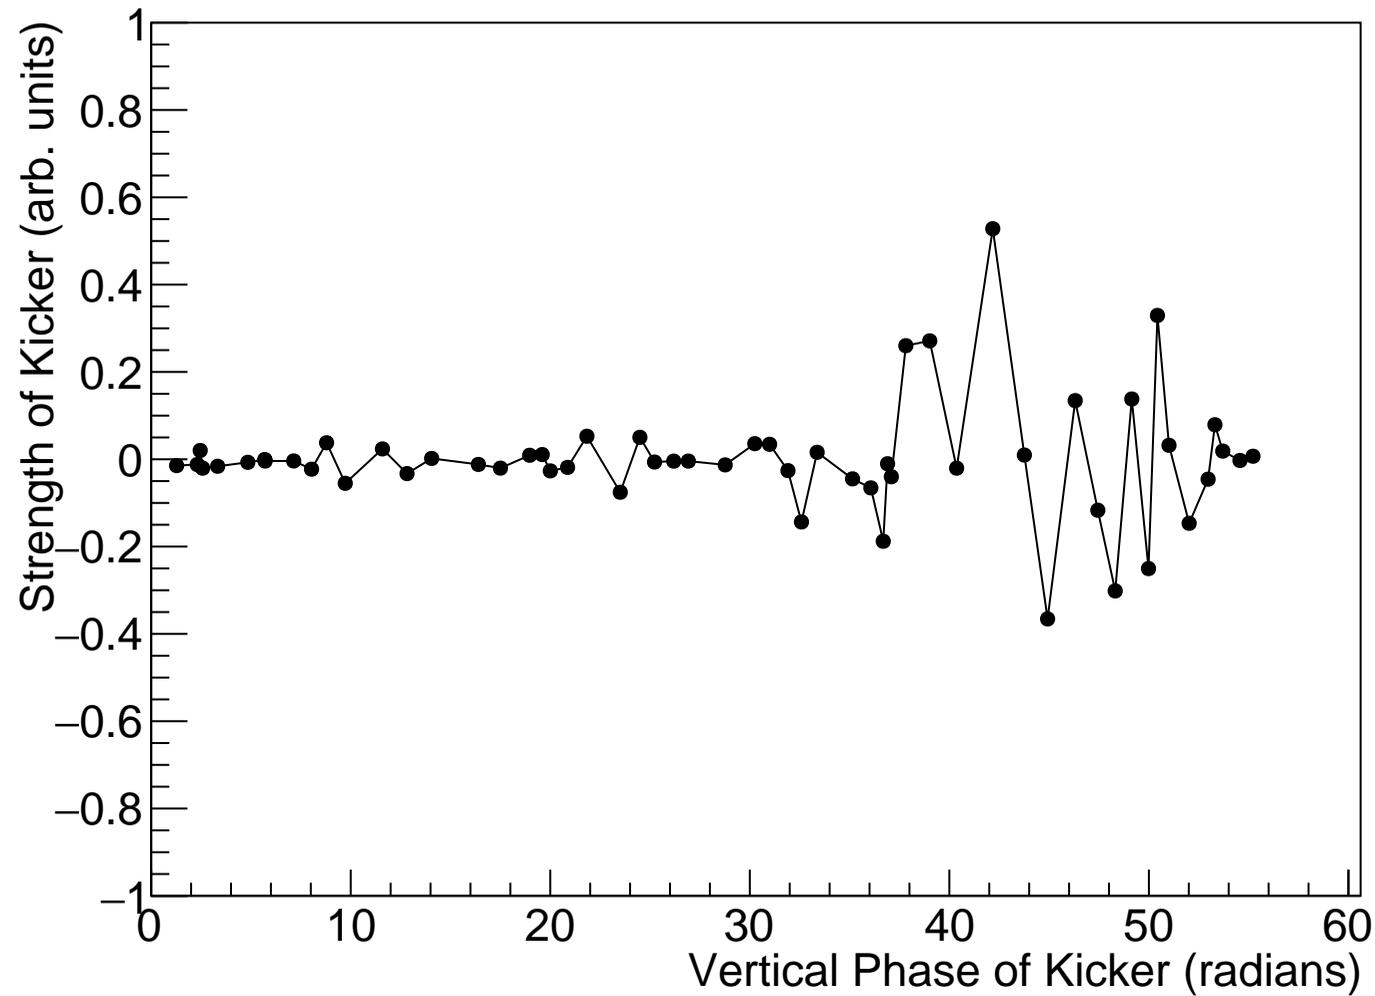

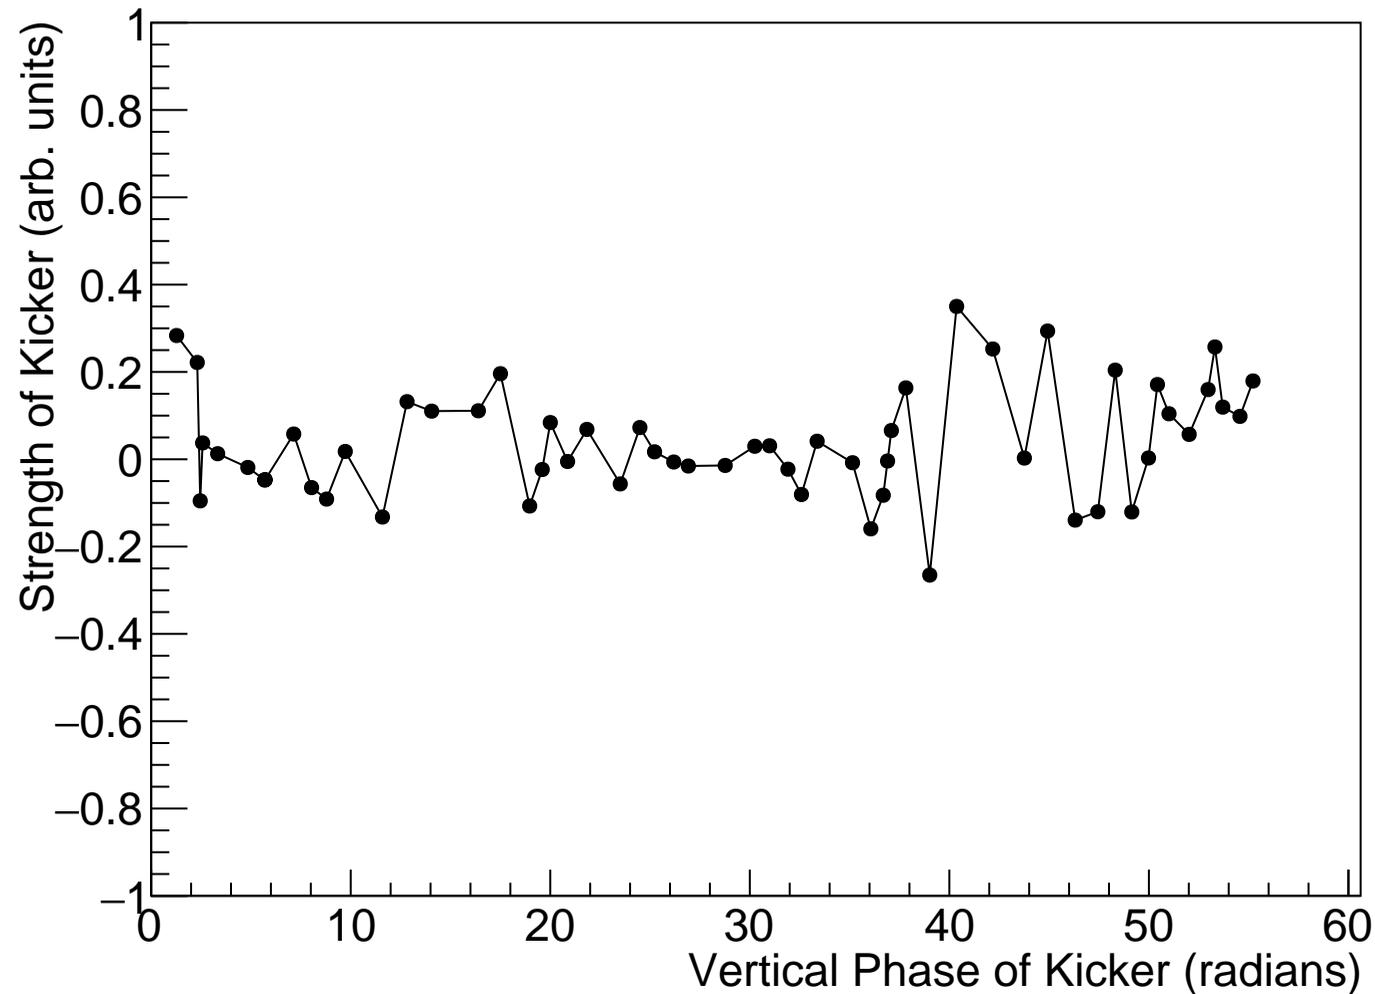

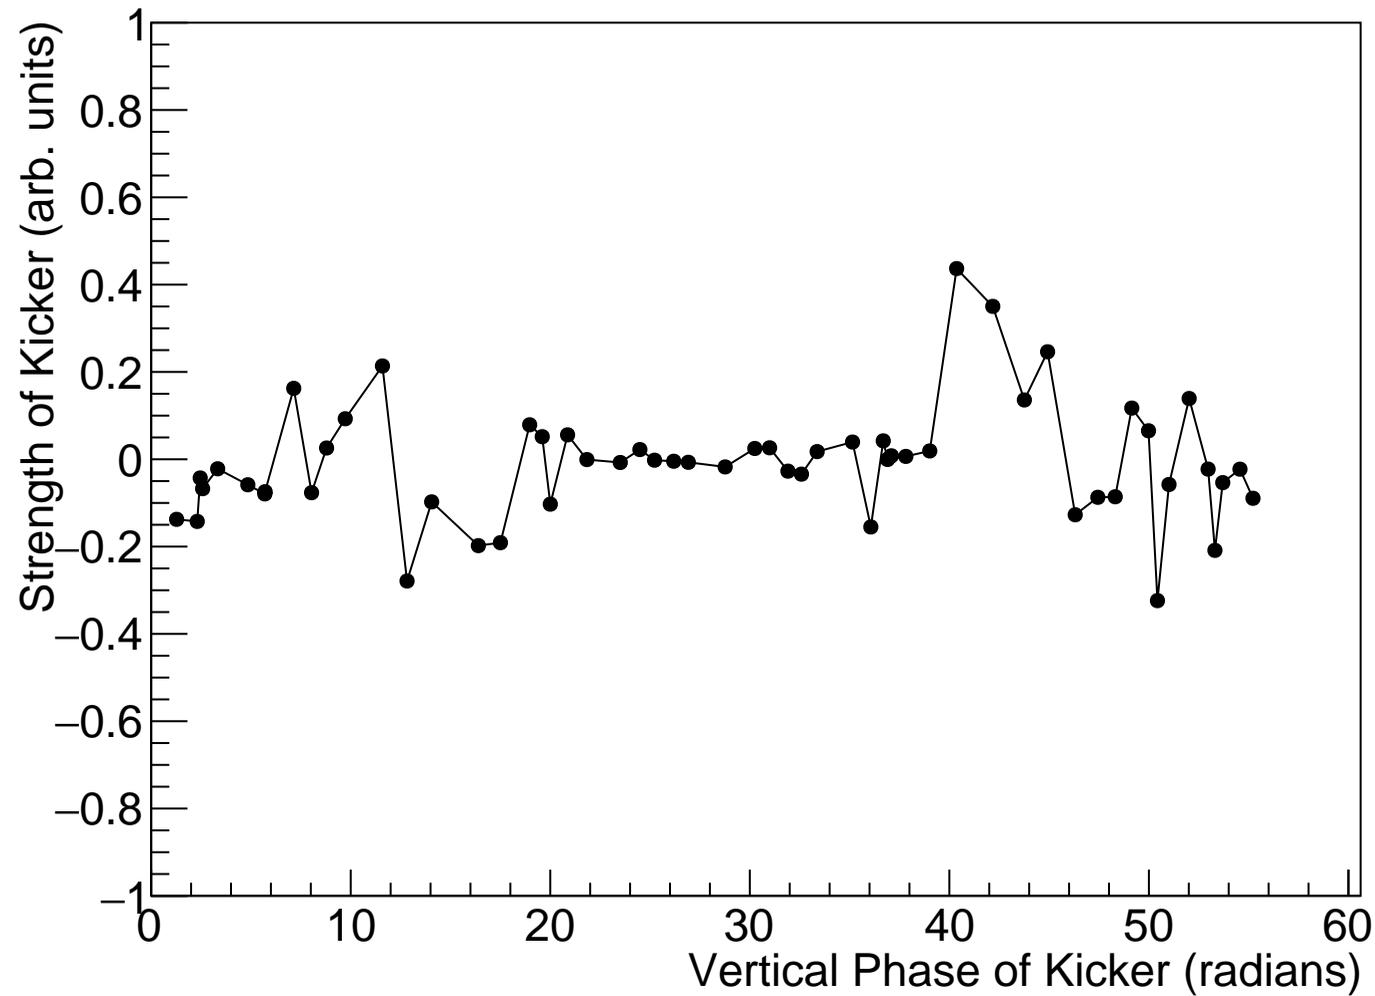

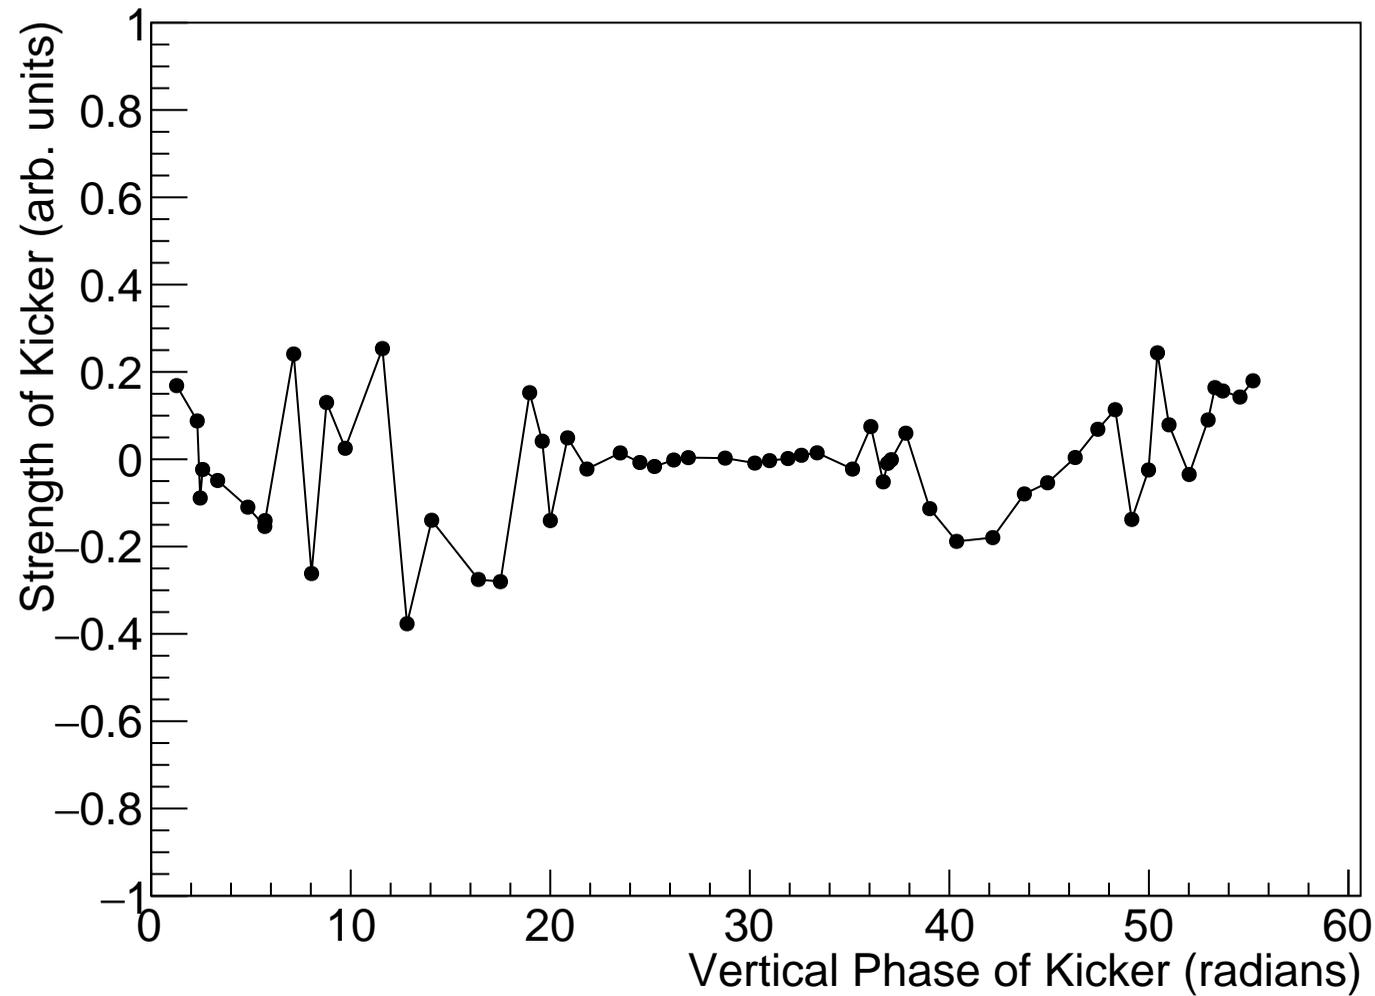

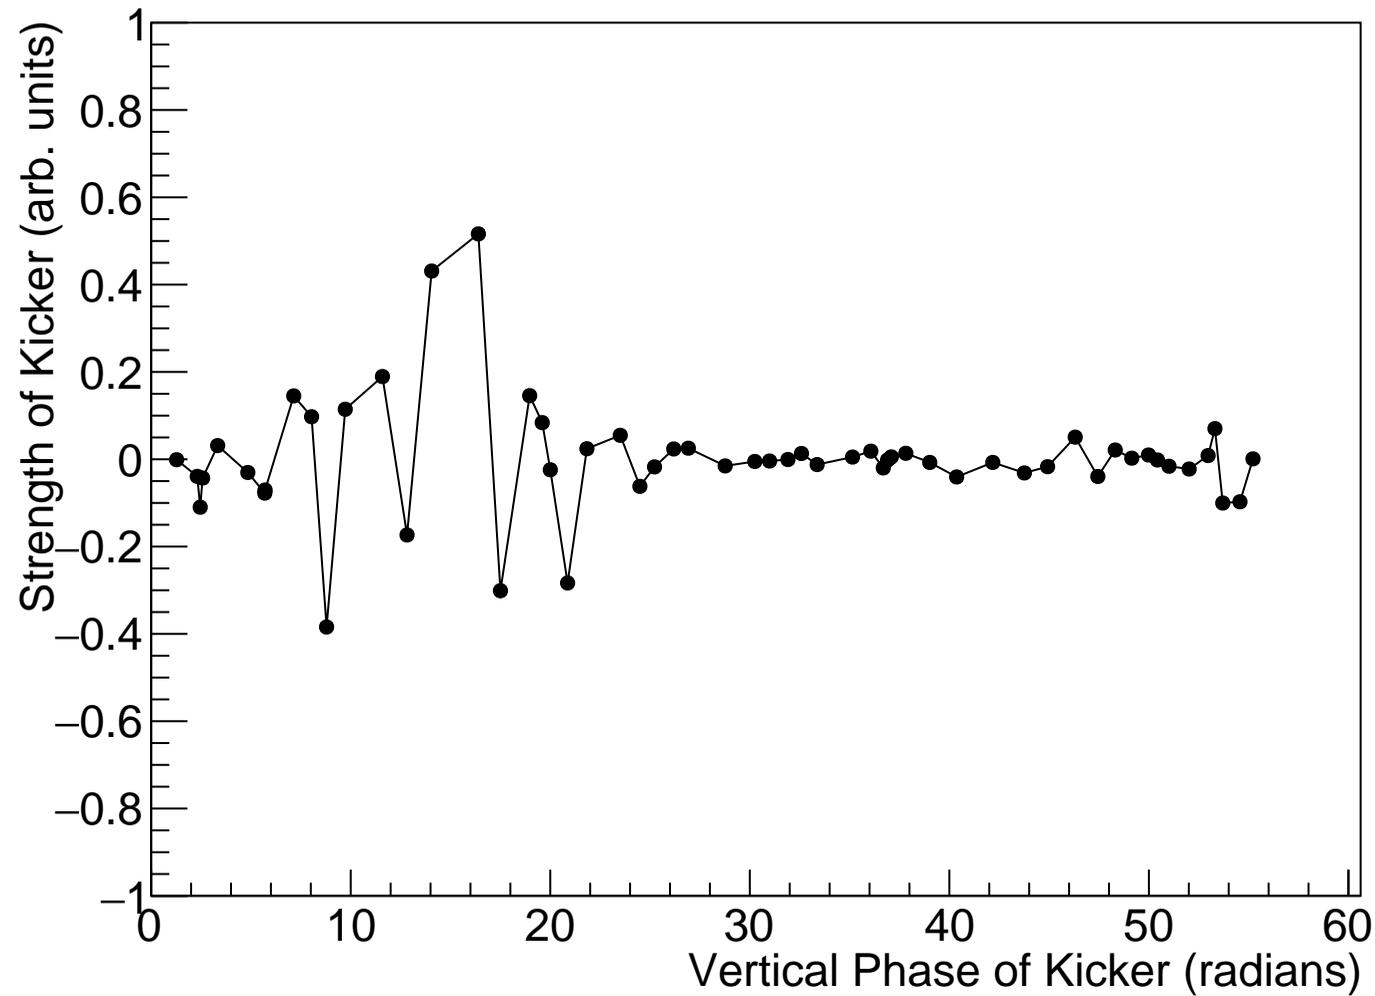

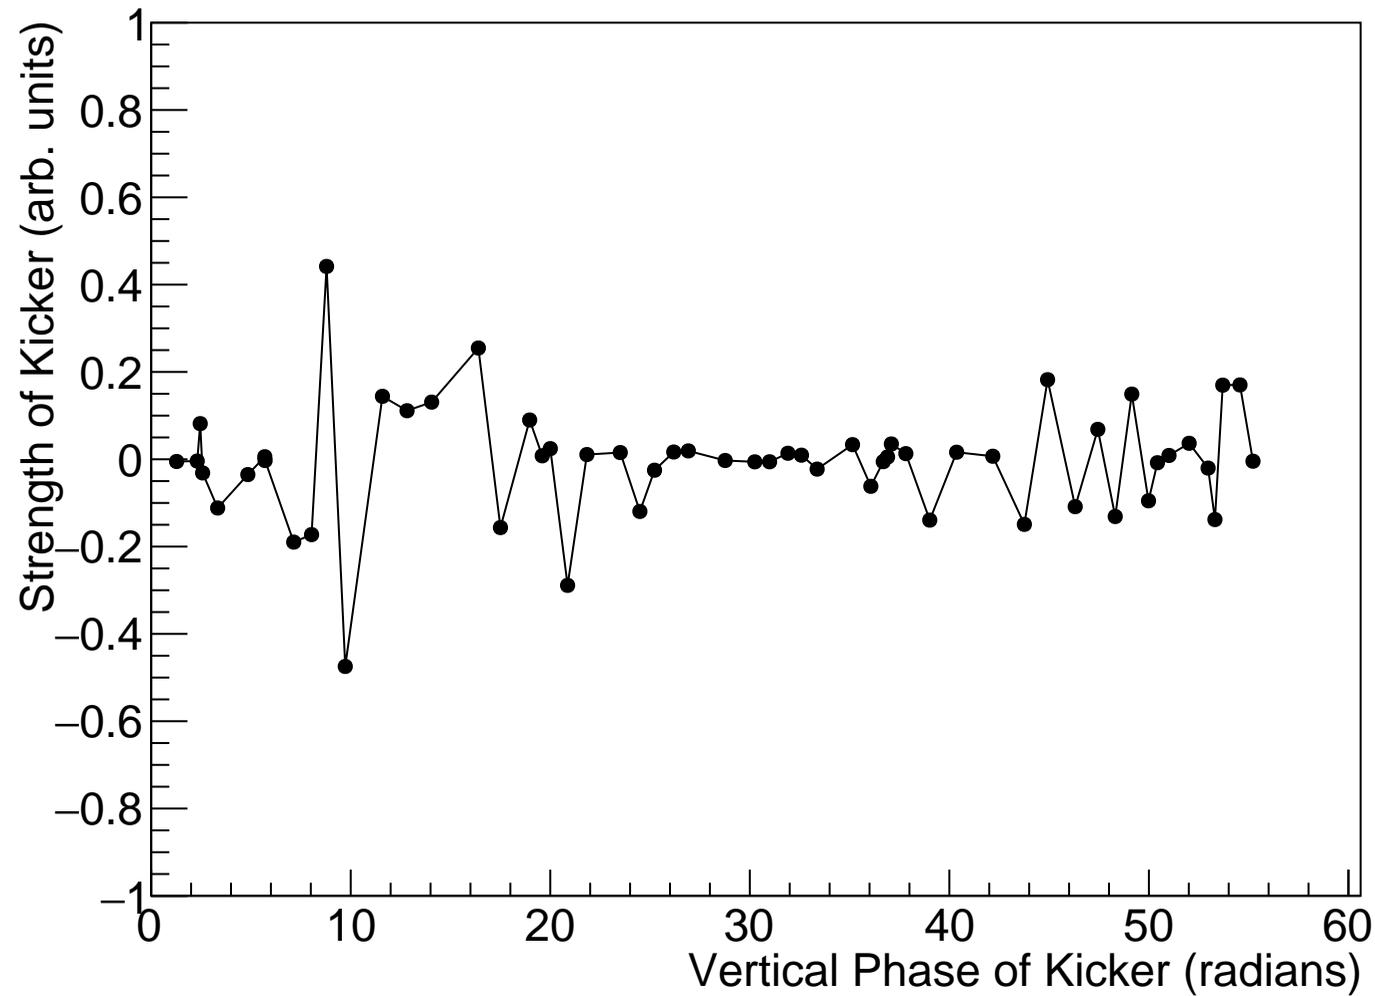

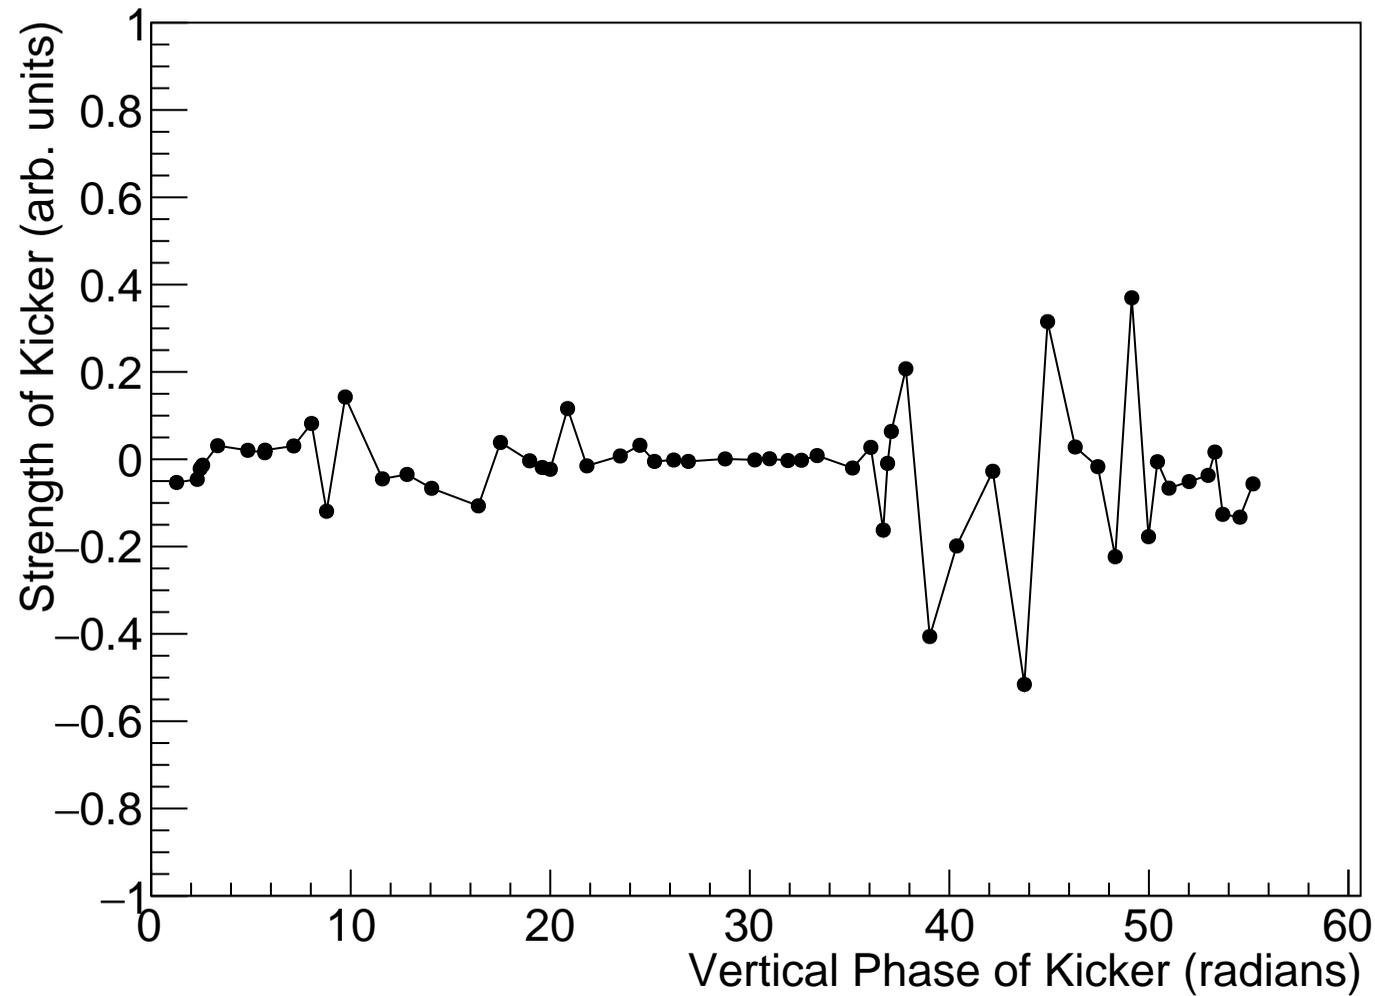

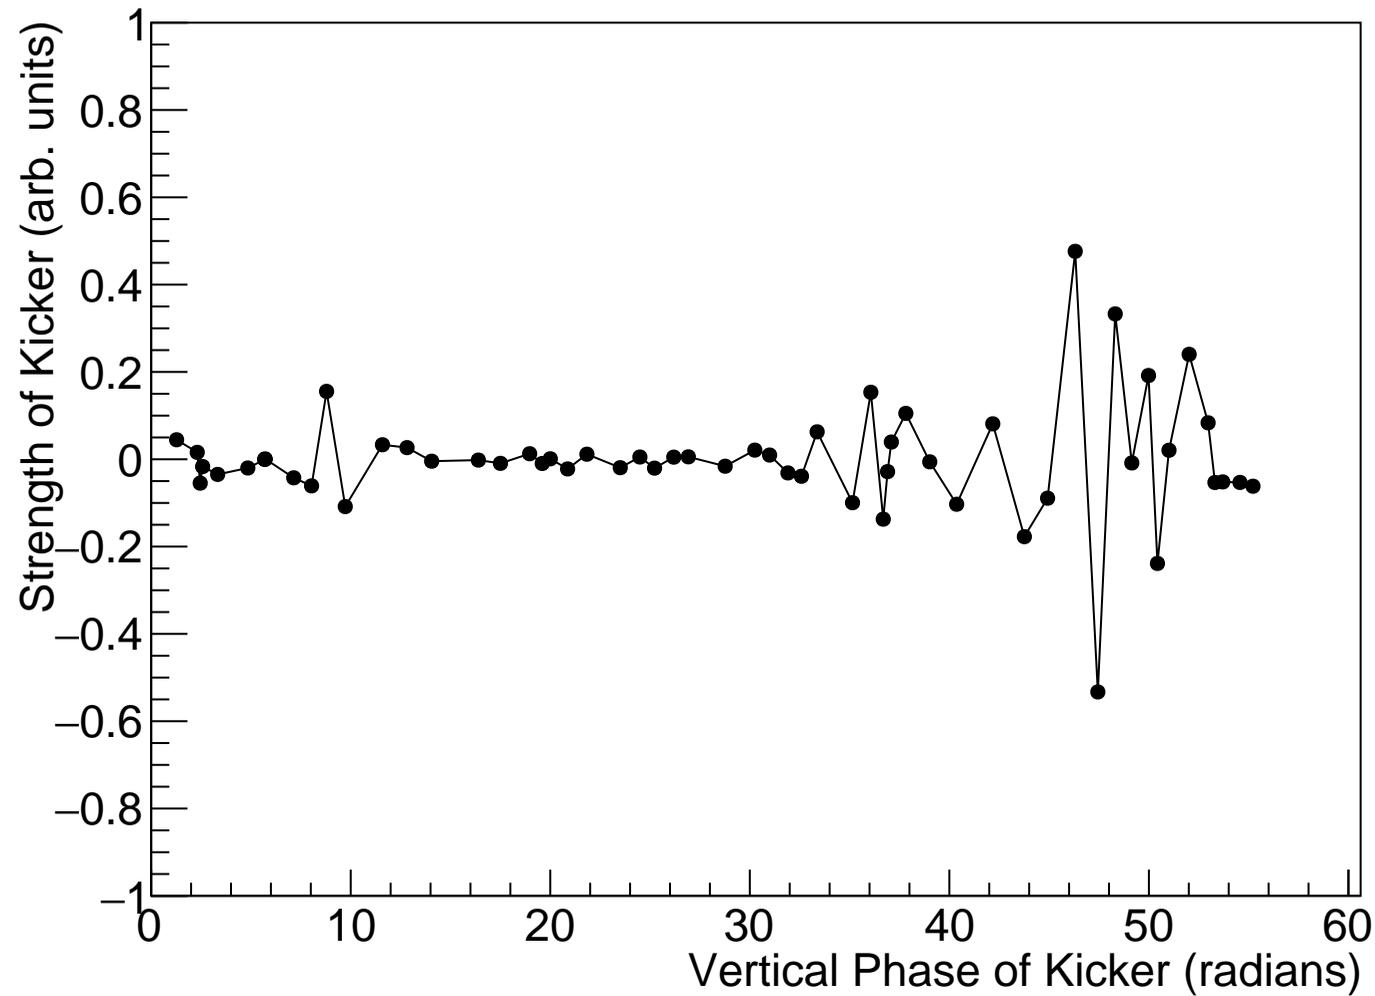

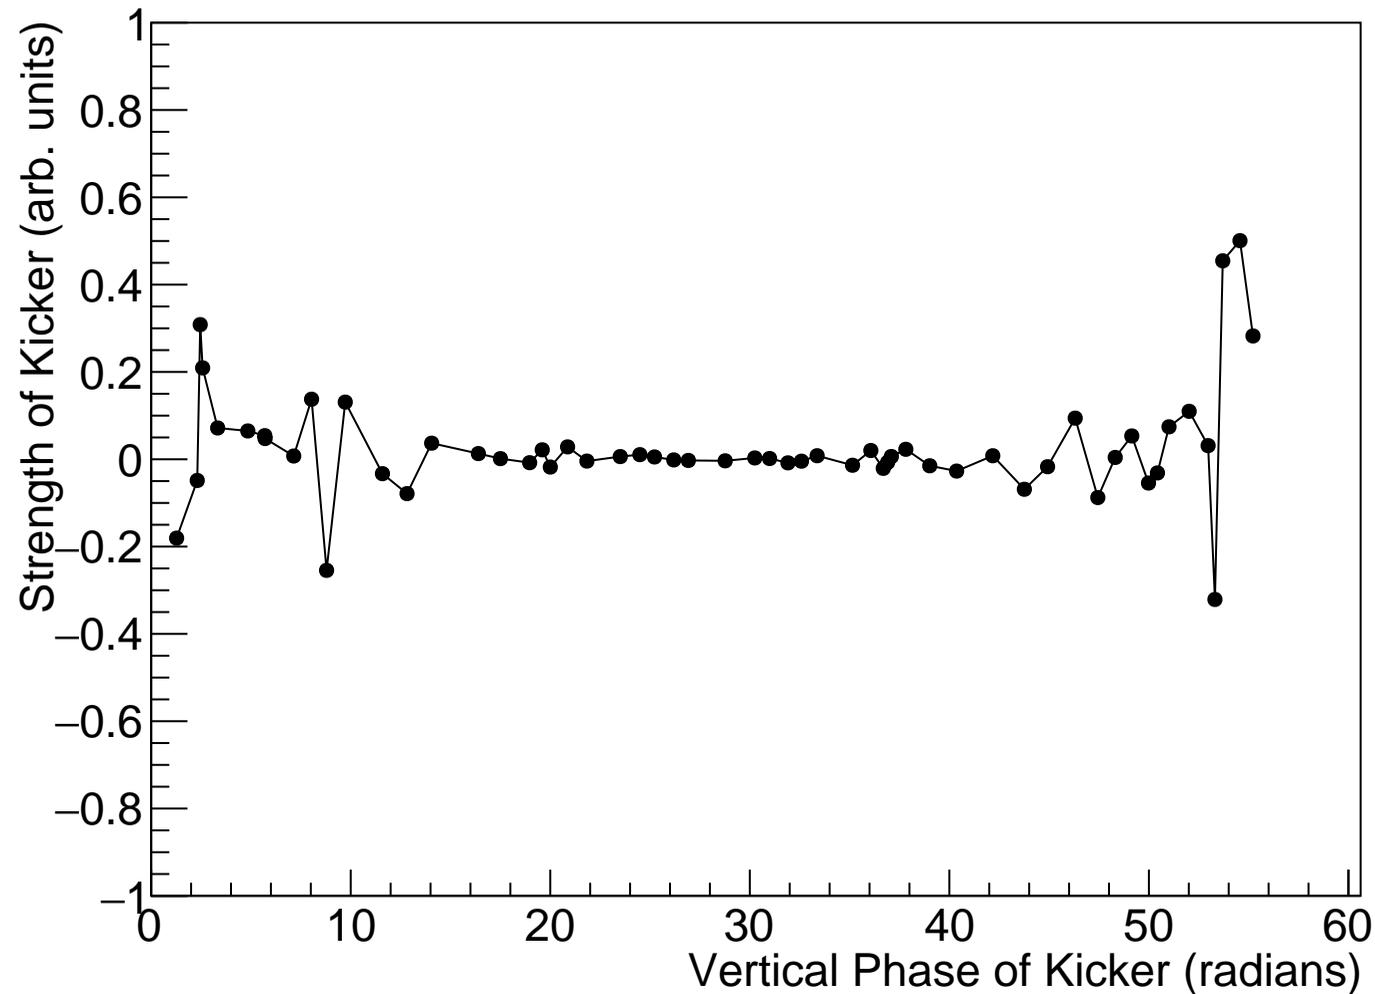

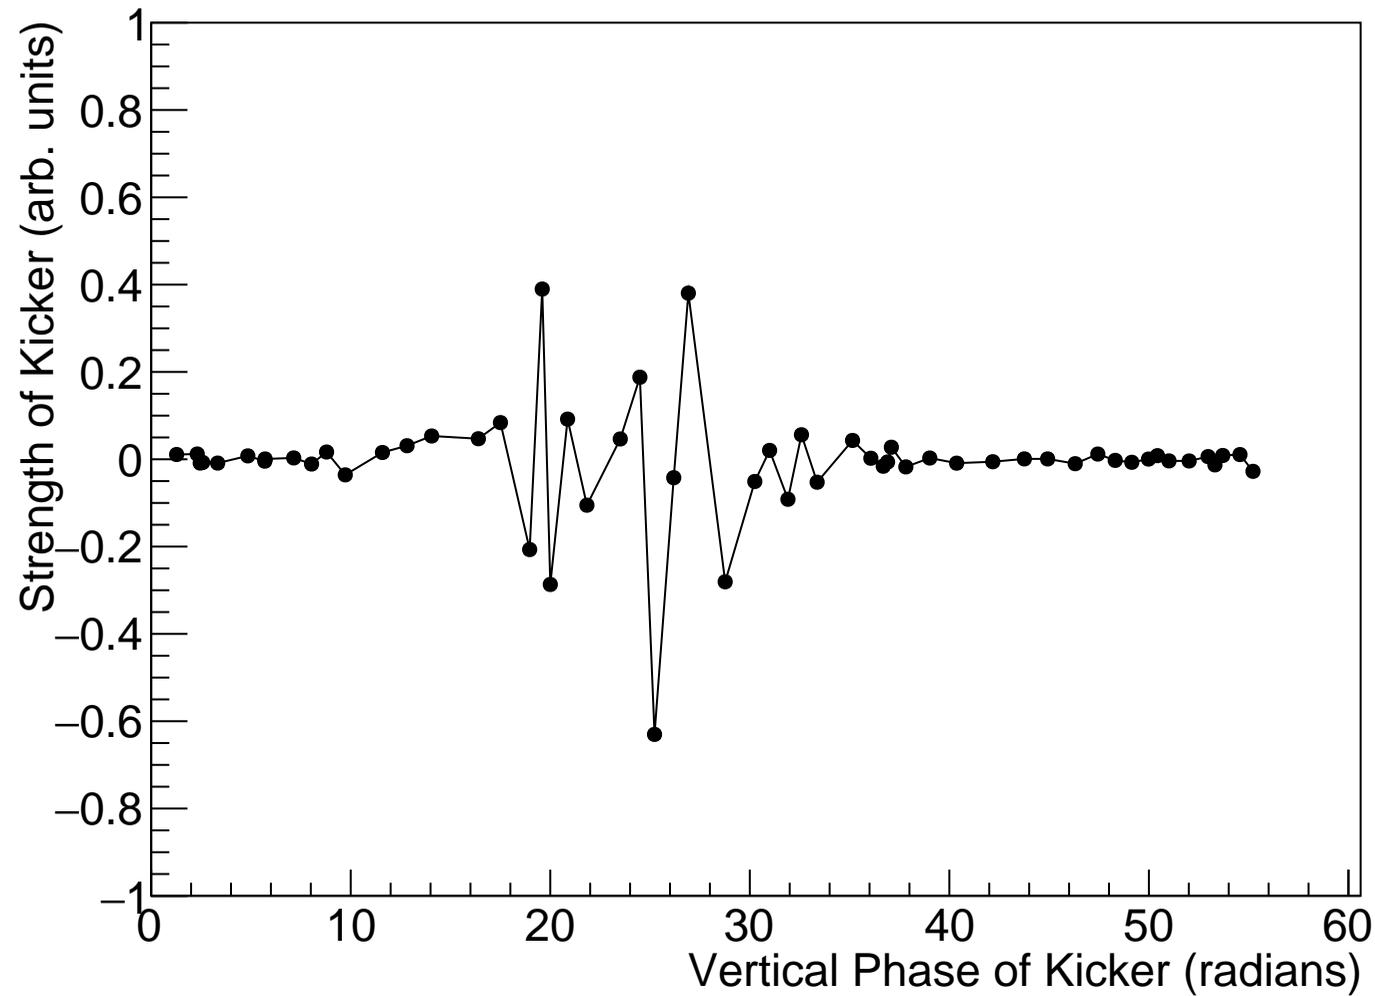

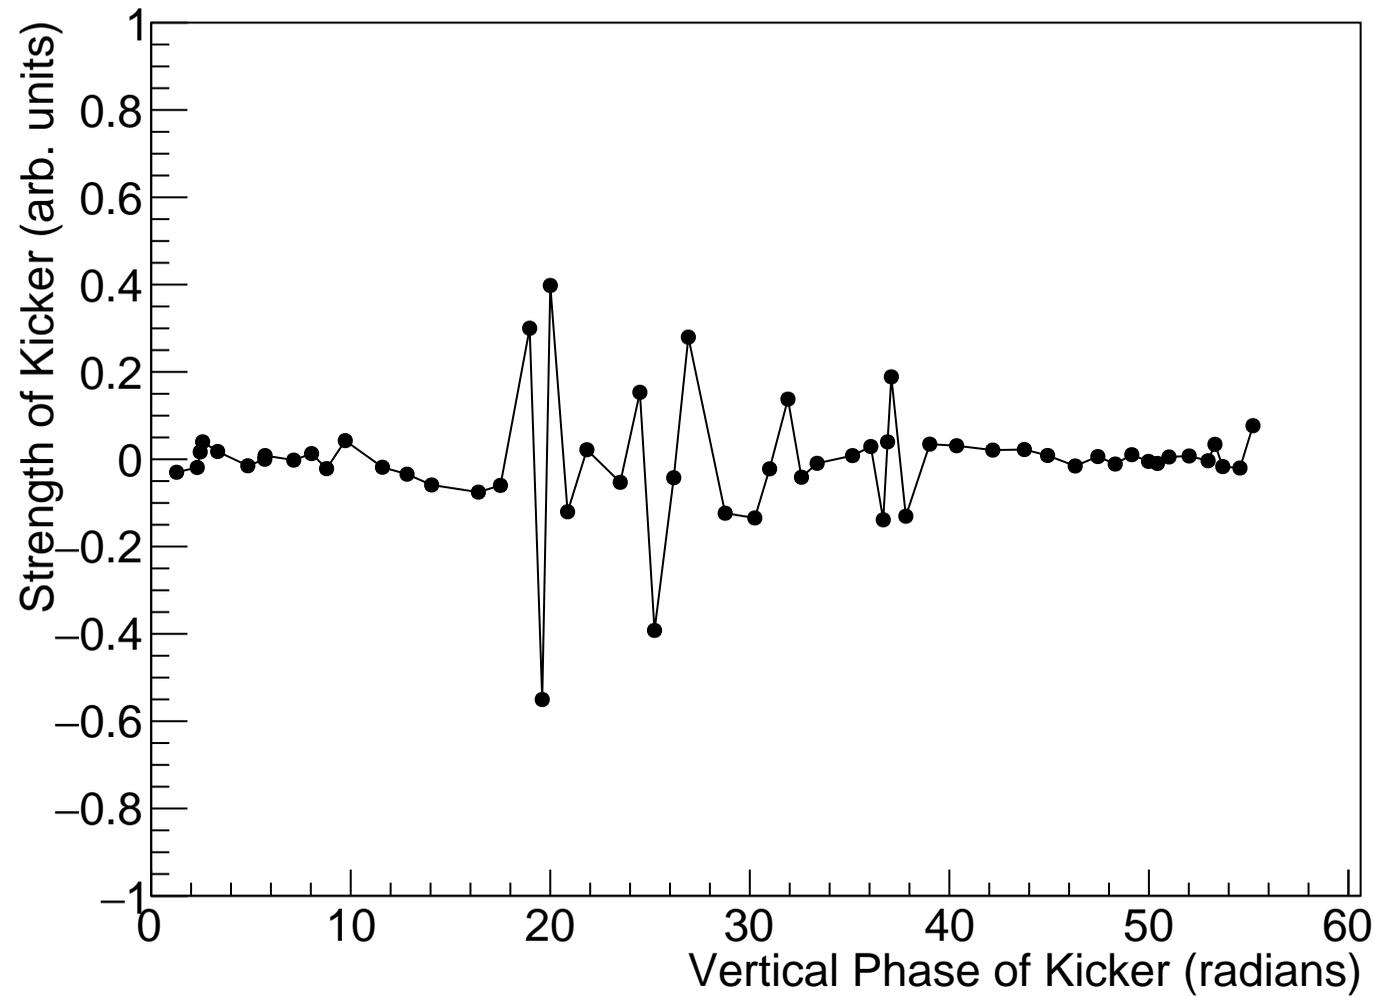

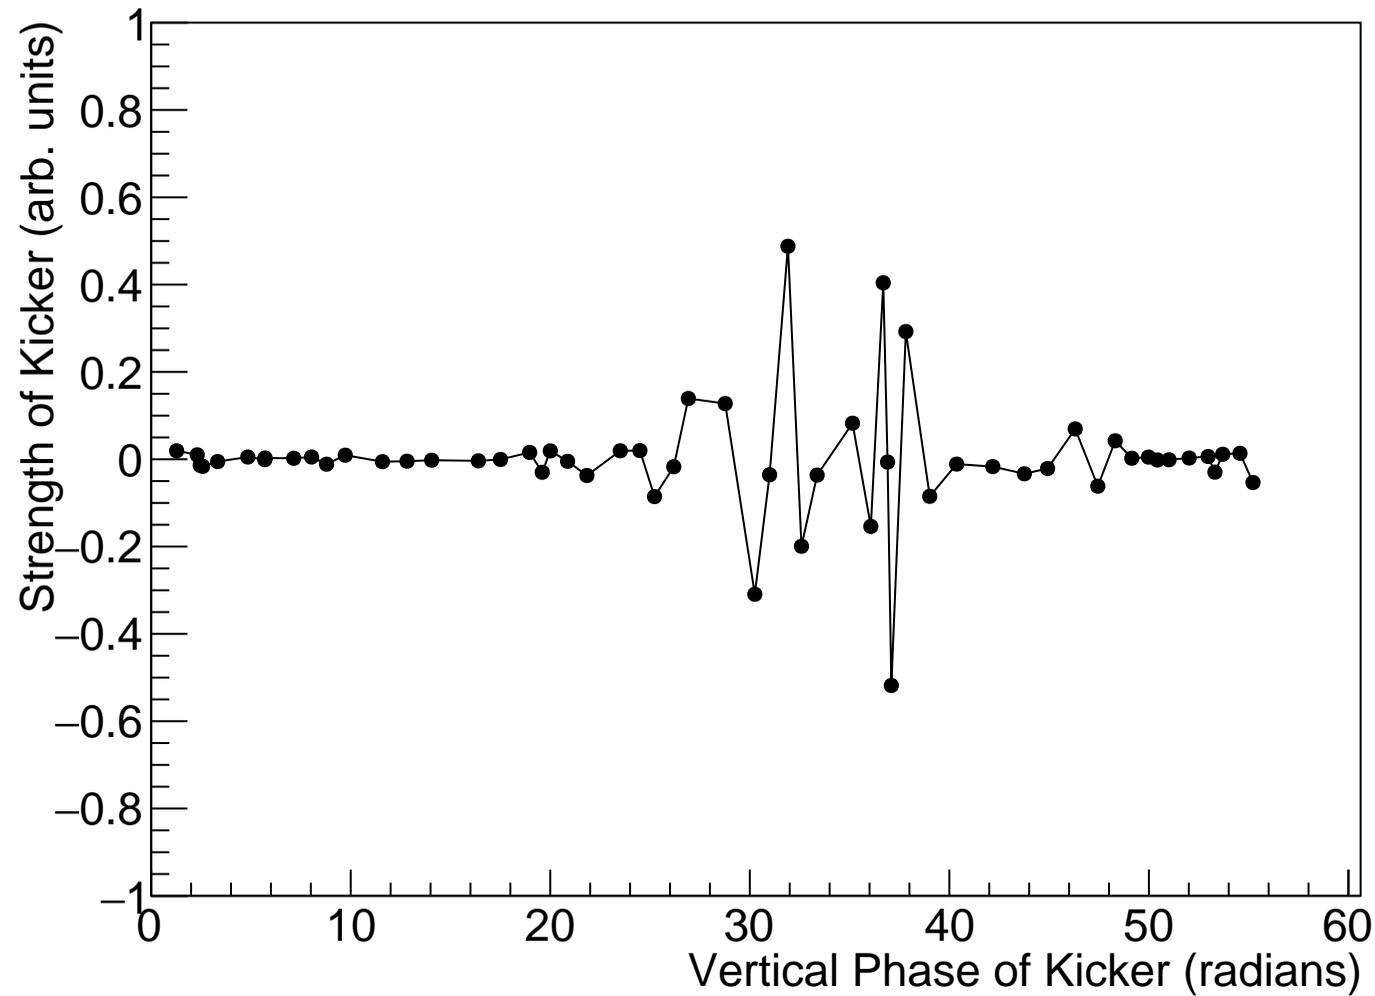

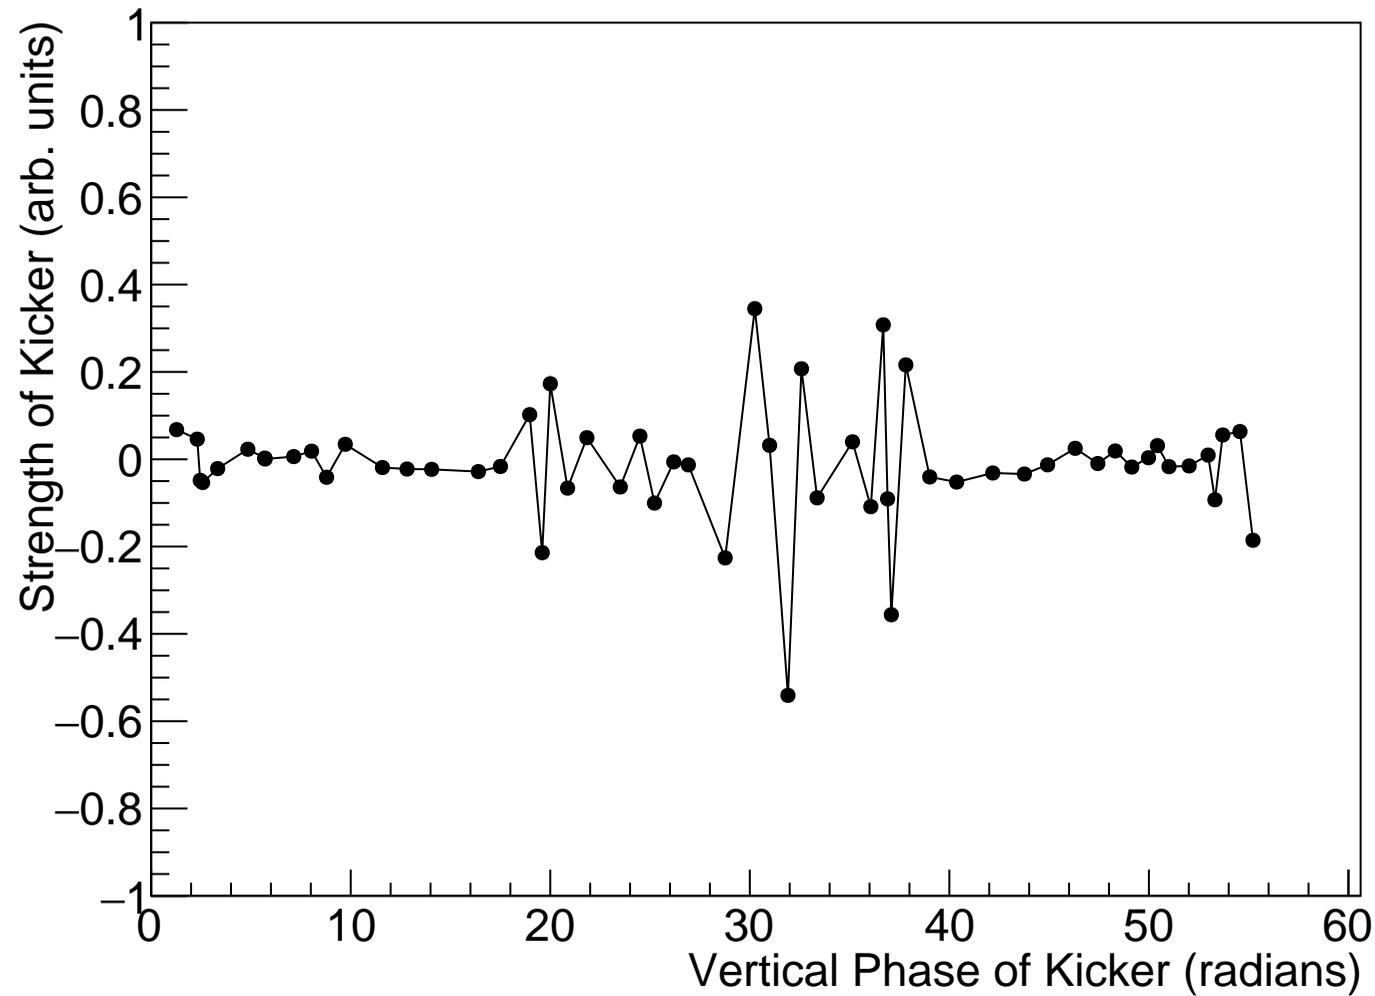

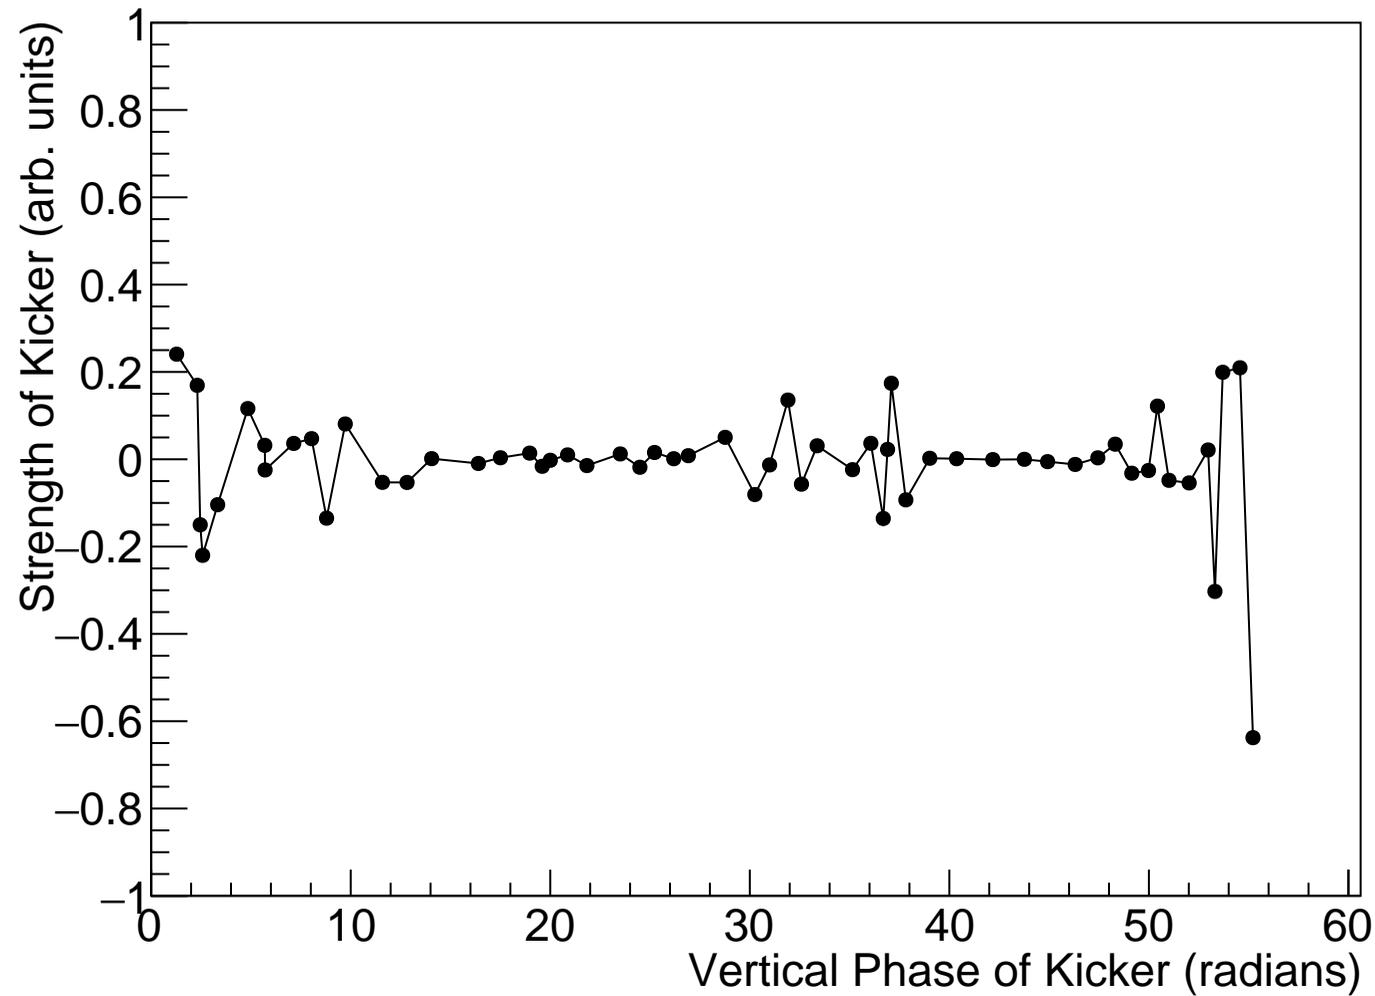

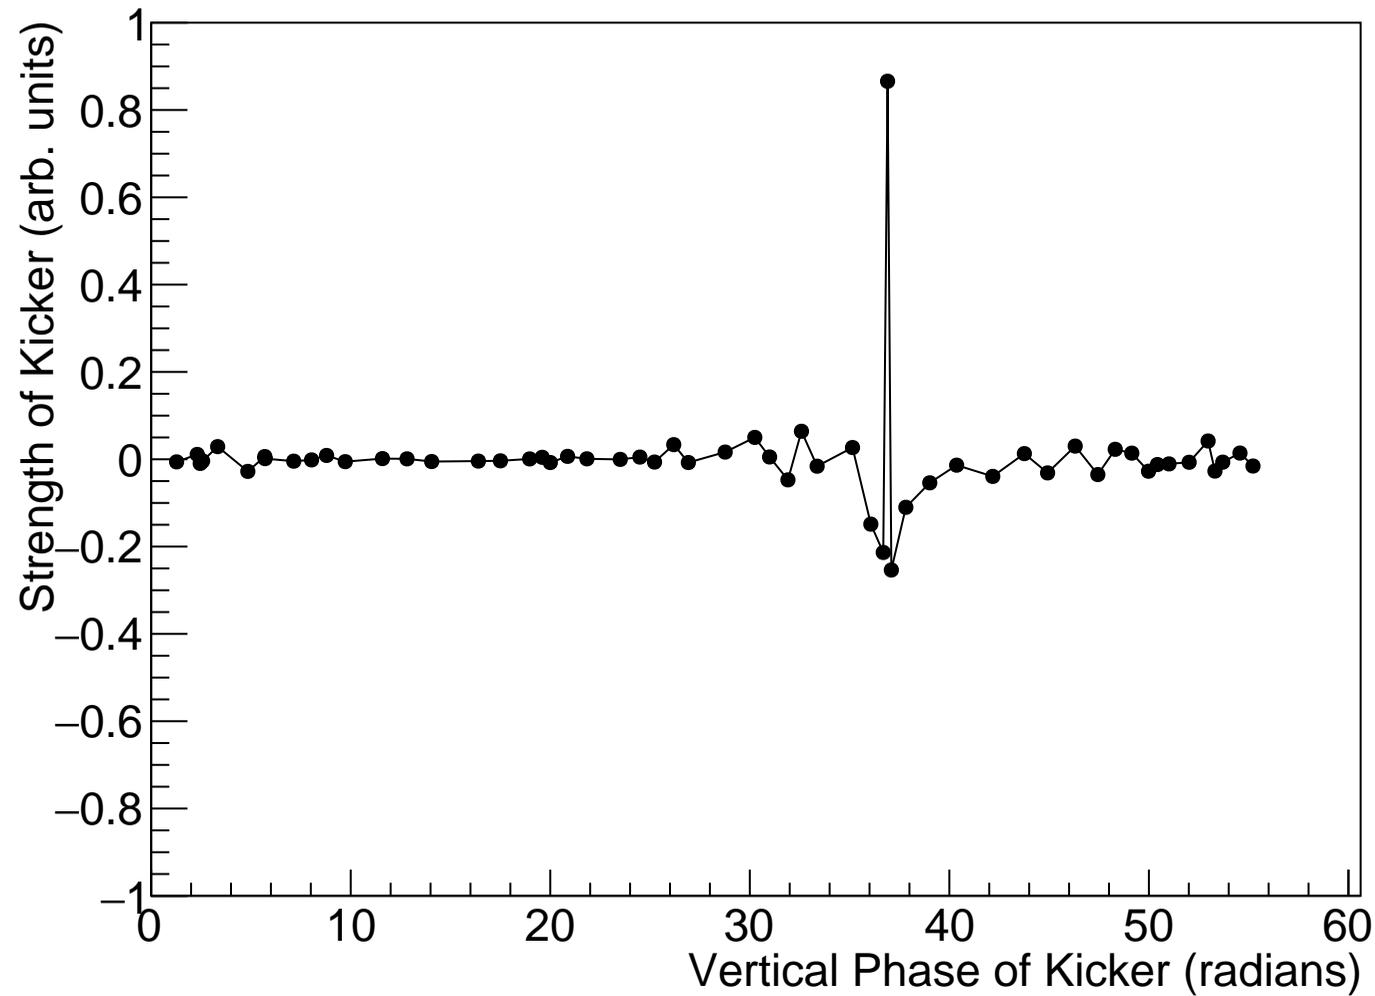

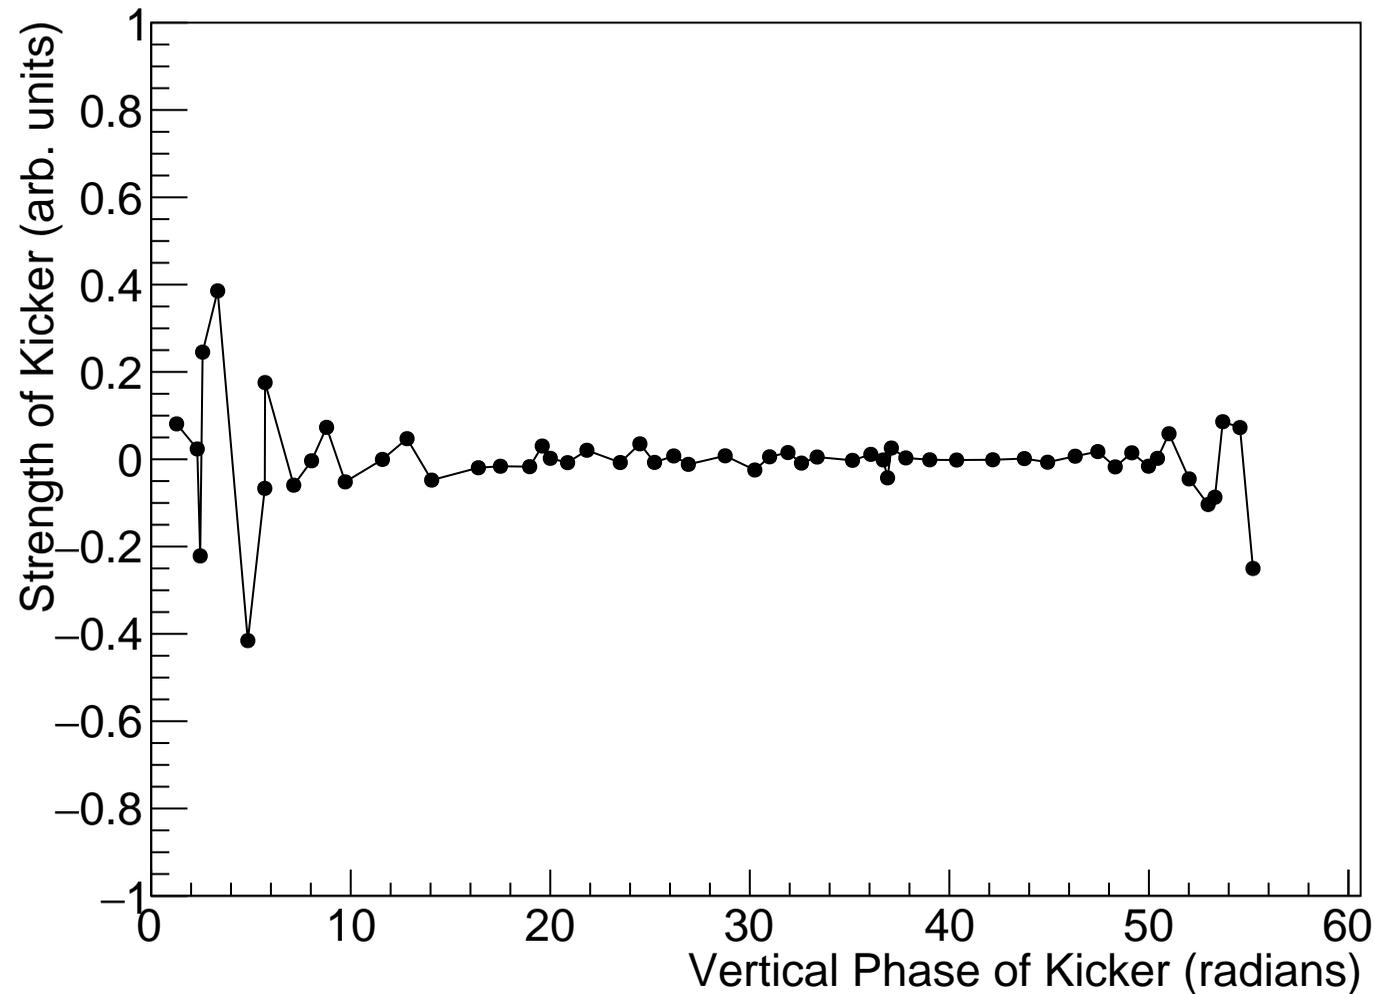

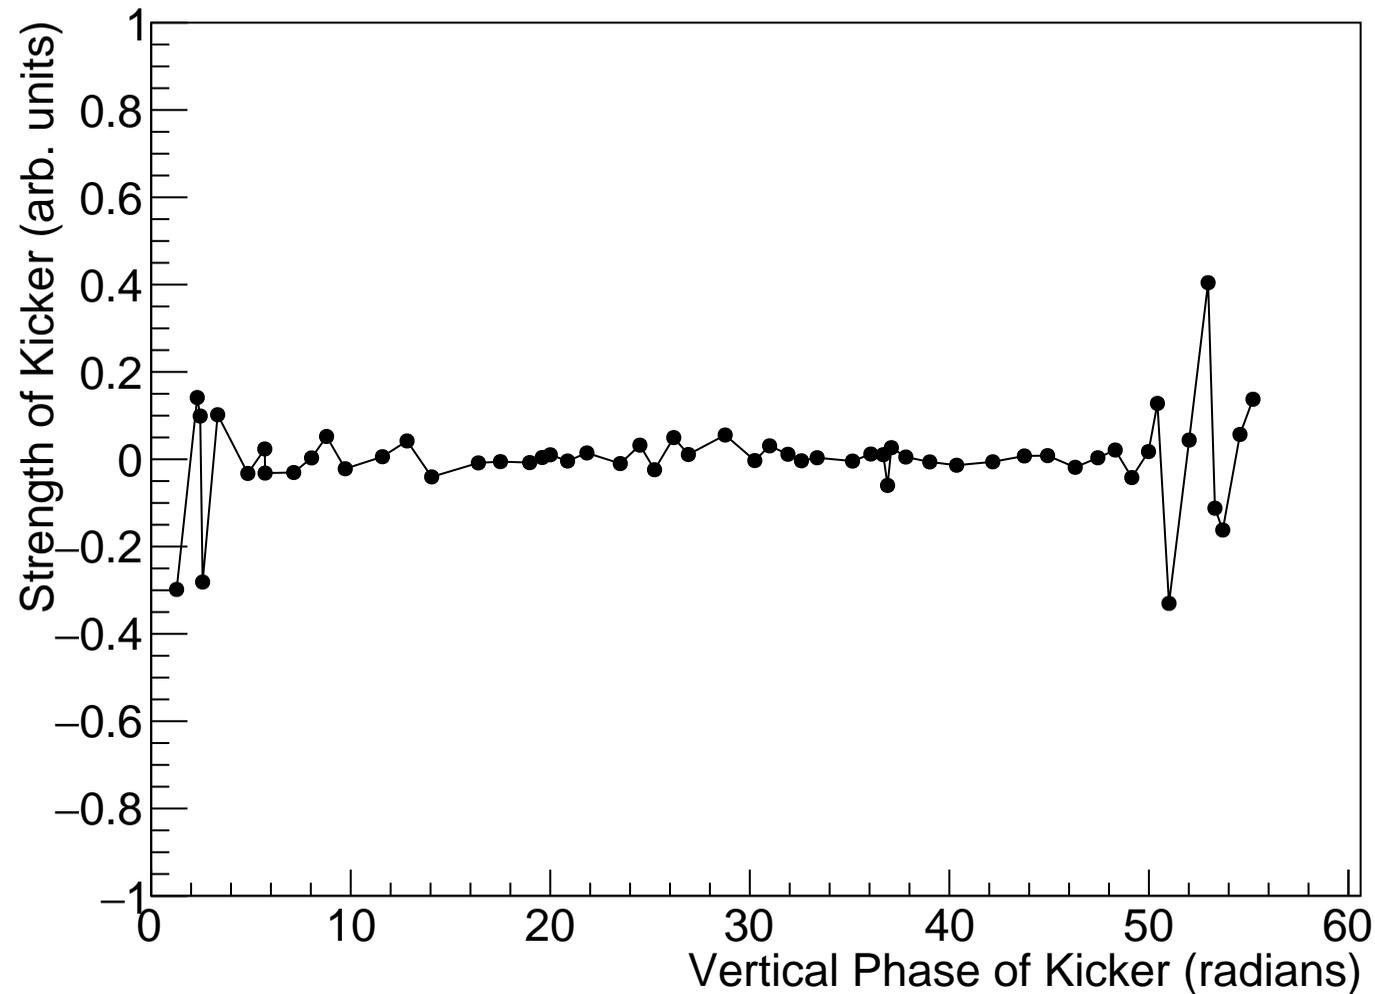

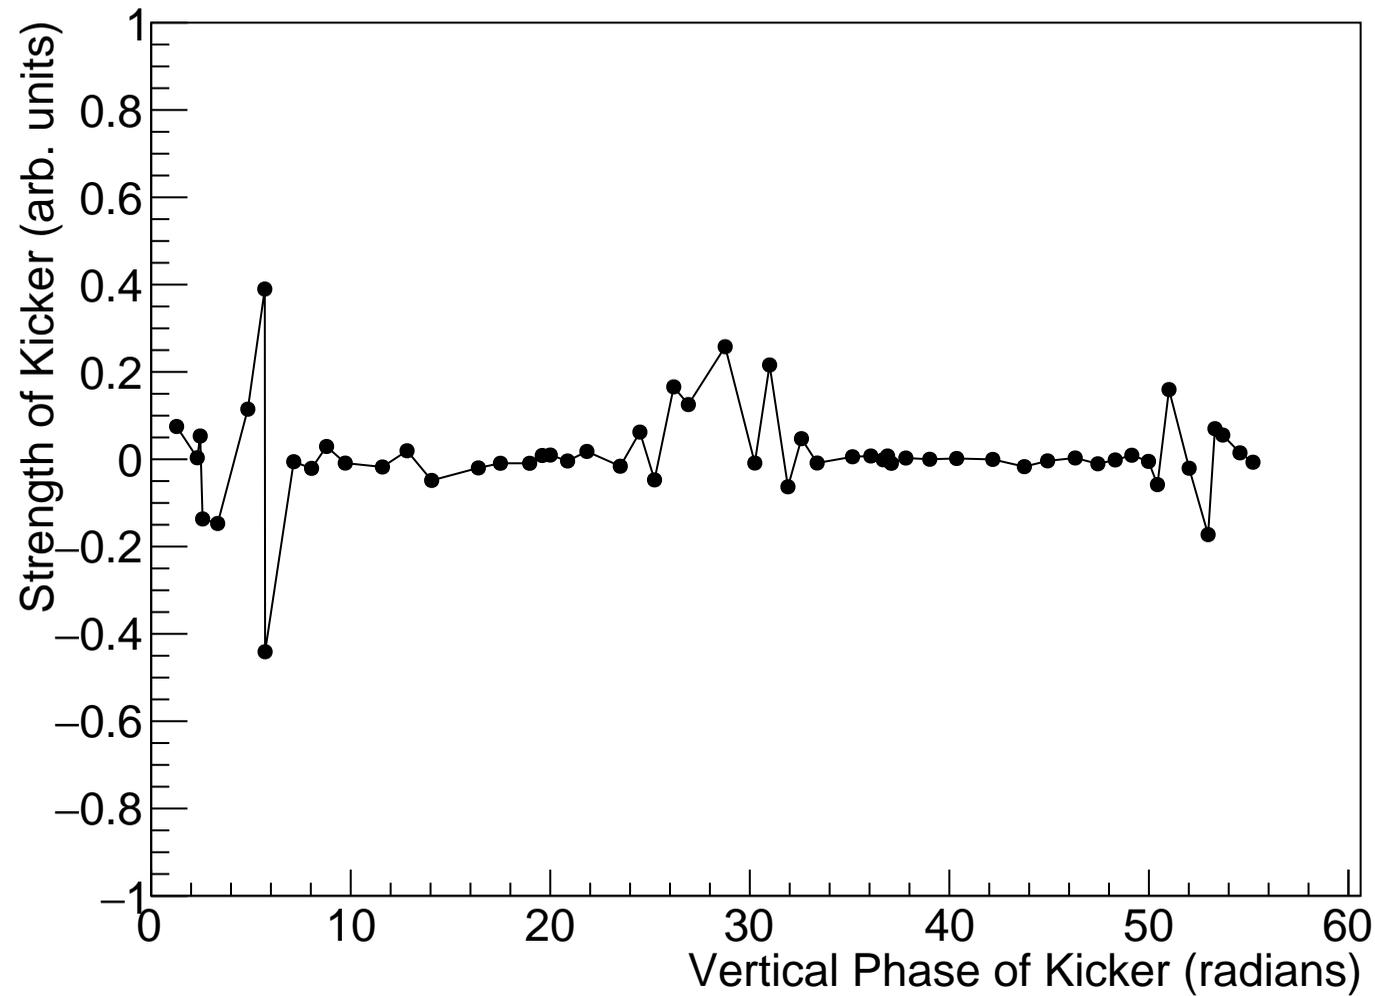

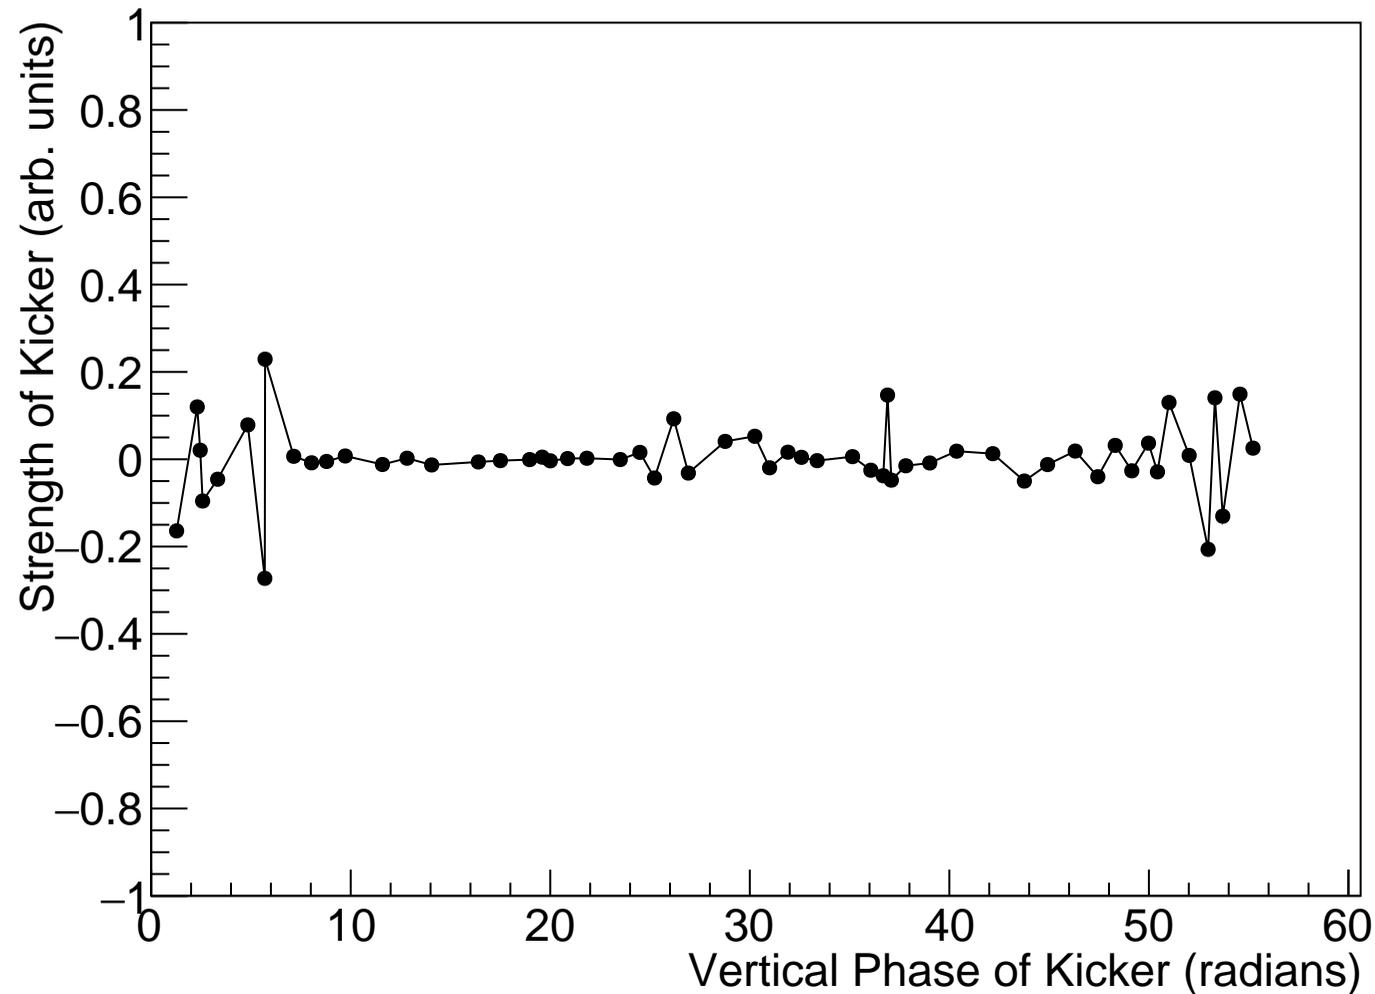

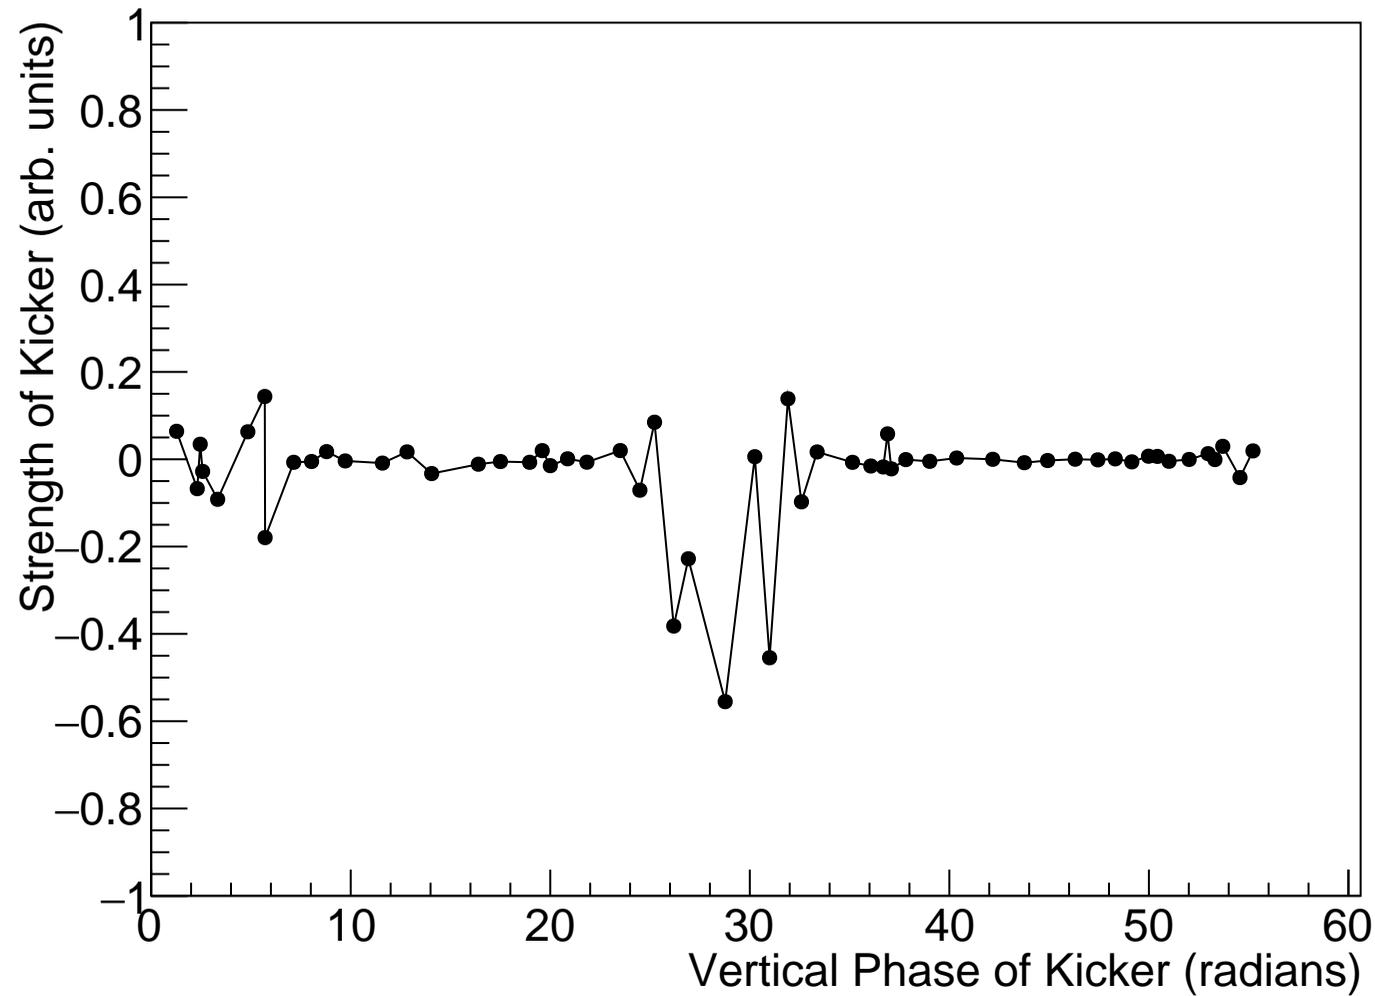

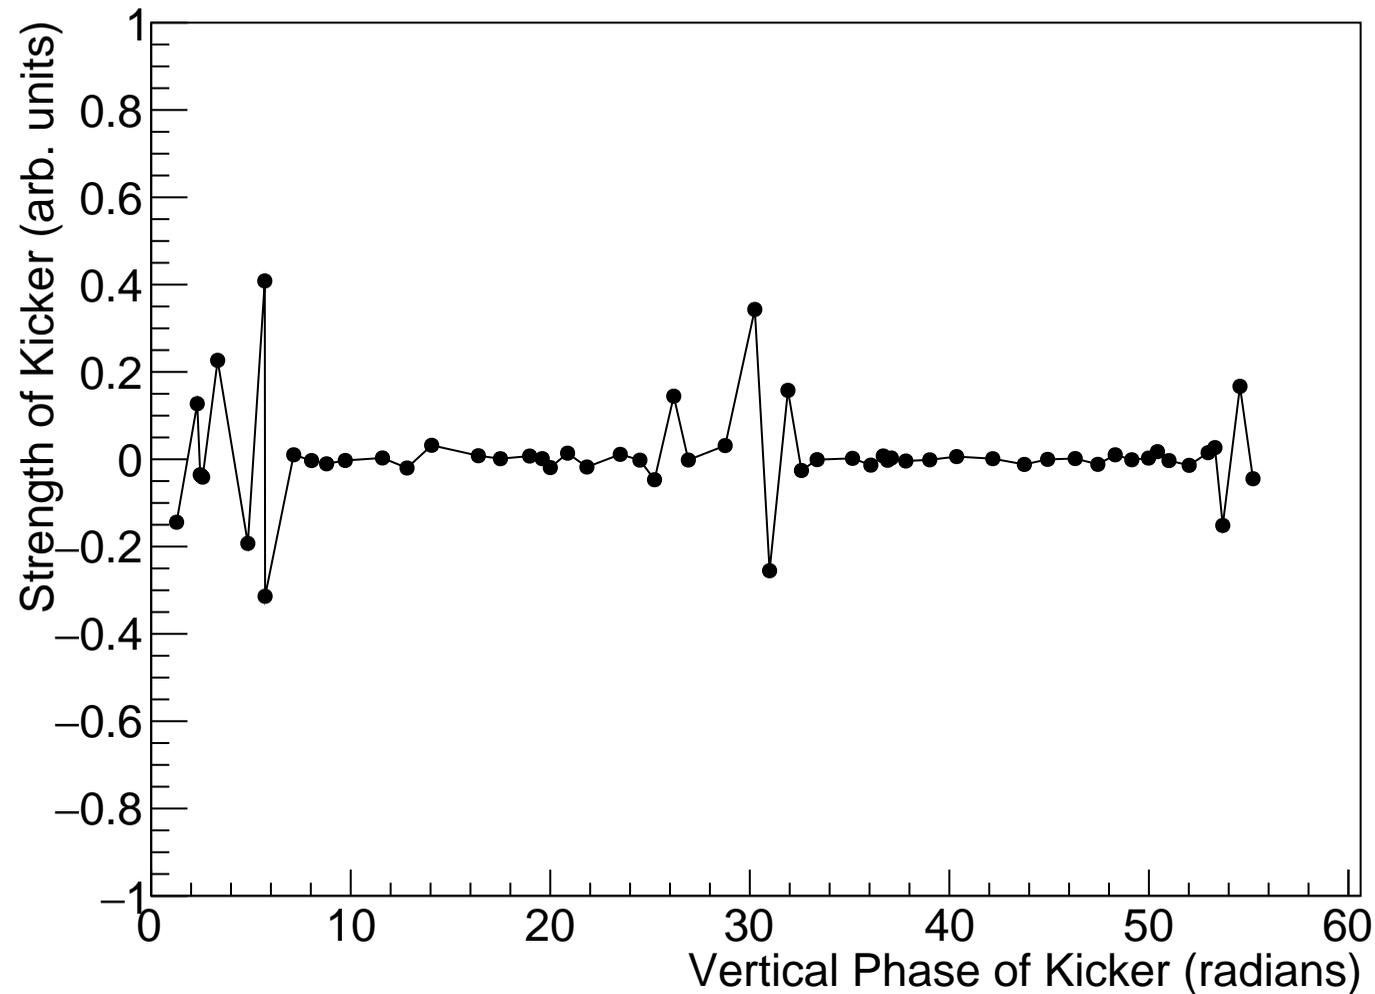

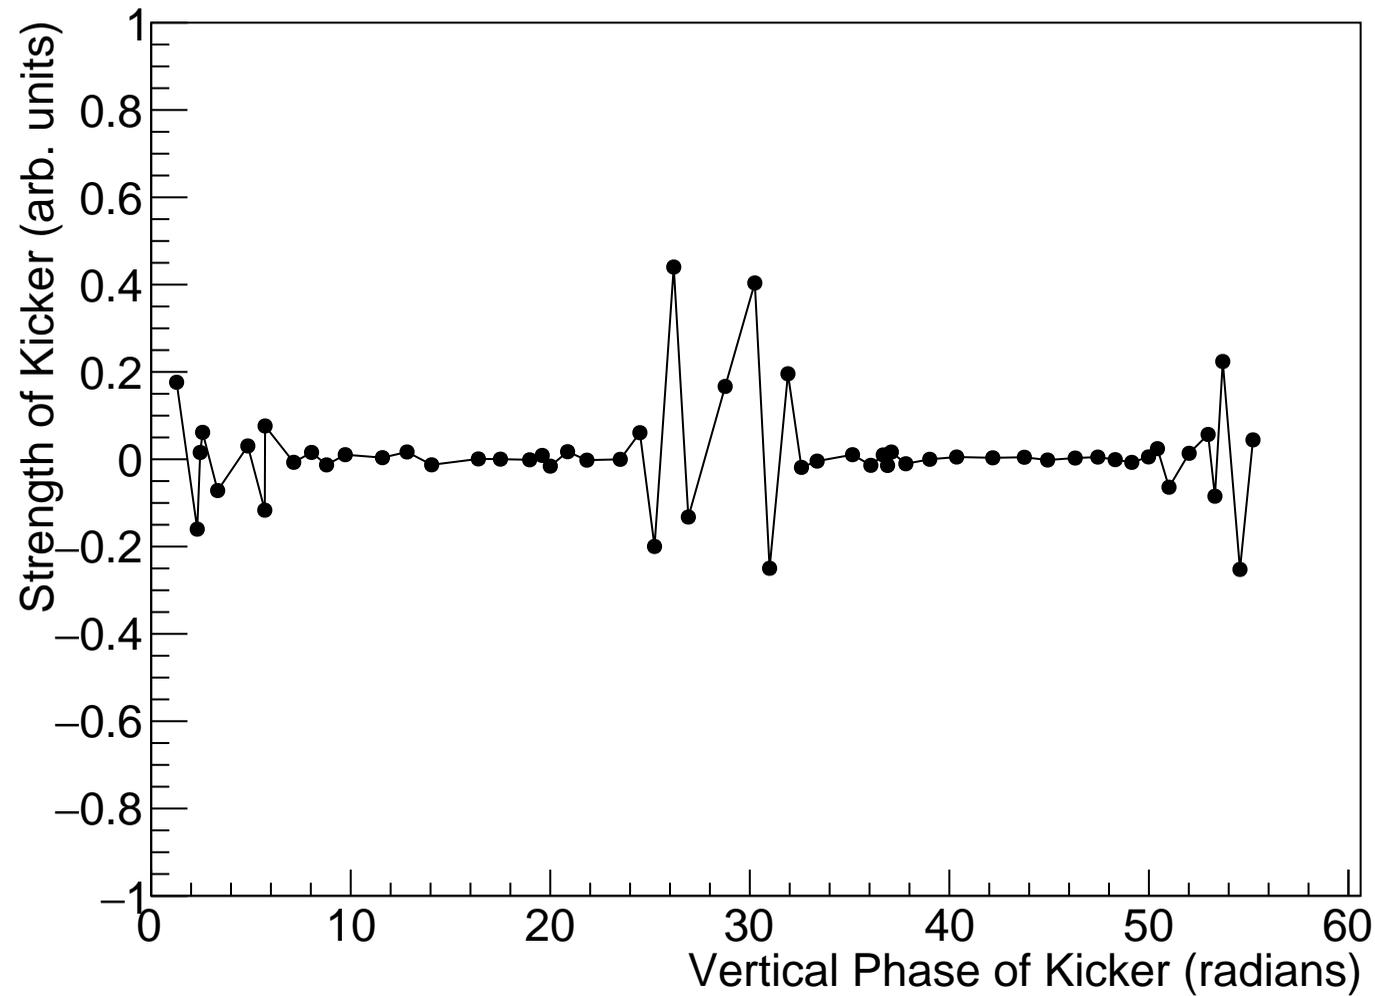

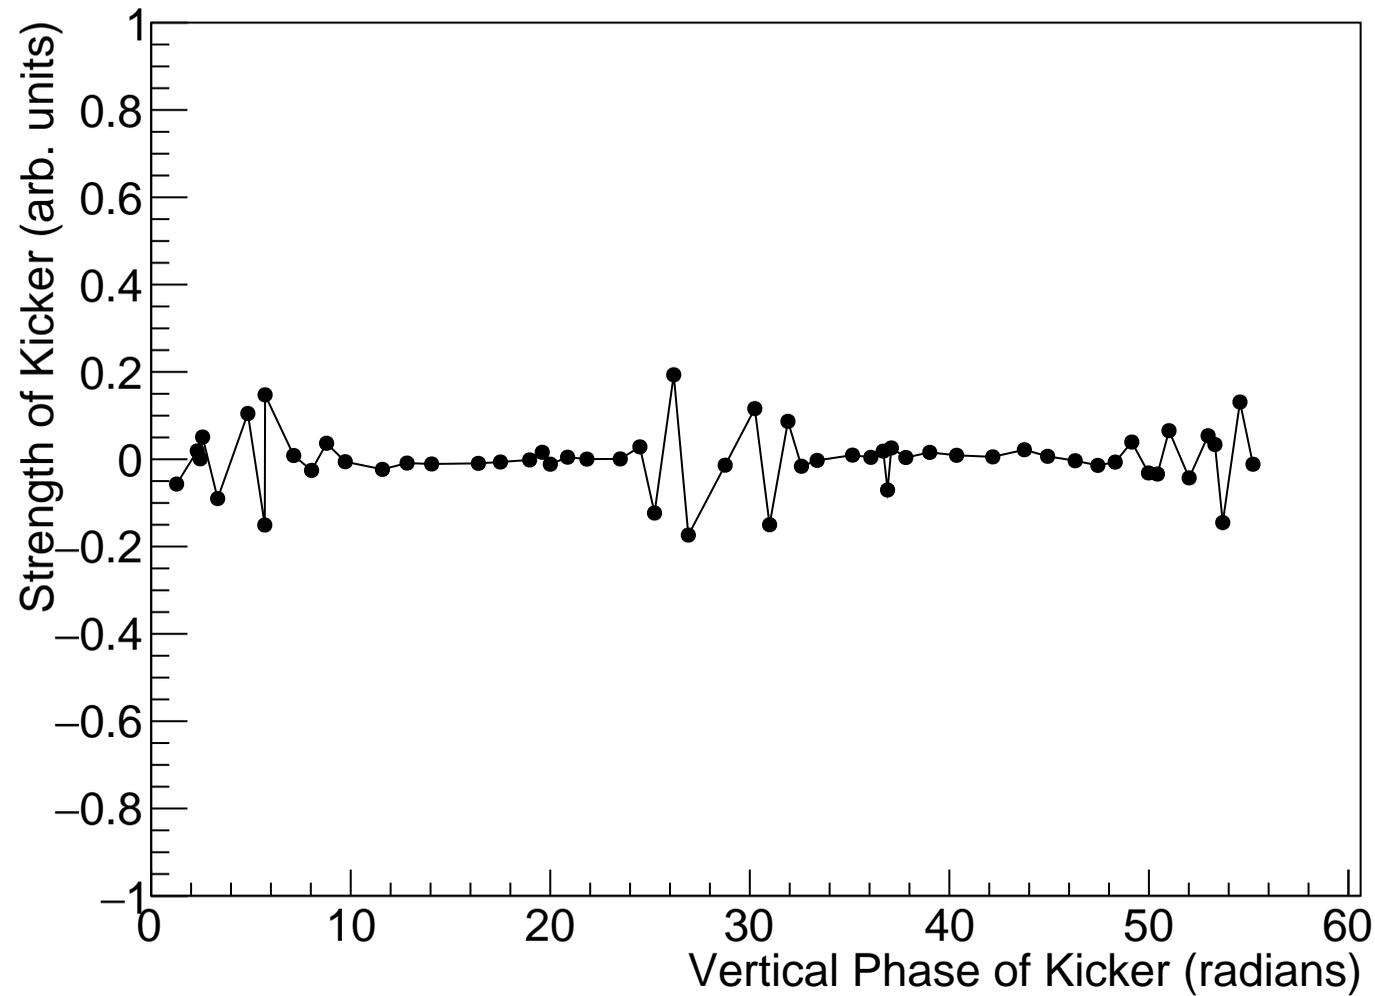

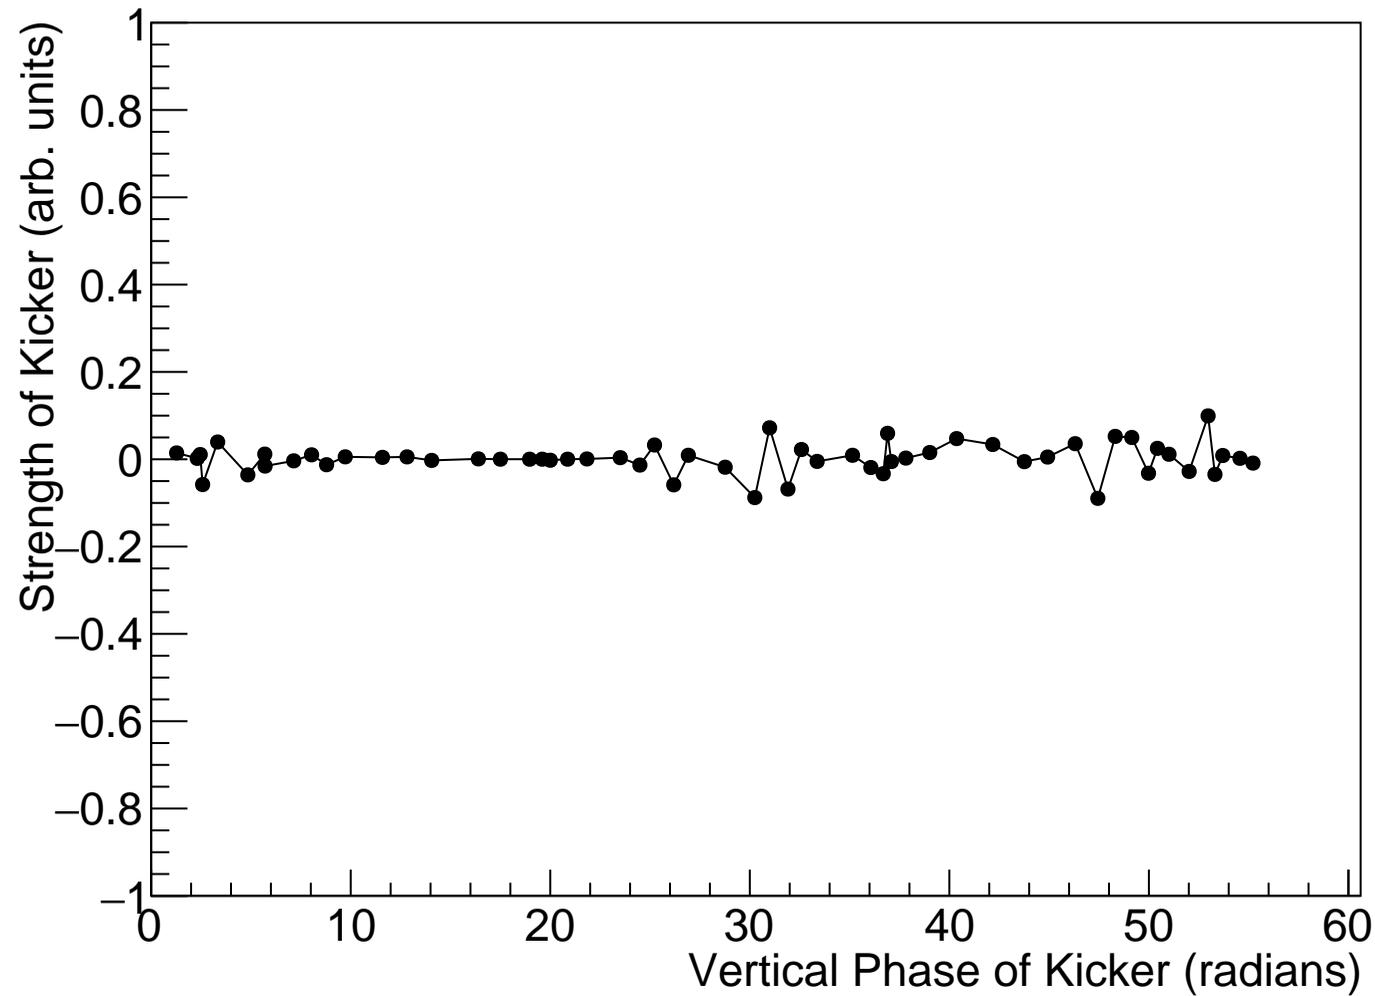

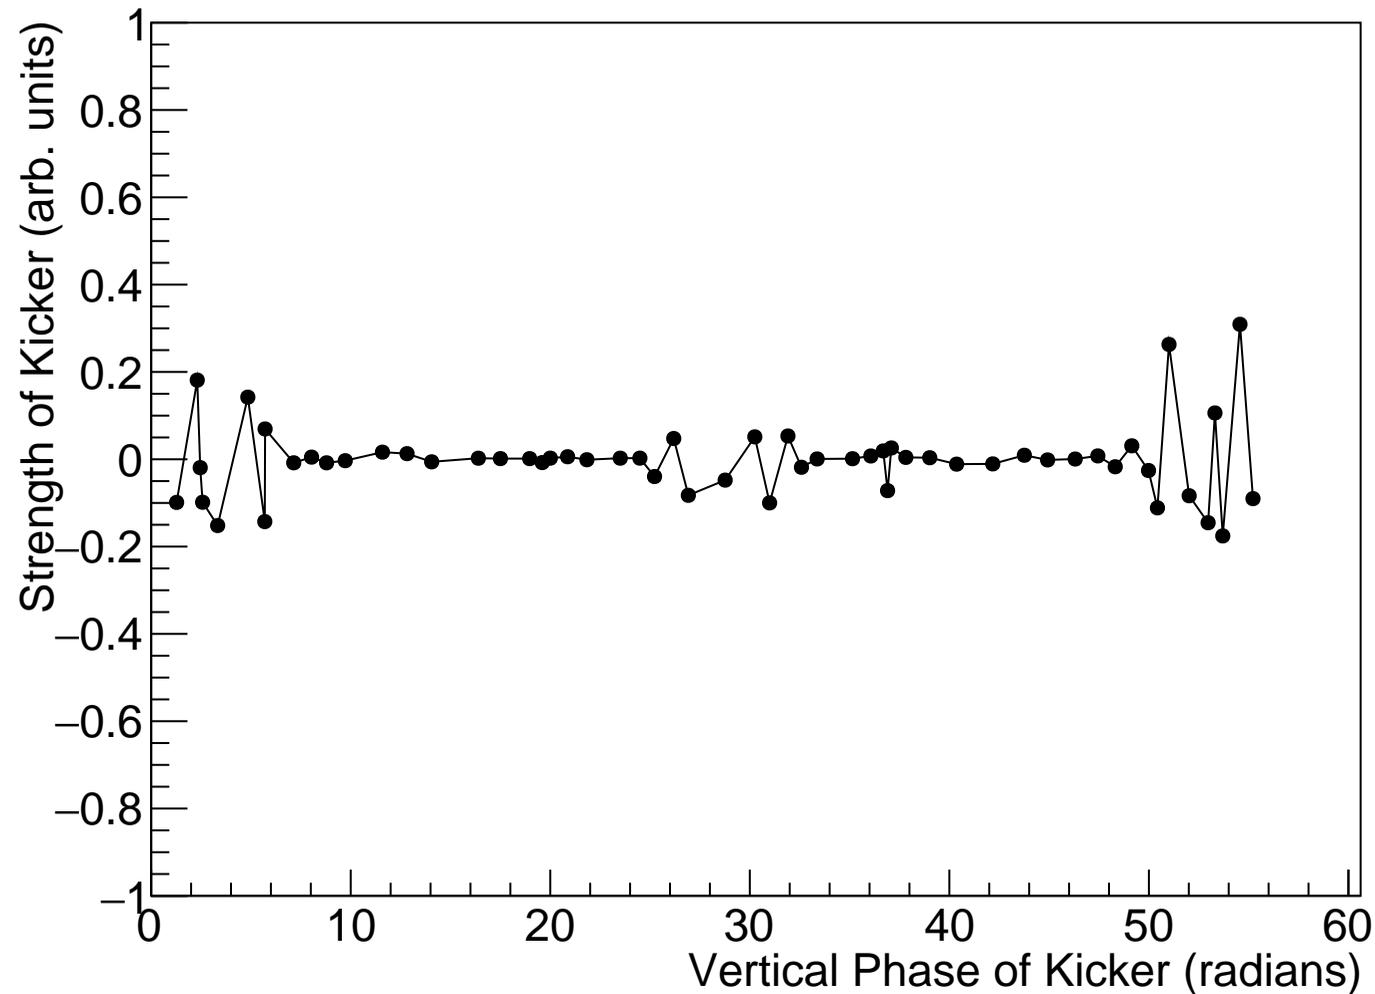

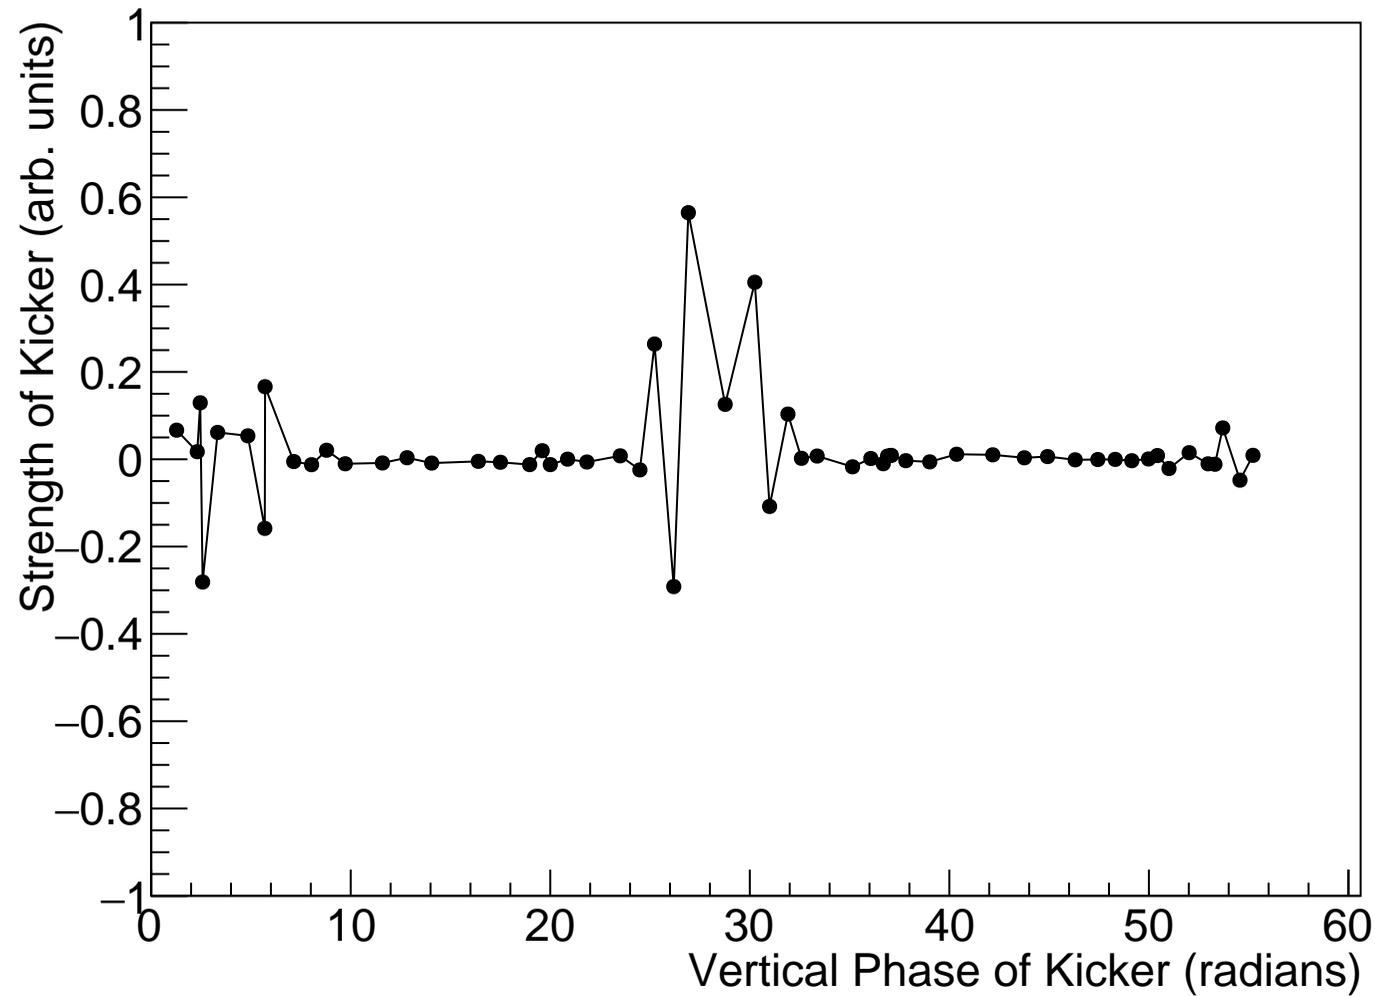

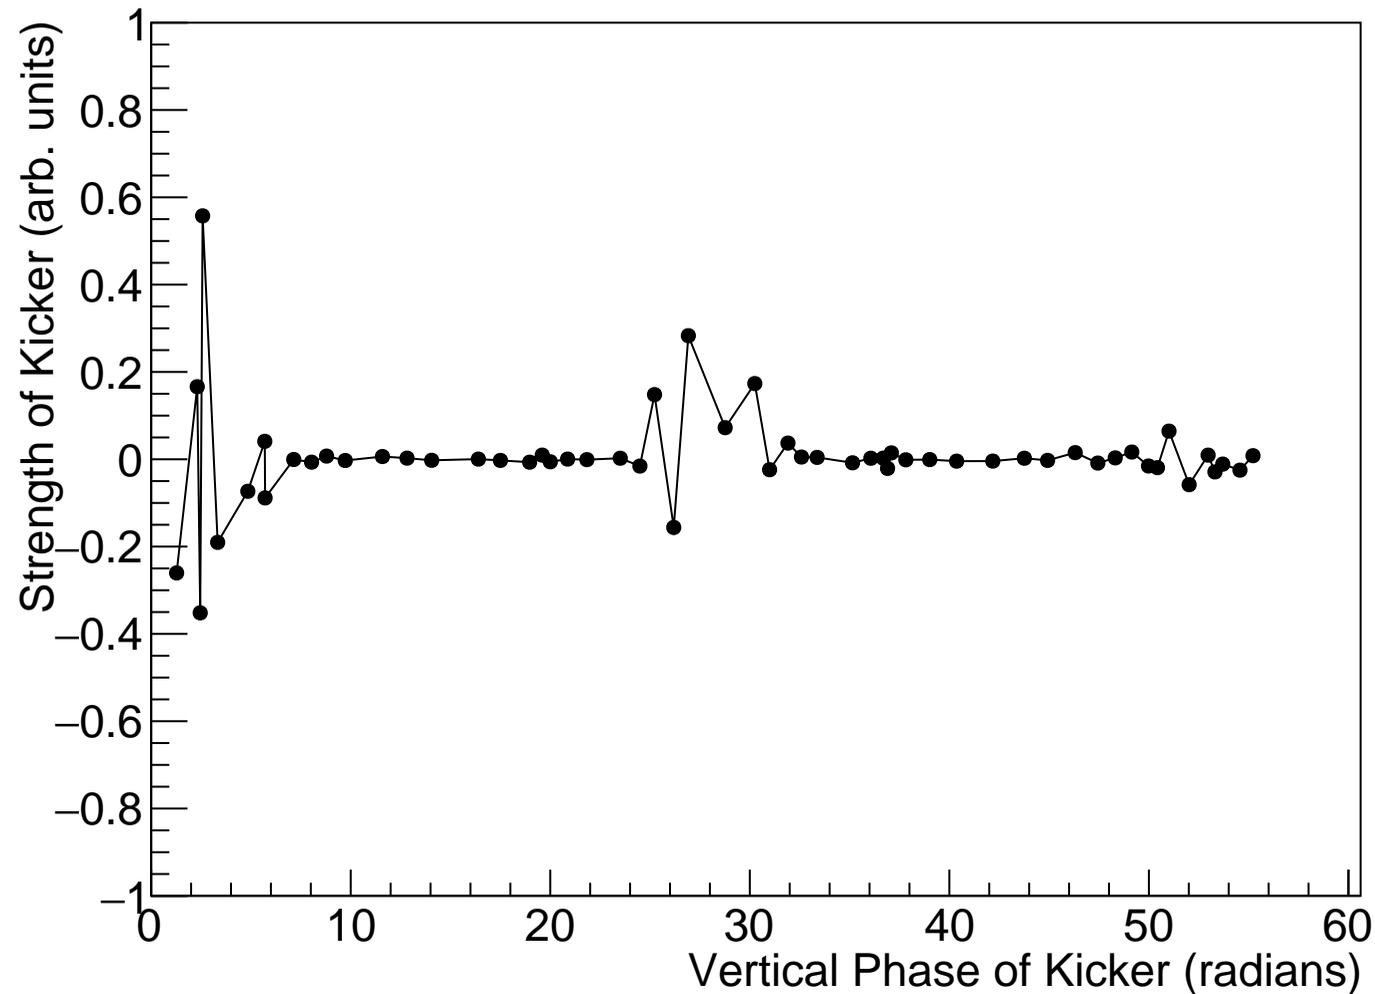

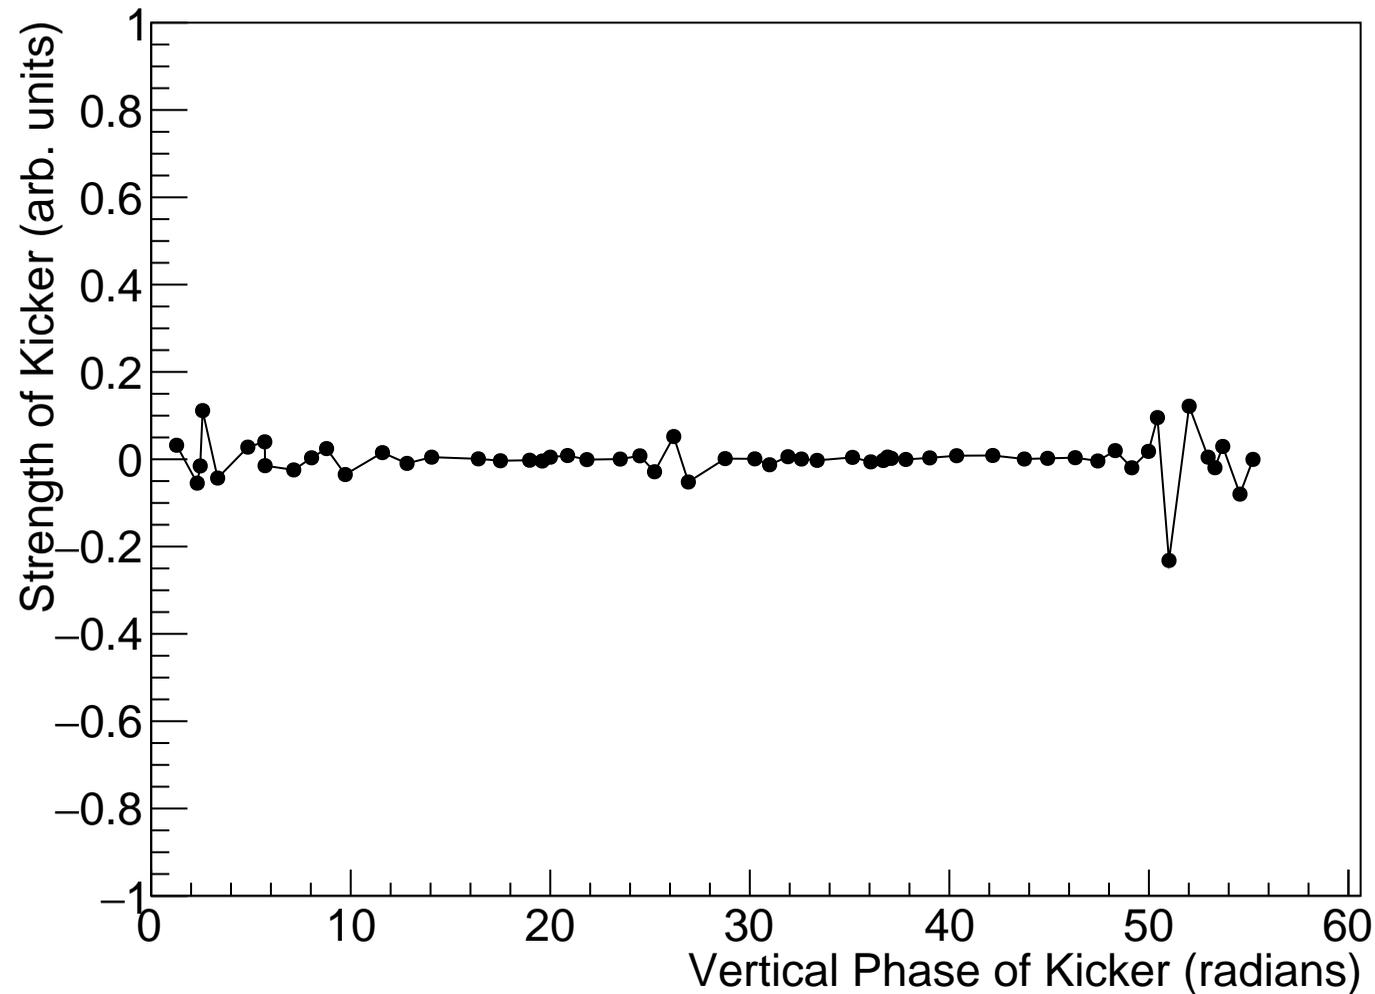

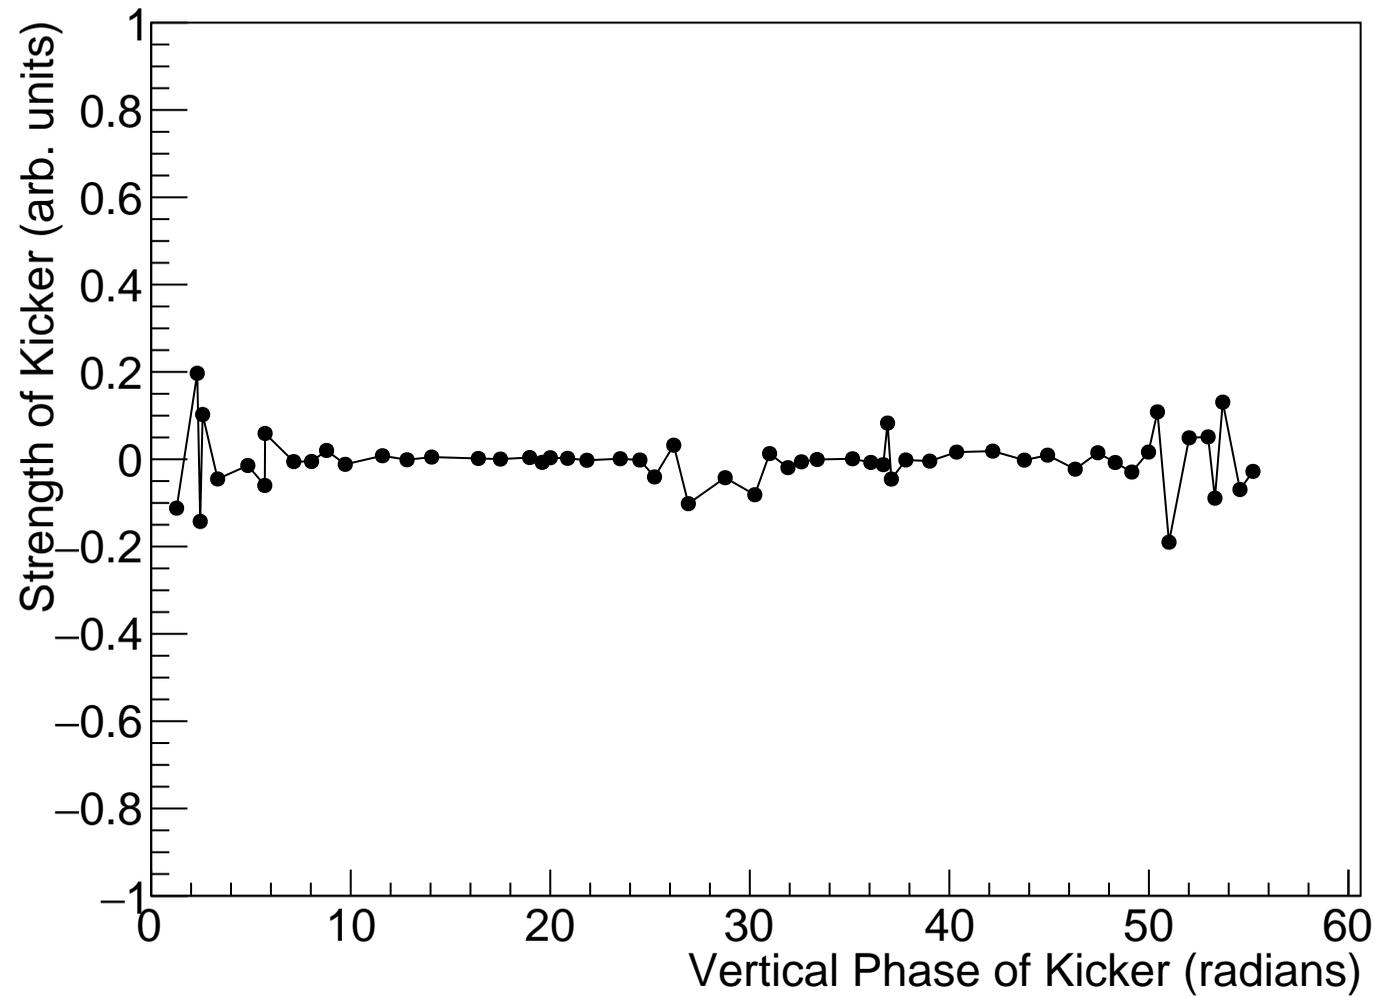

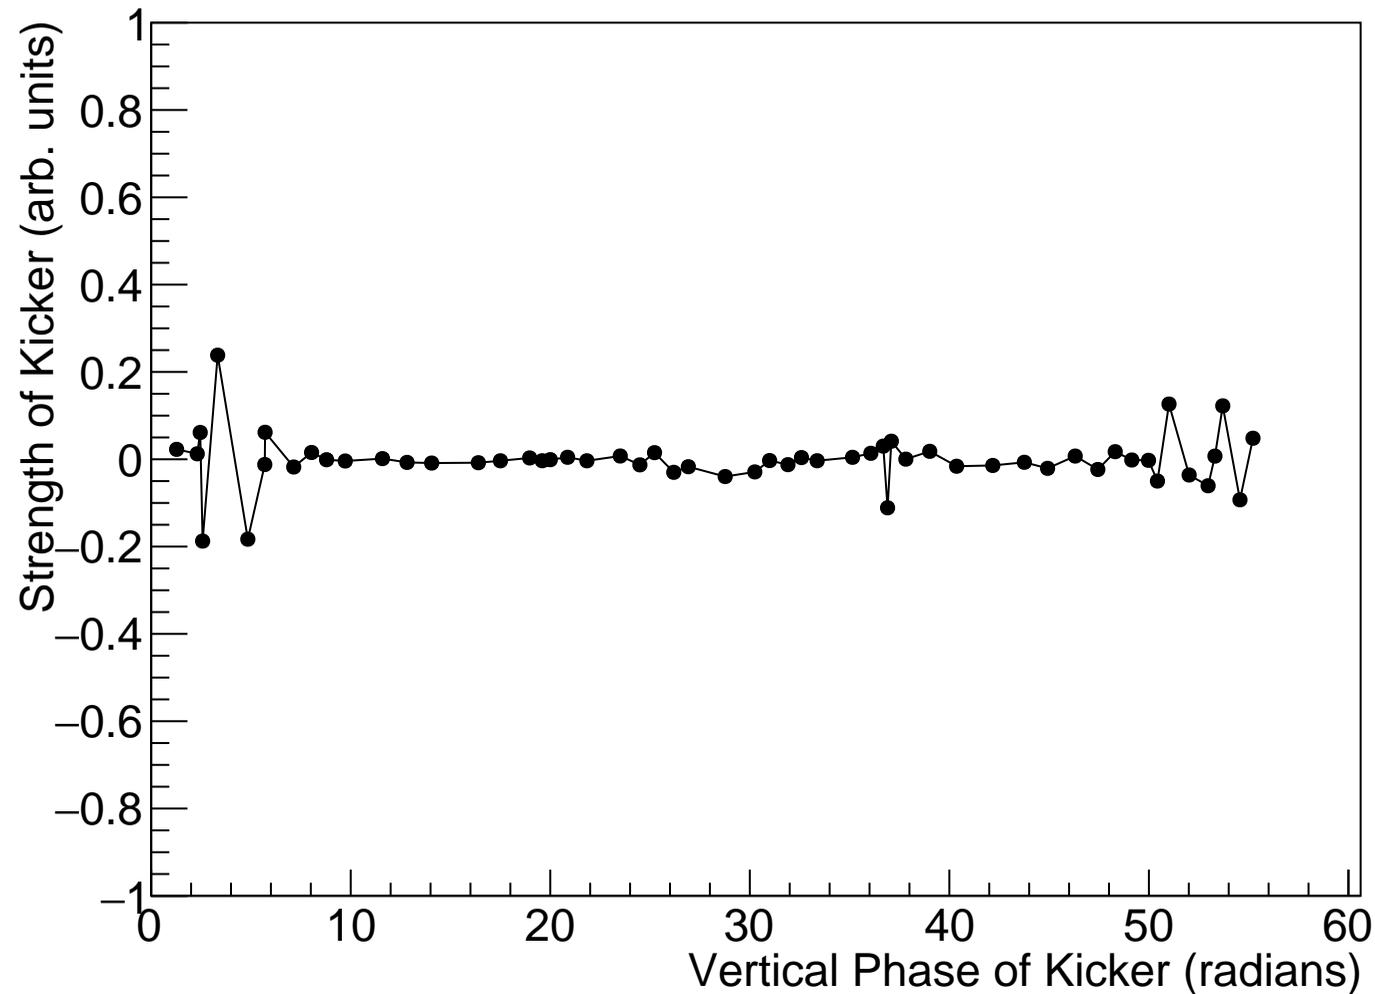

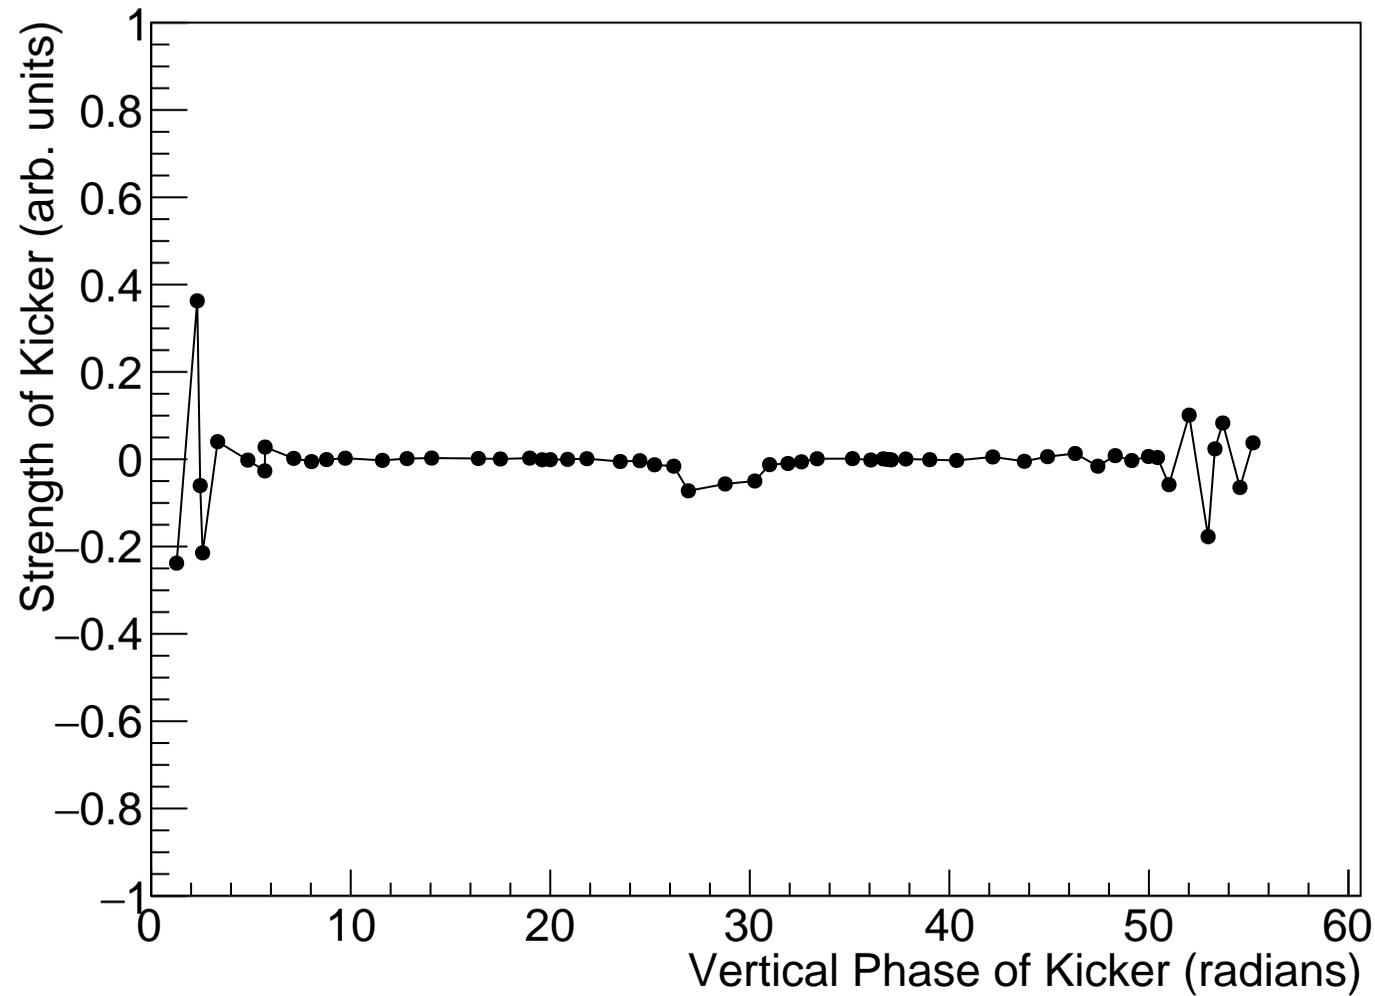

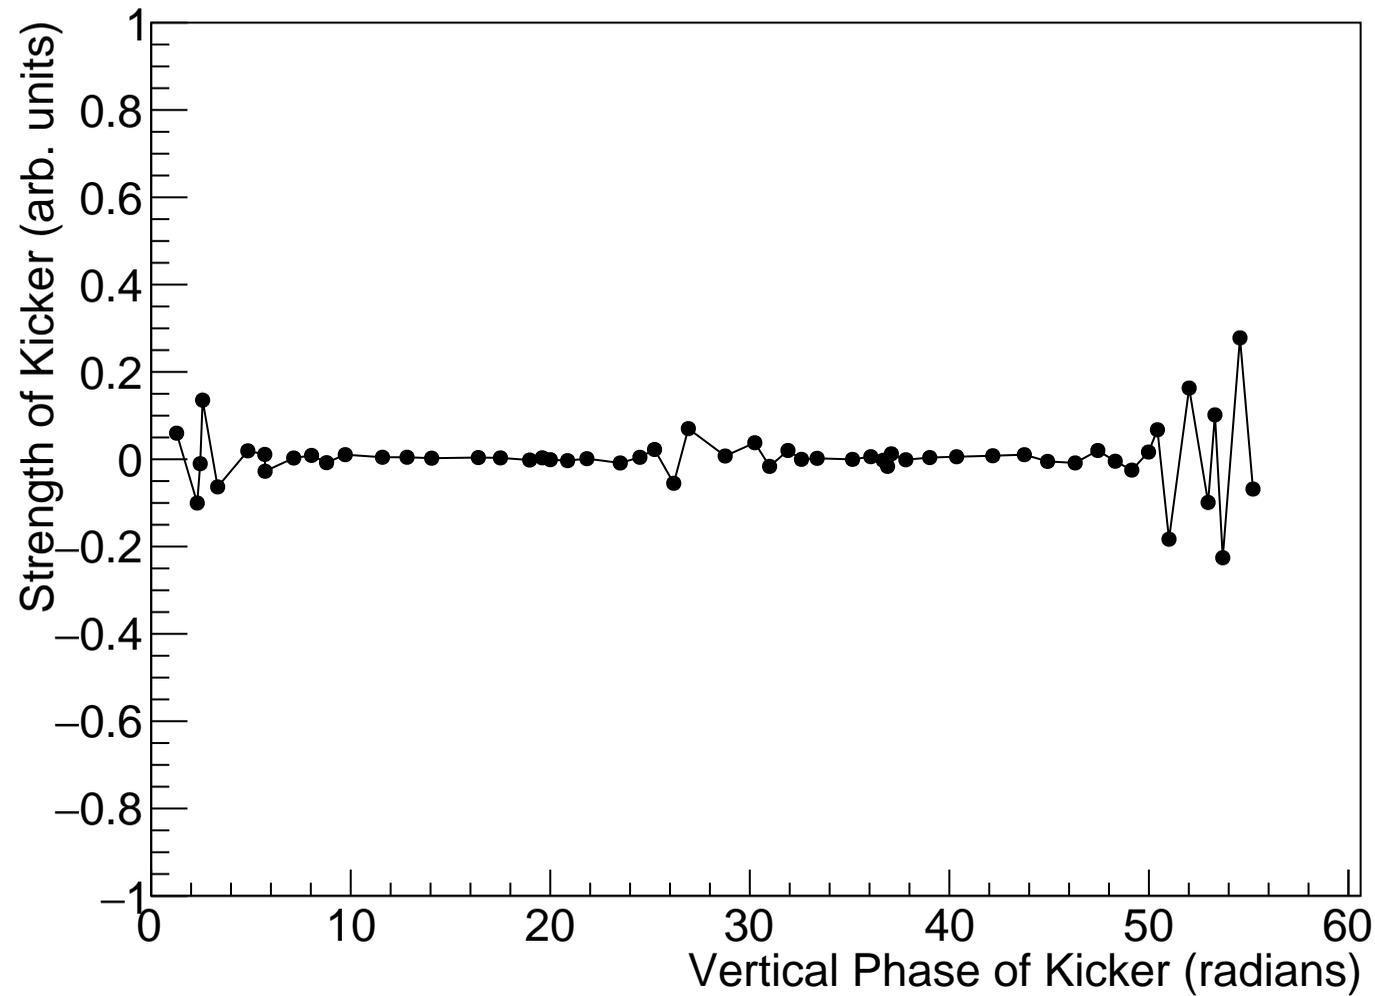

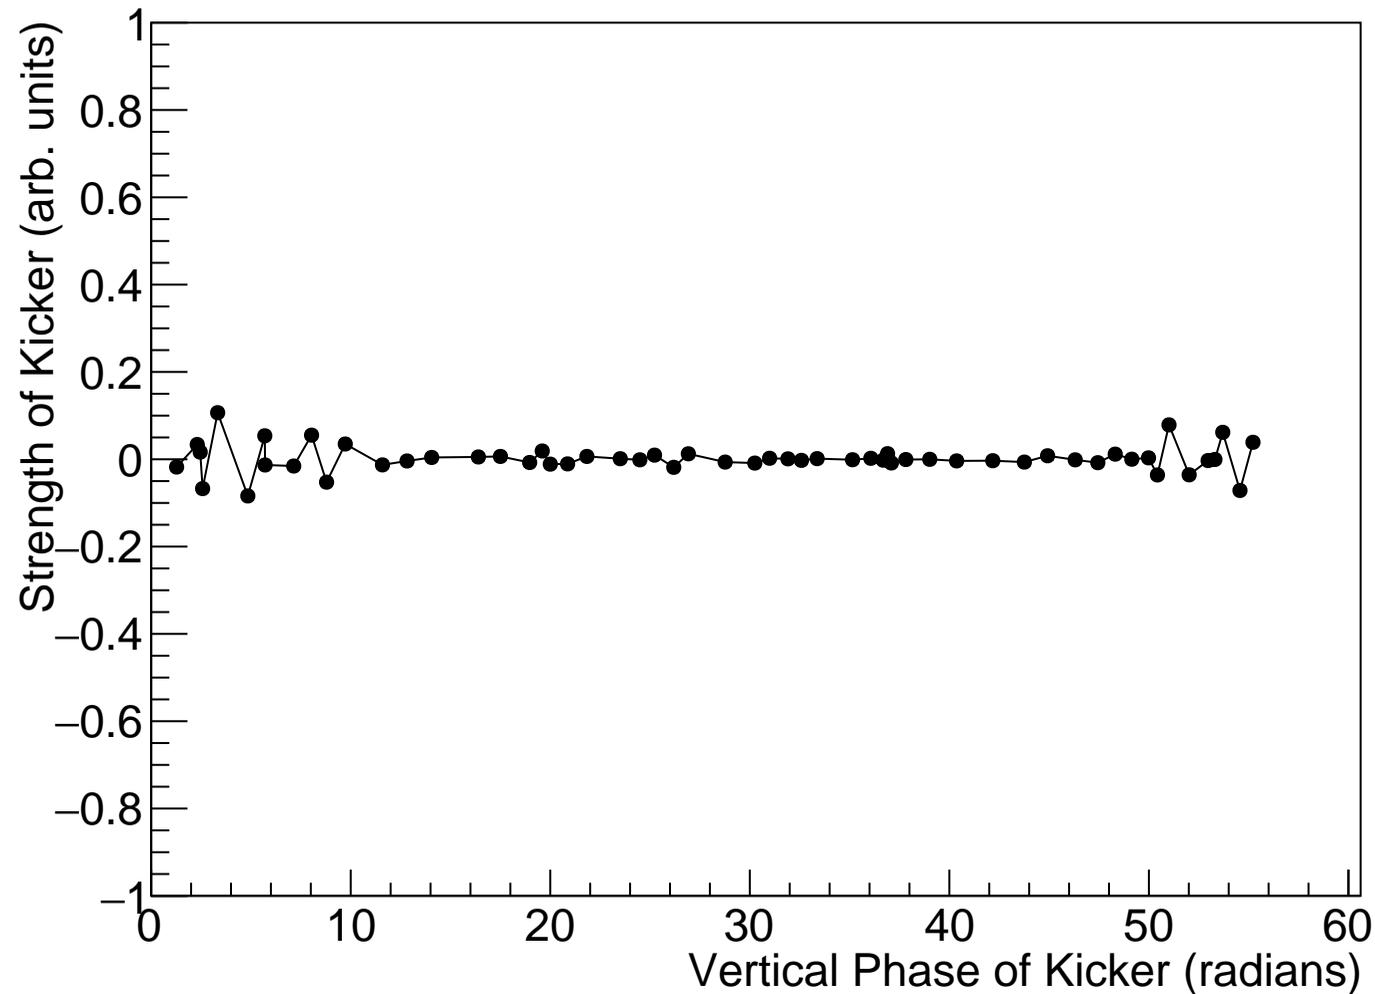

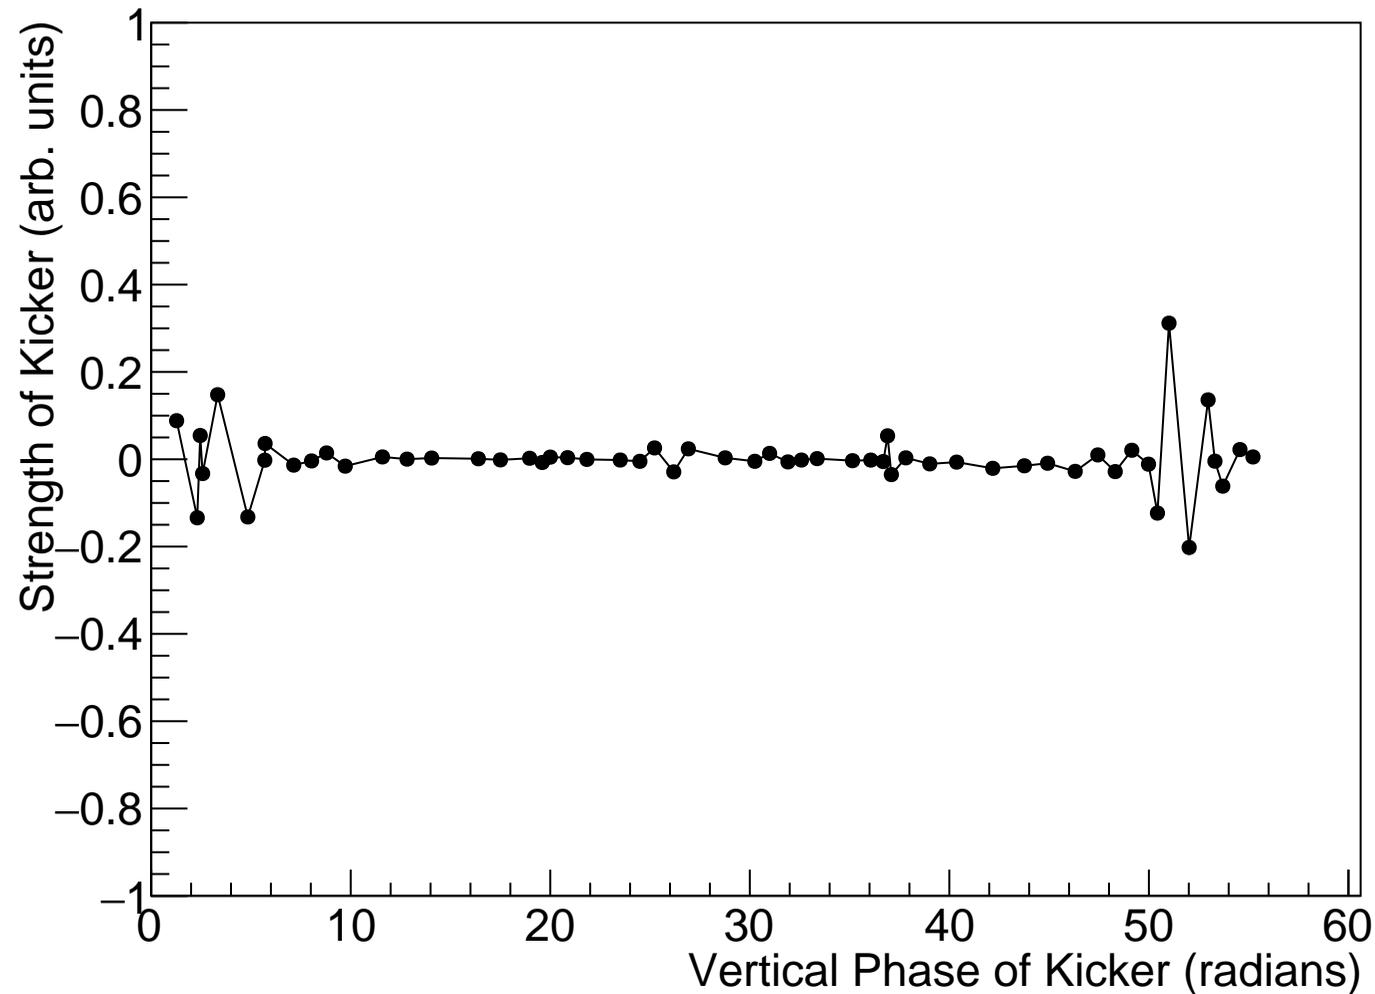

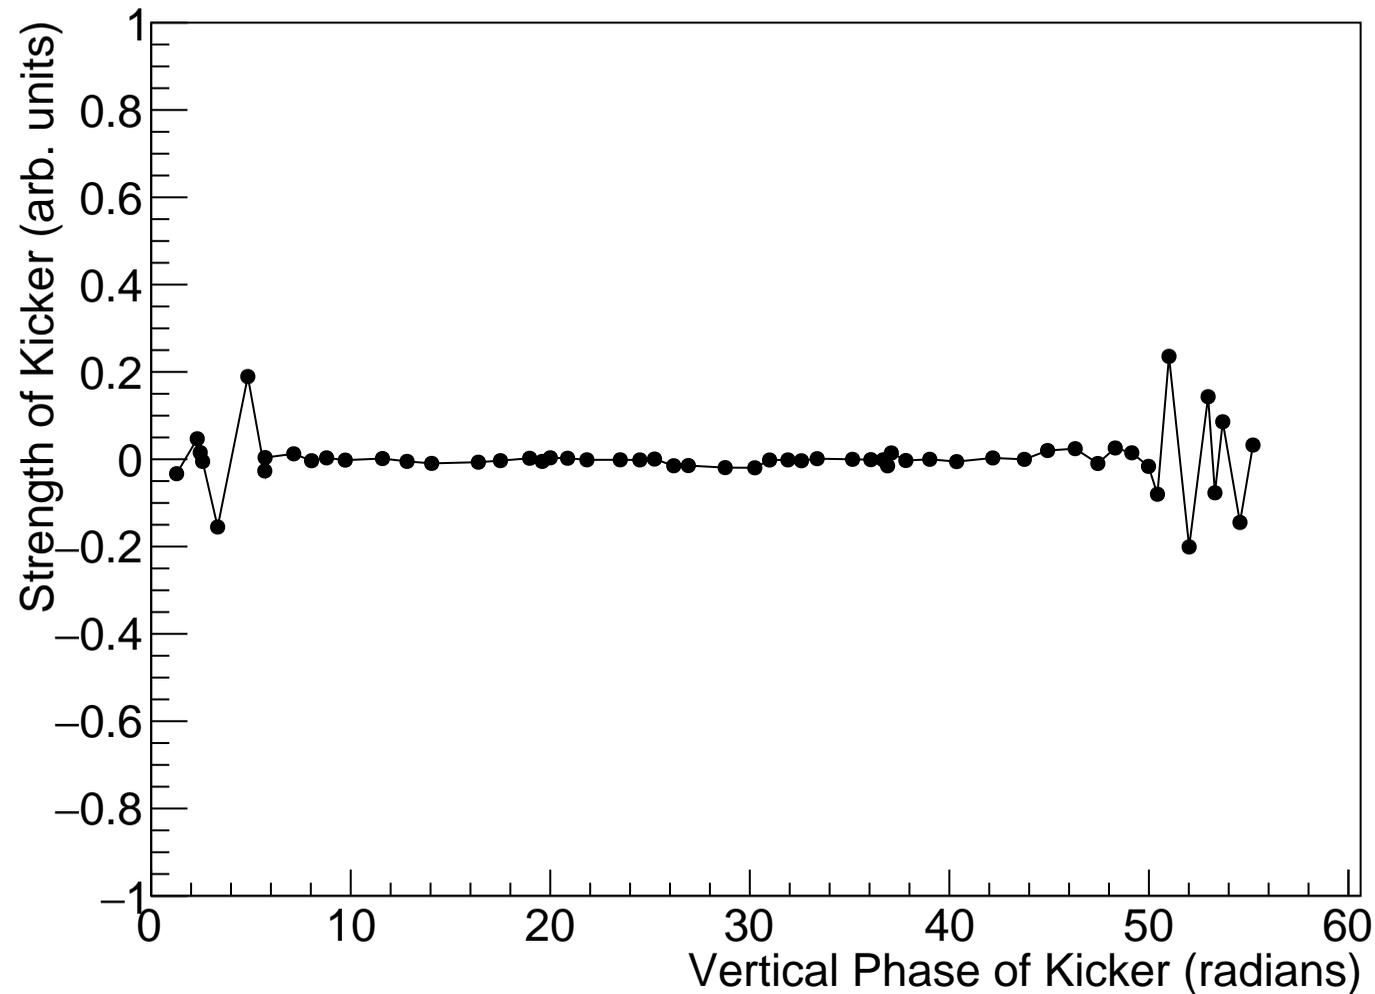

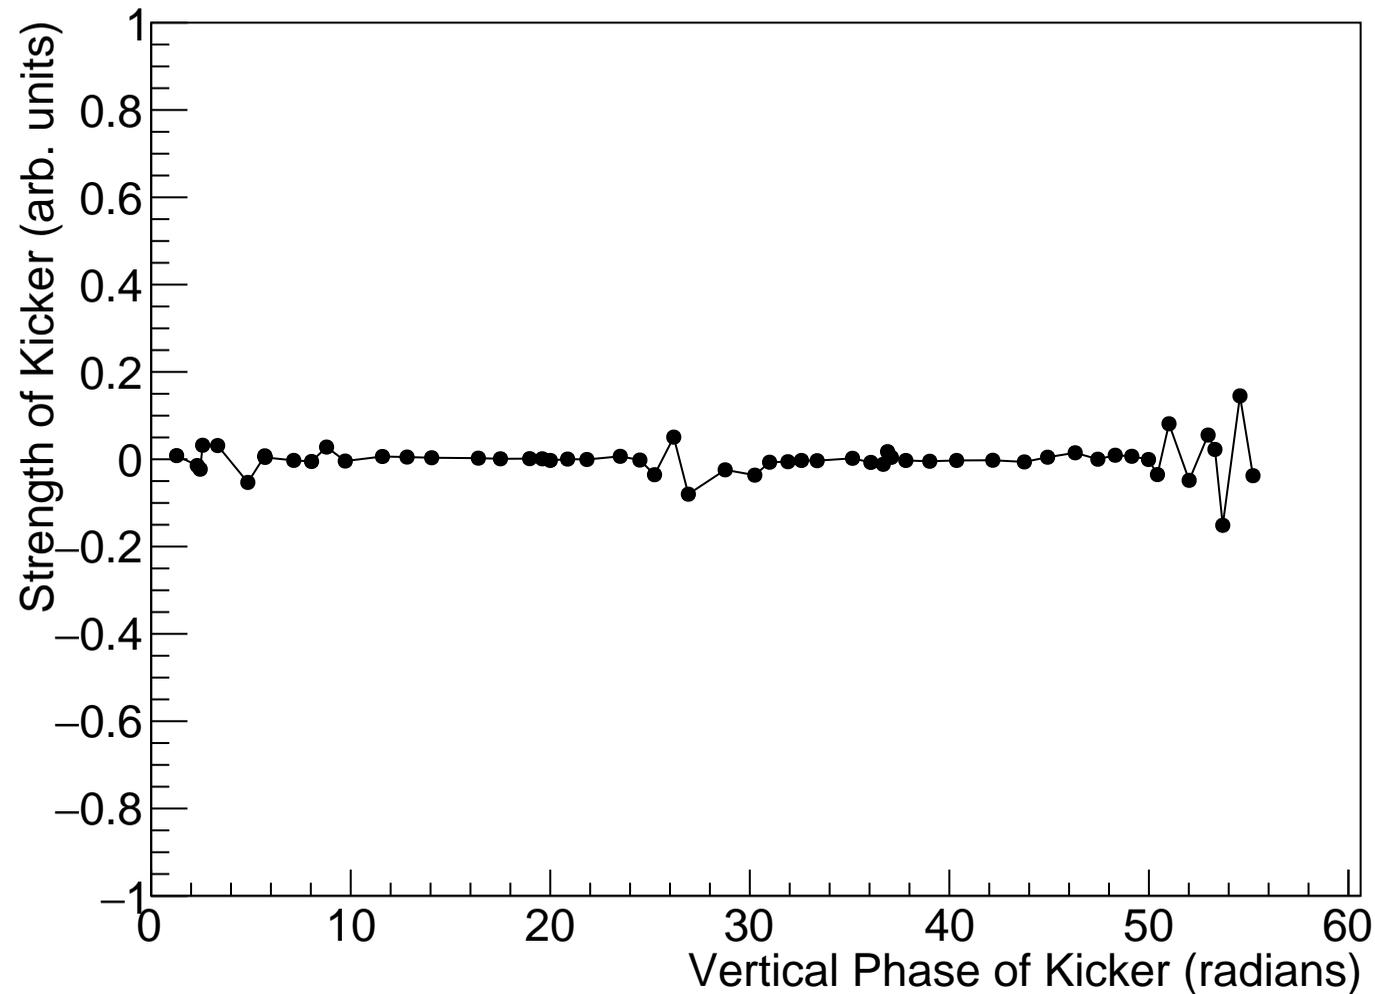

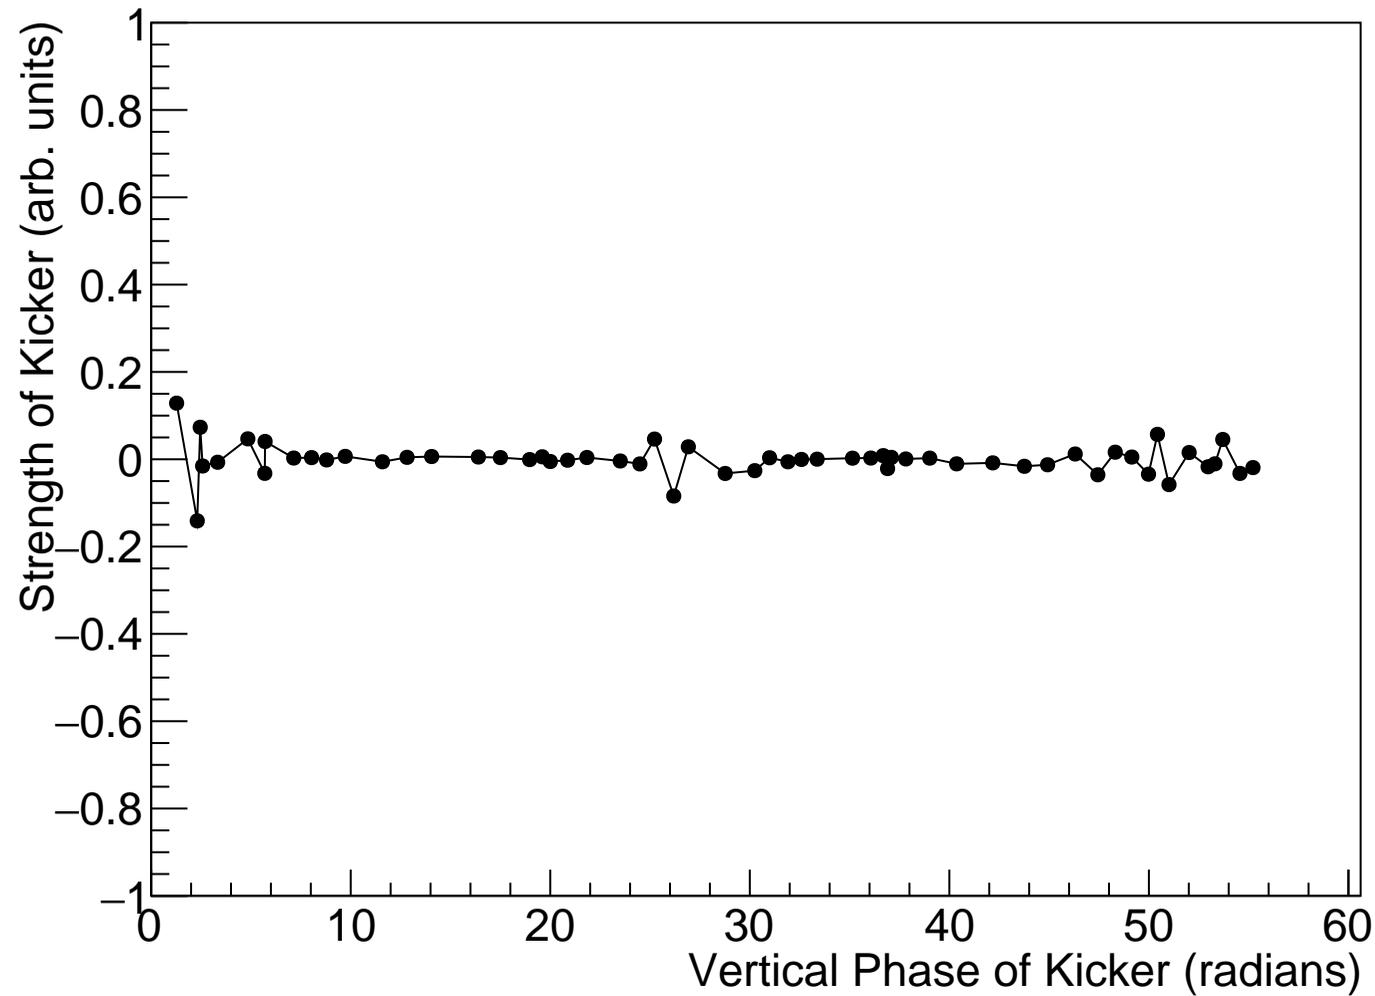

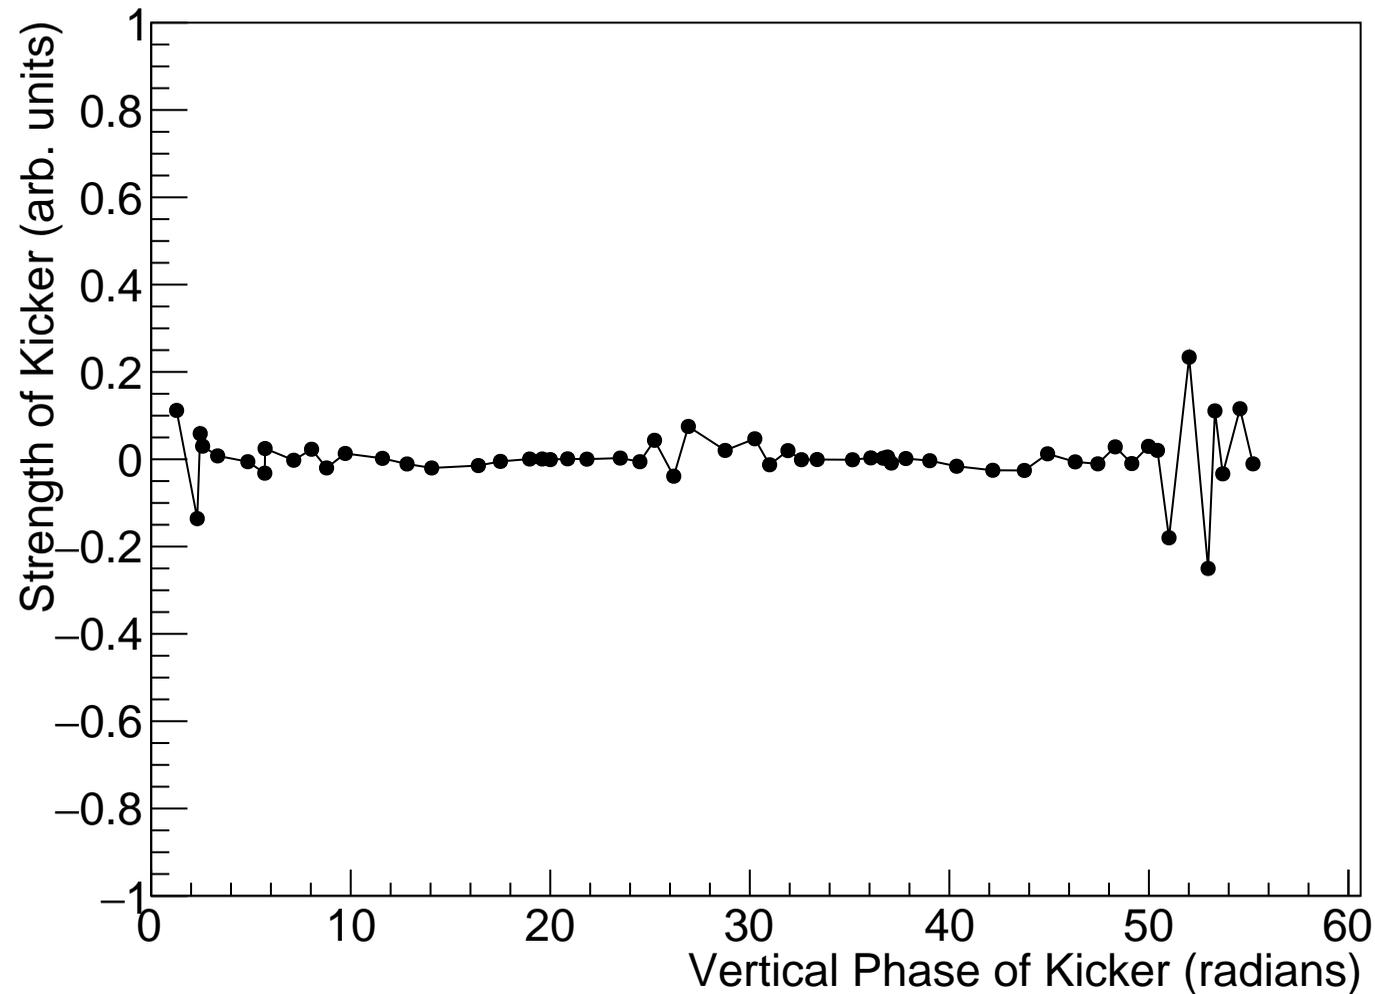

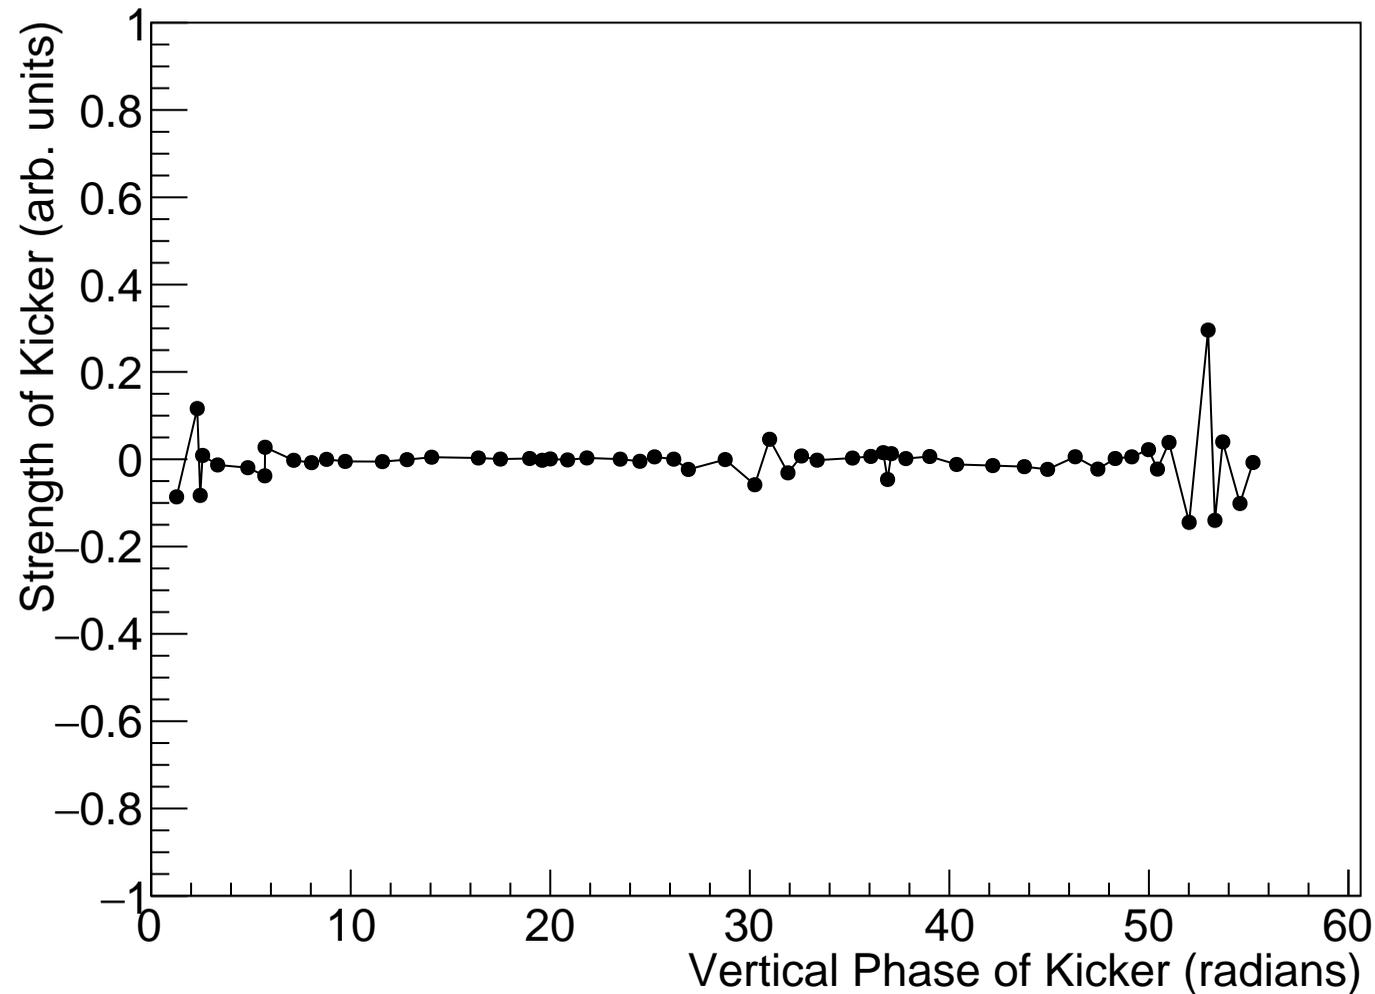

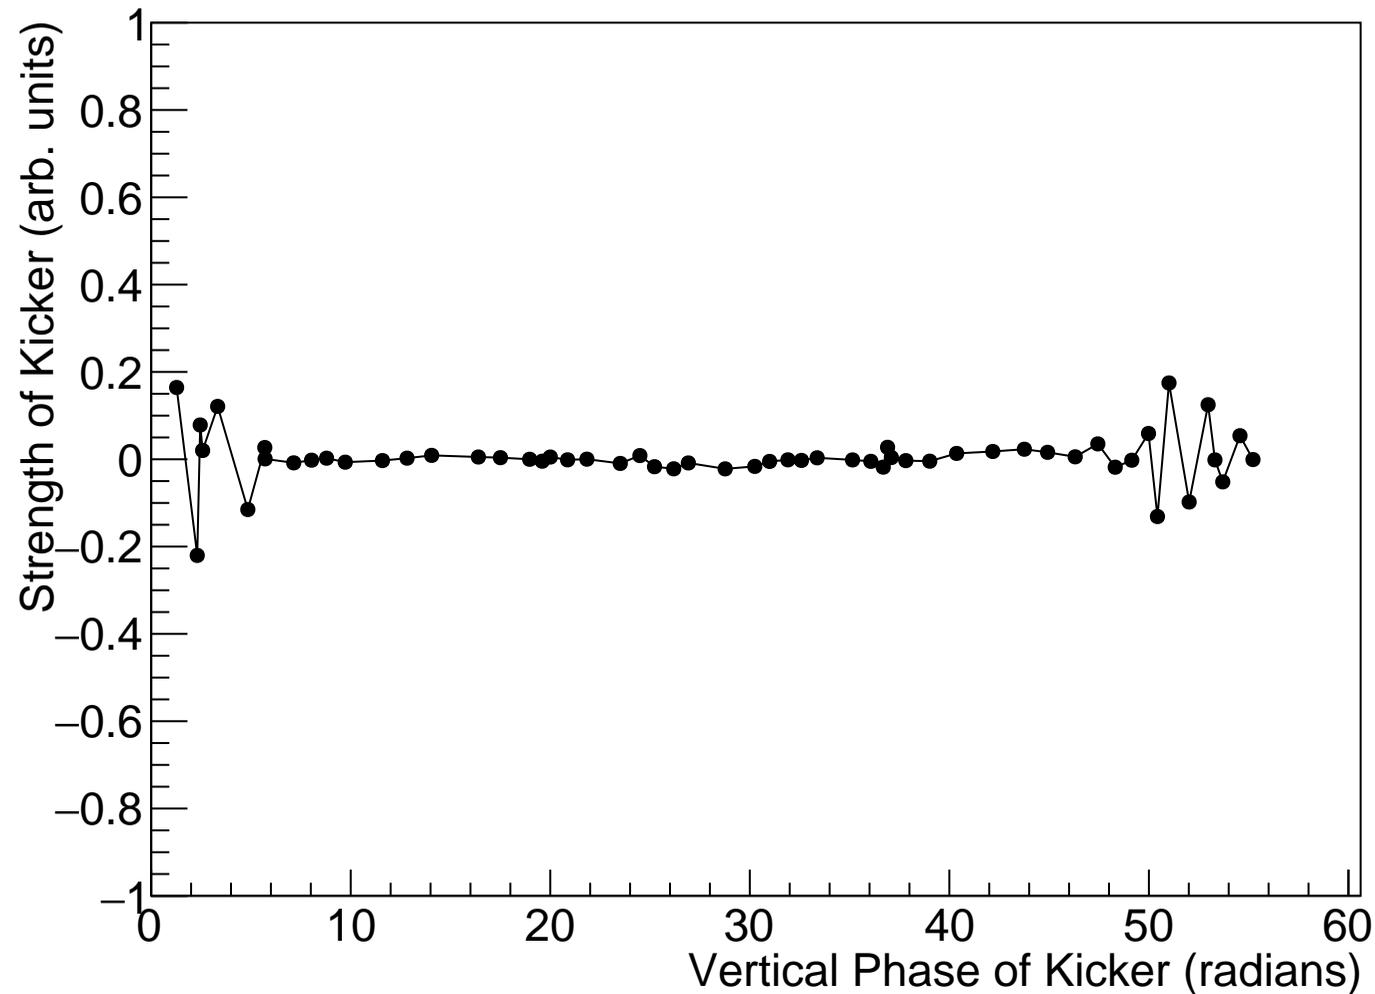

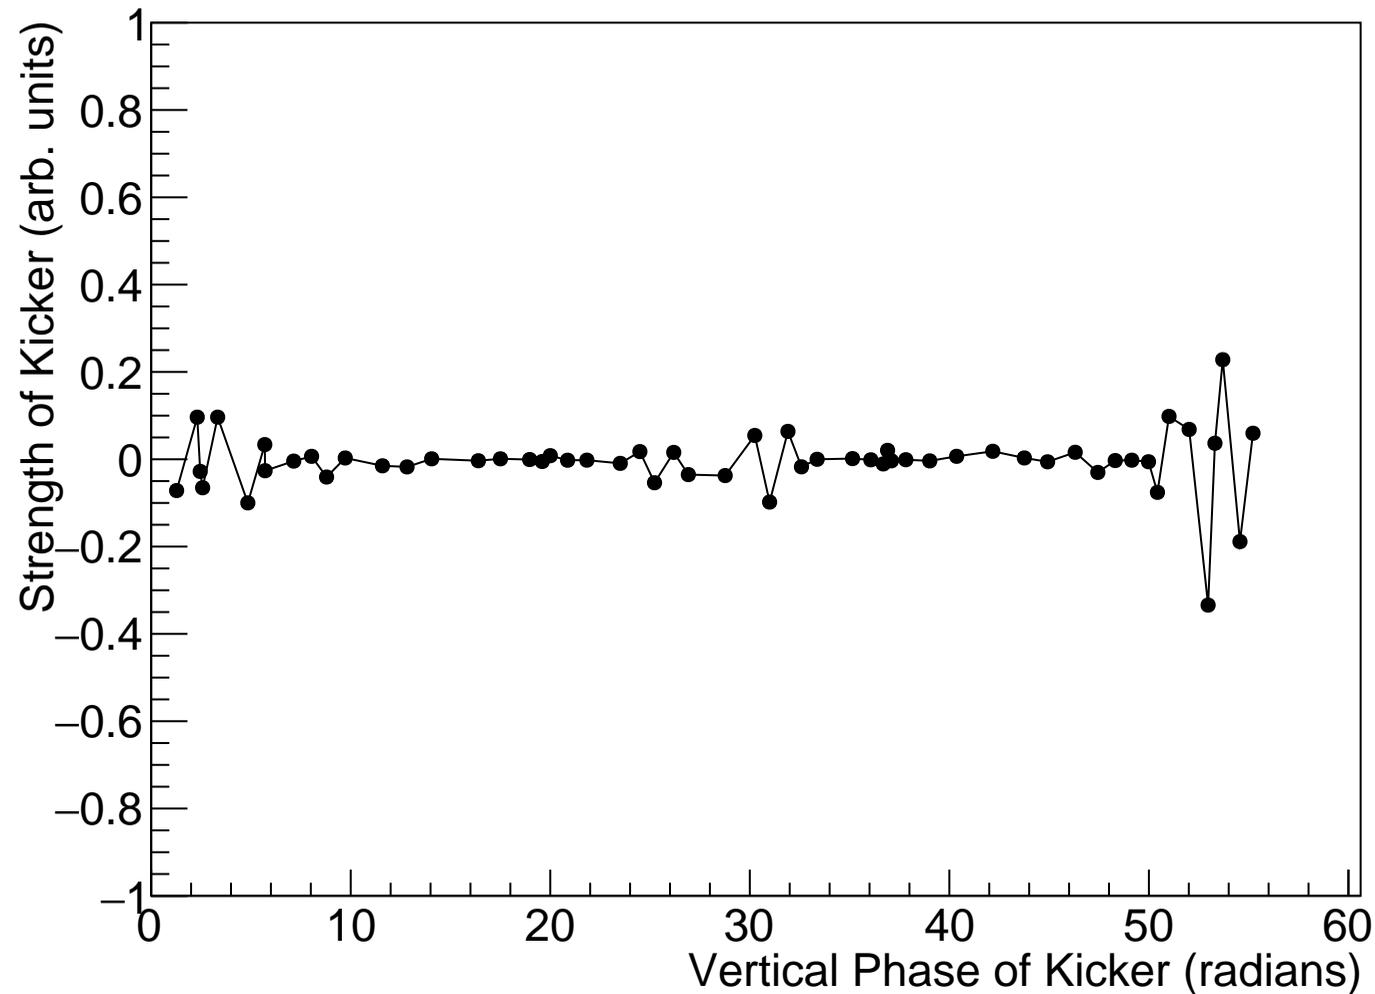

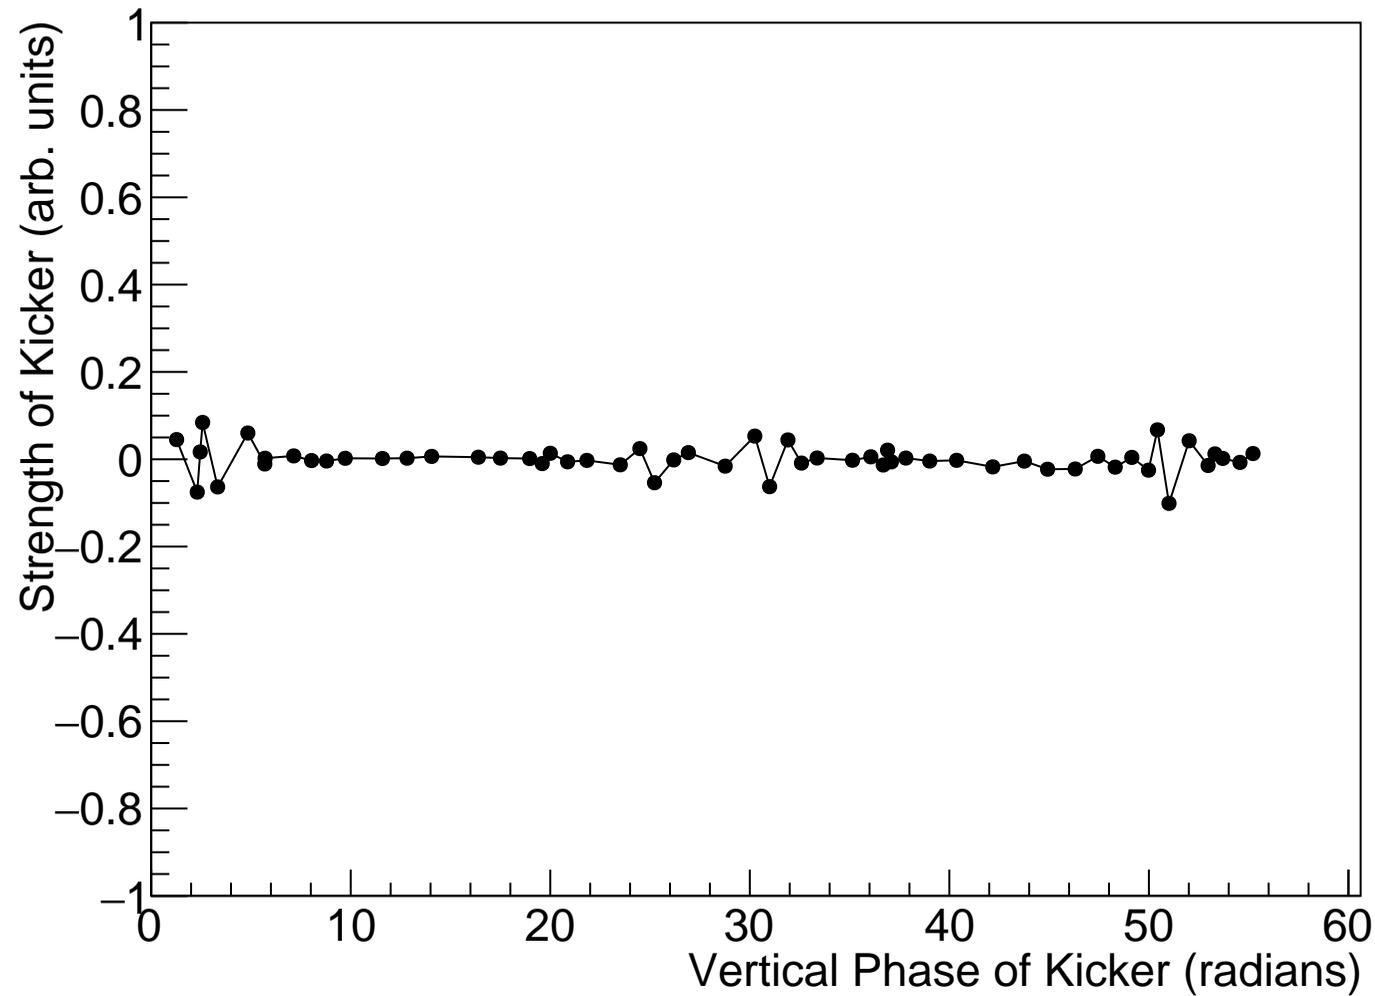

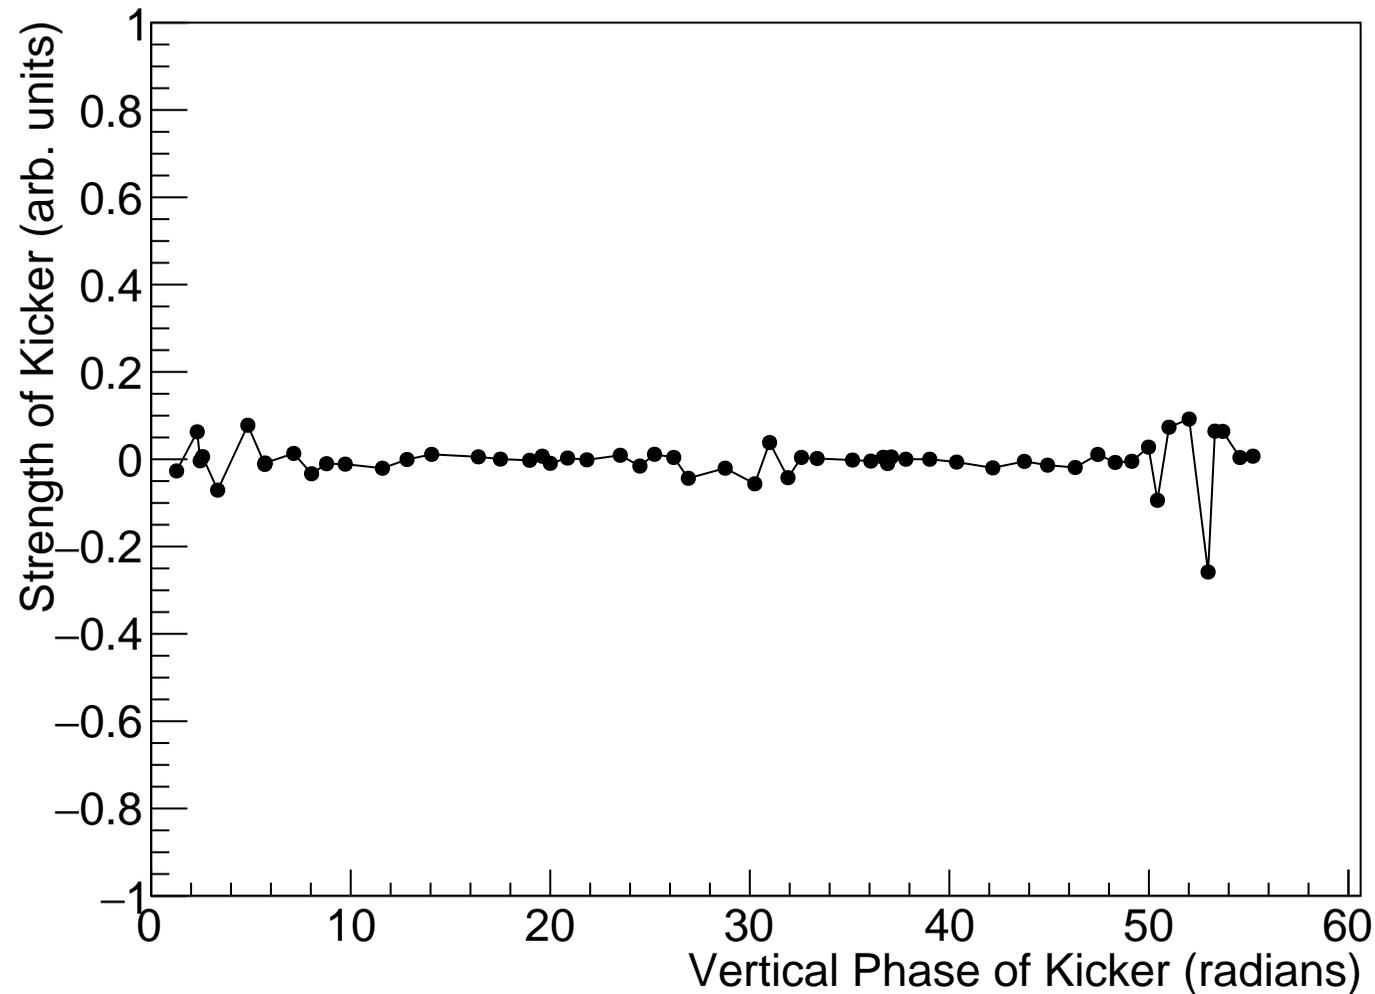

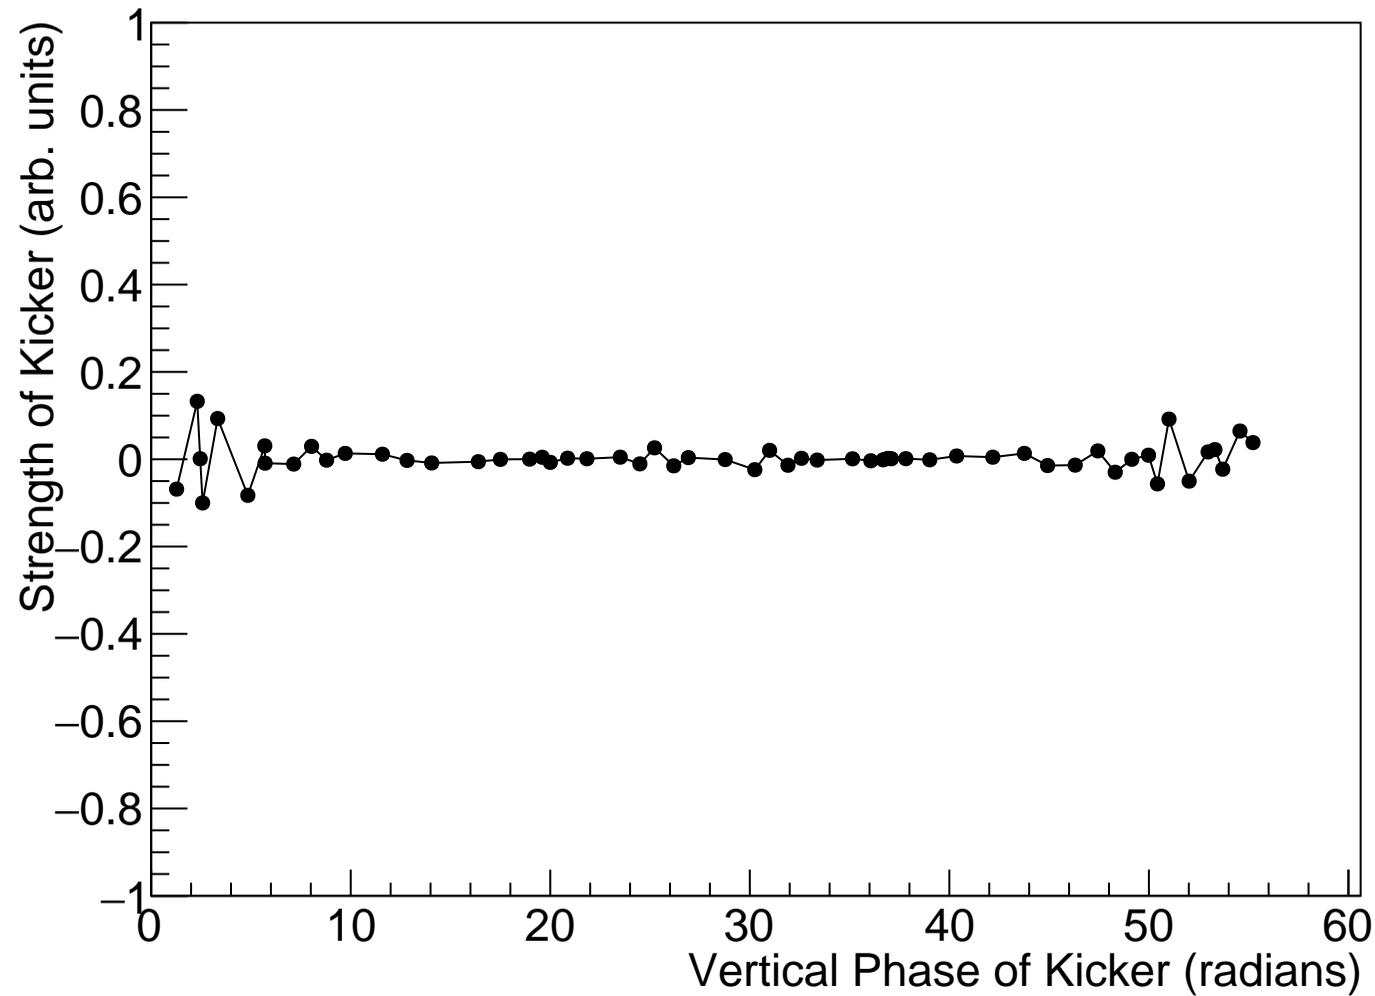

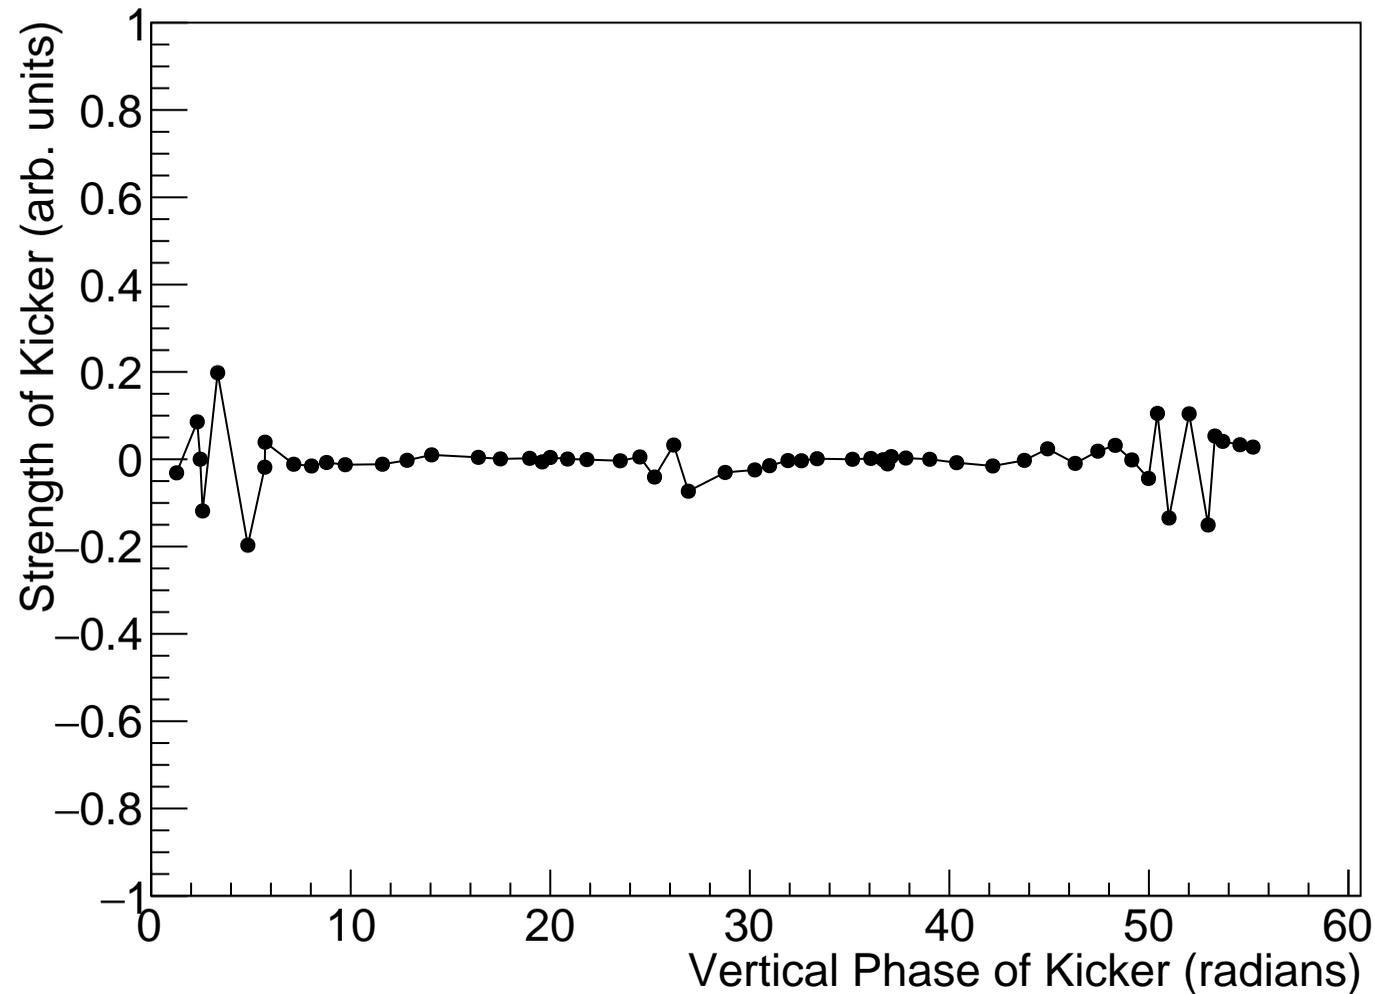

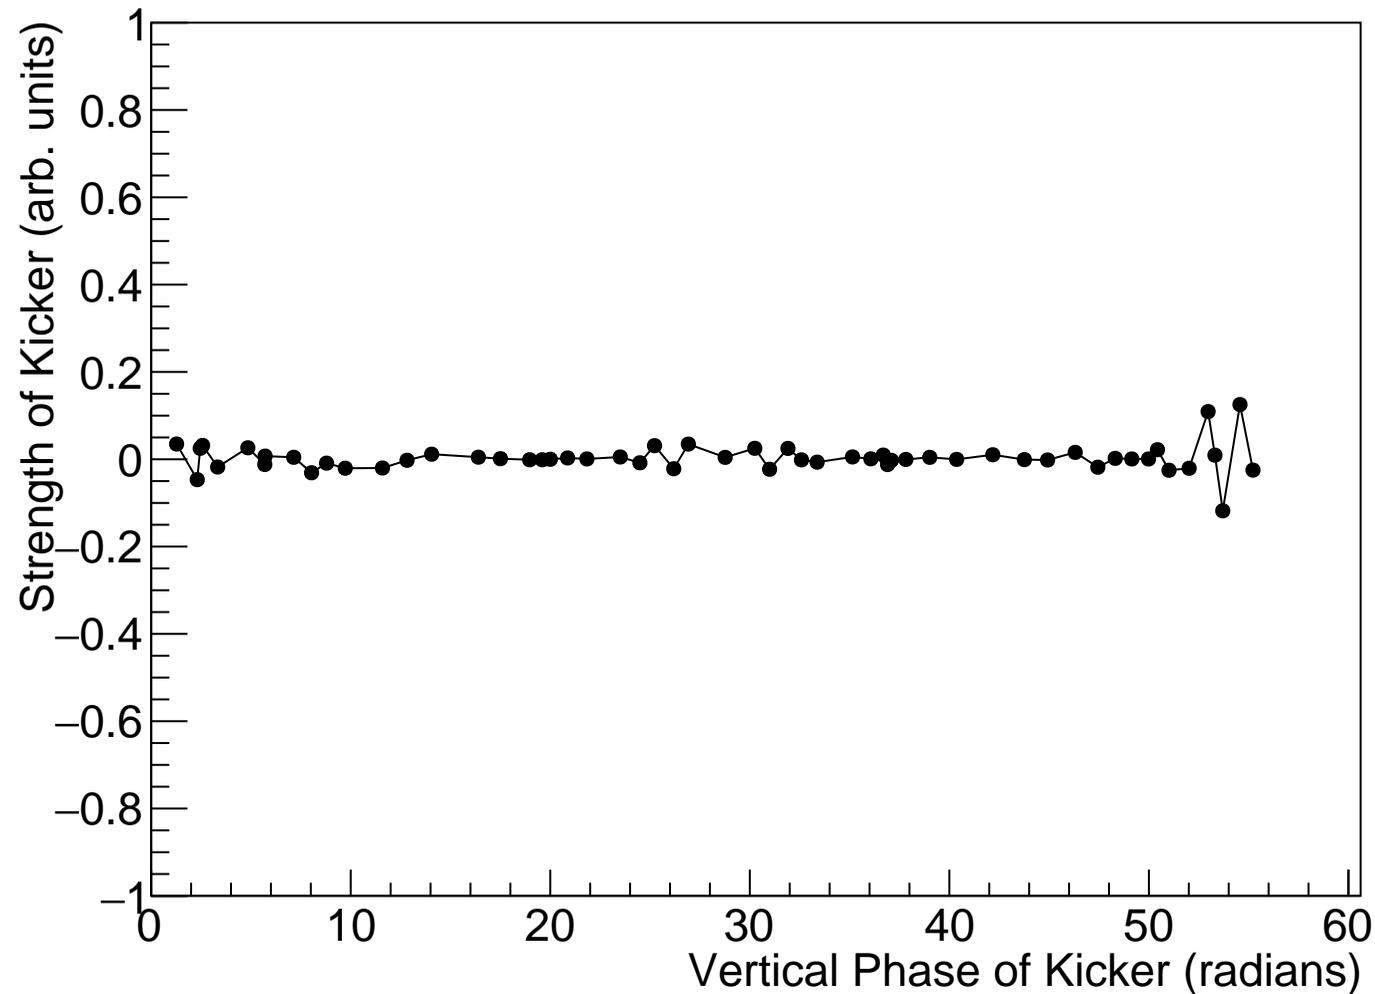

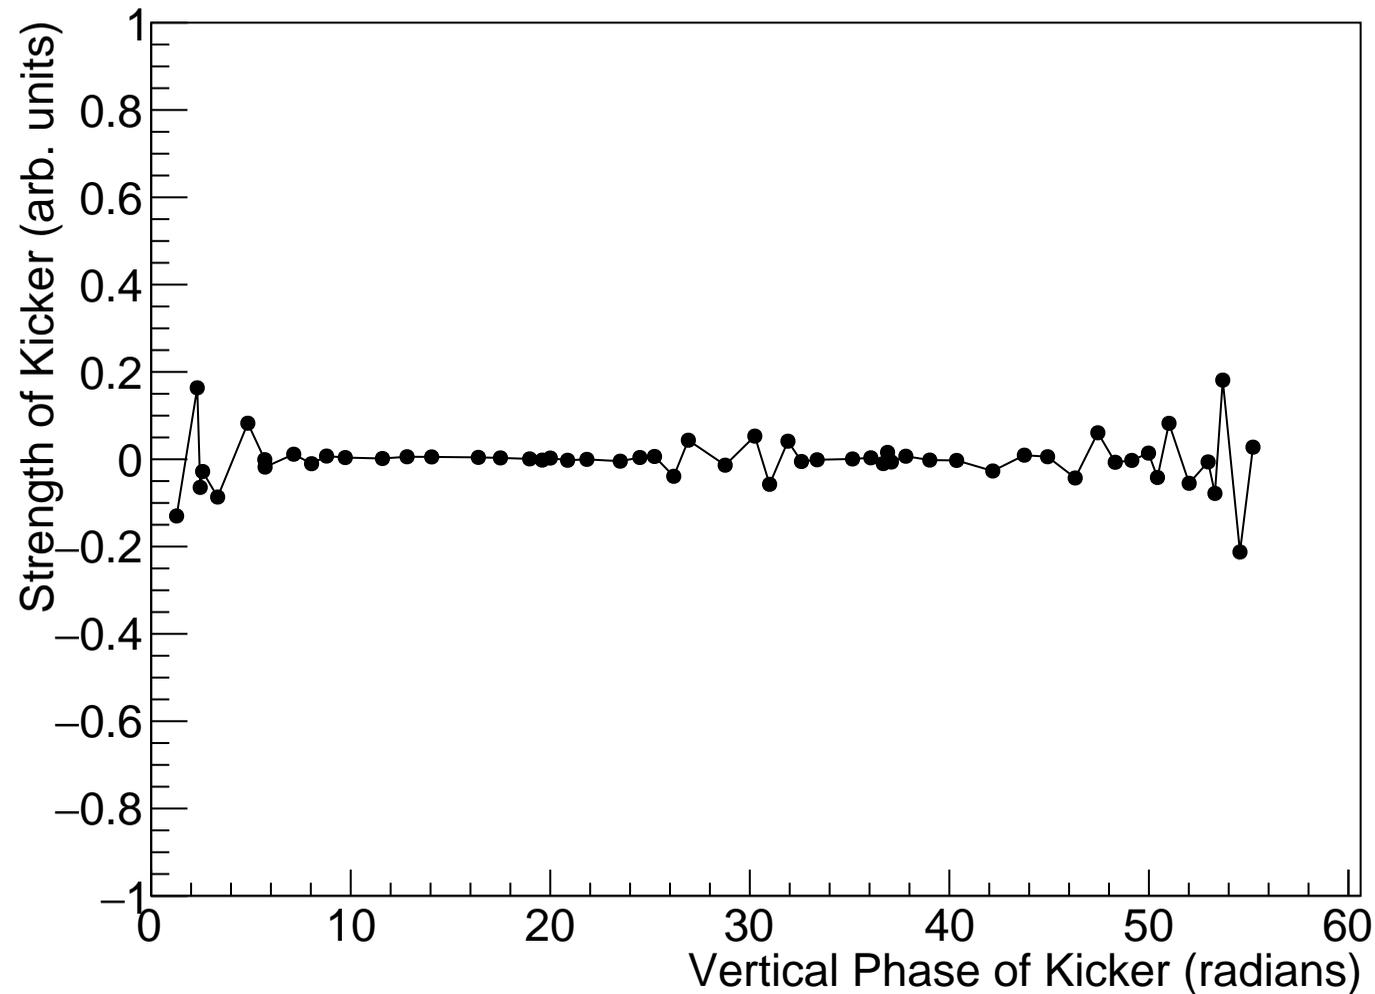

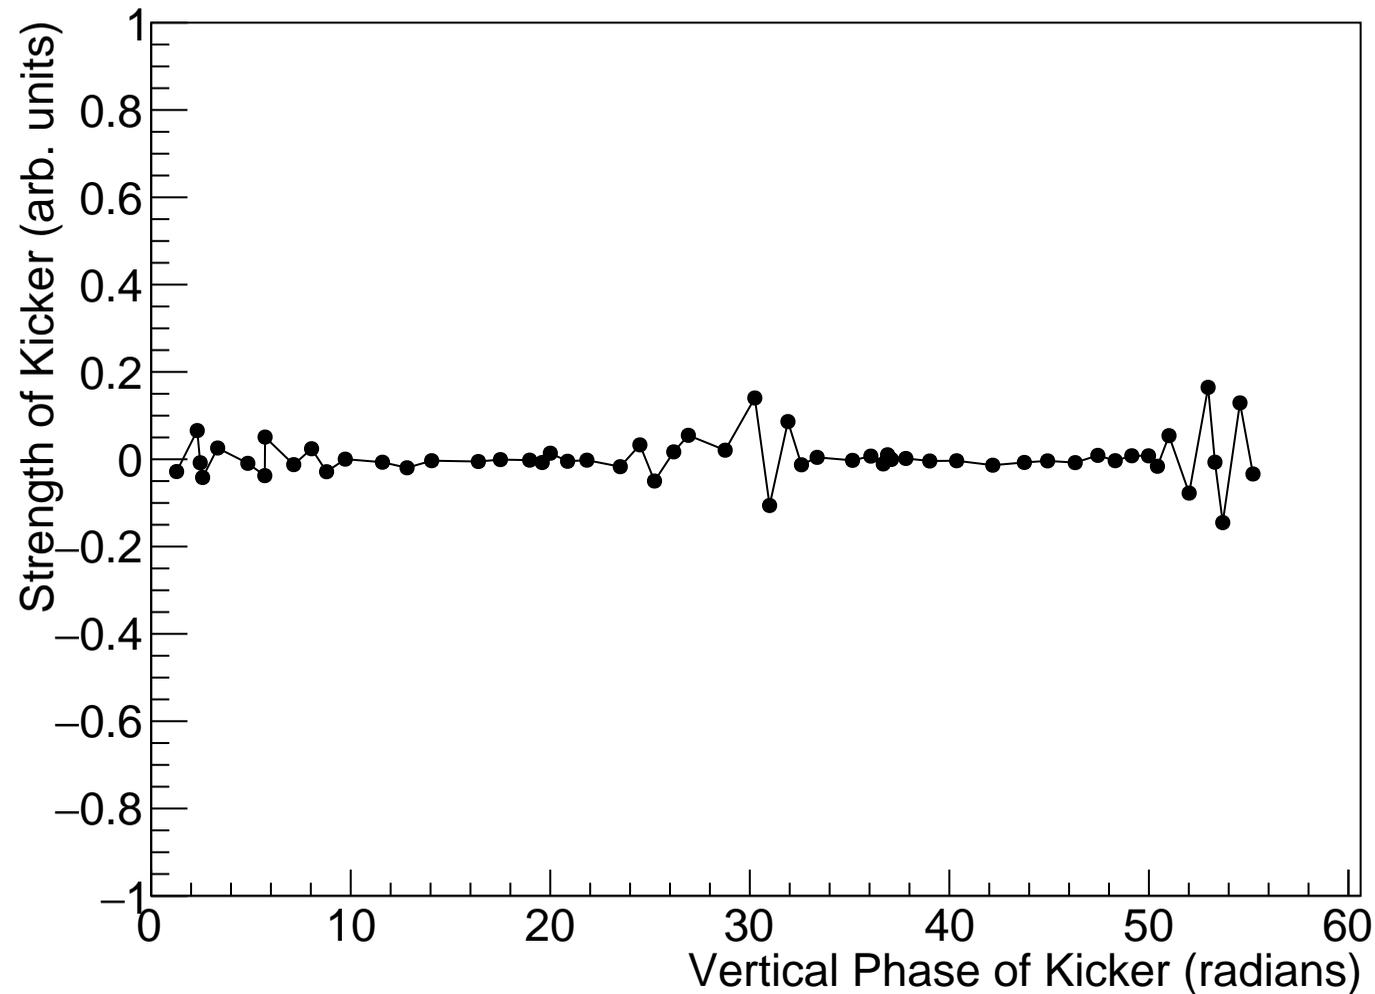

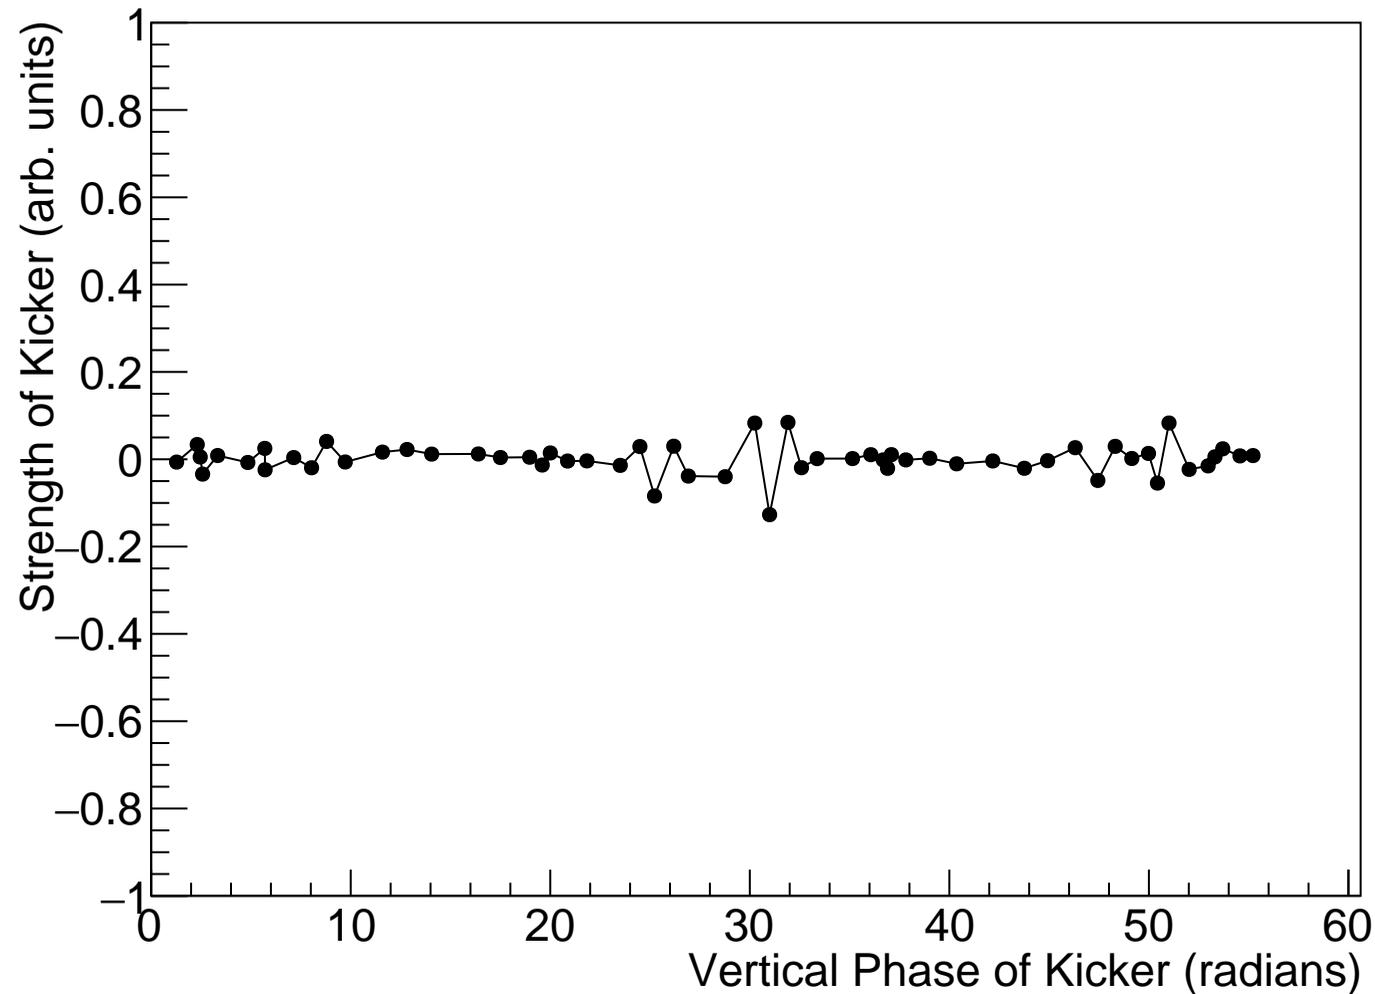

Supplement: Supplementary file 1 [file eigenvector_plots_kick.pdf]
